# Supplementary material for: Conics on smooth quartic surfaces
Source: arXiv:2407.00493 ancillary file (2026-02-11)
Supplement: Supplementary file 1 [file 4tab.pdf]

# CONICS ON SMOOTH QUARTICS: THE COMPUTATION

ALEX DEGTYAREV

This text is a companion to [Alex Degtyarev, \*Conics on smooth quartic surfaces\*](#): we outline the technical details of the computation and present more complete results thereof. References to the main text are prefixed with \*\*. We mostly keep the notation and terminology of \*\*.

The principal goal of these notes is outlining a few tricks and recording the parameters used so that the computation can be reproduced.

## 1. ALGORITHMS

1.1. **The notation.** Essentially, we discuss various ways of computing the sets  $\mathcal{B}_n(\mathcal{S})$  introduced in [\\*\\*\(4.4\)](#). However, for our practical purposes, we modify and refine this purely theoretical notion.

We stick to [\\*\\*Definition 3.2](#) and [\\*\\*Definition 3.3](#) of, respectively, *admissible* and *geometric* sets. An admissible set  $\mathfrak{C}$  is called *exceptional* if  $|\mathfrak{C}| \geq 720$ . Exceptional, as well as some other (see [§1.2](#) below) sets  $\mathfrak{C}$  are detected in the course of computation, their oversets  $\mathfrak{C}' \supset \mathfrak{C}$  are analyzed by other means, upon which  $\mathfrak{C}$  is excluded from the further consideration. Thus, the assertion

$$\mathcal{B}_m^*(\mathcal{S}) = \emptyset$$

(where the superscript is explained in [§1.2](#) below) means that  $|\mathfrak{C}| < m$  for any admissible/geometric subset  $\mathfrak{C} \subset \mathcal{S}$  *with the exception of a number of sets that have already been analyzed*. (Here and below, the choice between admissible and geometric depends on the problem at hand: we always insist that  $\text{rk } \mathfrak{C} \leq 20$ , see [\\*\\*\(3.4\)](#), but we often ignore the other conditions in [\\*\\*Definition 3.3](#).)

Needless to say that it is this “further analysis” that gives rise to the exceptional sets mentioned in [\\*\\*Theorem 5.1](#) and [\\*\\*Theorem 6.1](#) and, eventually, to the four quartics in [\\*\\*Theorem 1.1](#).

Therefore, in addition to the additive bounds  $b(\mathcal{S})$  in [\\*\\*§3.2](#), we use the *reduced bounds*  $\bar{b}(\mathcal{S})$ :

$$\bar{b}(\mathcal{S}) < m \quad \text{if and only if} \quad \mathcal{B}_m^*(\mathcal{S}) = \emptyset.$$

Often, the direct computation of  $\mathcal{B}_m^*(\mathcal{S})$  is not feasible and we break it into several steps. Thus, for an admissible set  $\mathfrak{C}$  and a set  $\mathcal{S} \subset \mathfrak{D}$ , we let  $\mathcal{S}' := \mathcal{S} \cup \sup \mathfrak{C}$  and (cf. also [Convention 1.5](#))

$$(1.1) \quad \mathcal{B}_m^*(\mathfrak{C}; \mathcal{S}) := \{\text{admissible/geometric sets } \mathfrak{C} \subset \mathfrak{C}' \subset \mathcal{S}' \mid |\mathfrak{C}'| \geq m\} / \sim.$$

(Here and below, the quotient is modulo the suitable stabilizer.) In terms of [\(1.1\)](#) we can define a number of other constructions, which mainly reflect the way of the computation rather than the final result. Thus, given pairwise disjoint sets  $\mathcal{S}_1, \mathcal{S}_2, \dots \subset \mathfrak{D}$  and integers  $0 \leq m_1 \leq m_2 \leq \dots$ , we define recursively

$$(1.2) \quad \mathcal{B}_{m_1, m_2, \dots}^*(\mathcal{S}_1; \mathcal{S}_2; \dots) := \bigcup \mathcal{B}_{m_2, \dots}^*(\mathfrak{C}; \mathcal{S}_2, \dots) / \sim, \quad \mathfrak{C} \in \mathcal{B}_{m_1}^*(\mathcal{S}_1), \text{ and}$$

$$(1.3) \quad \mathcal{B}_m^*(\mathcal{S}_1, \mathcal{S}_2, \dots) := \bigcup \mathcal{B}_m^*(\mathfrak{C}; \mathcal{S}_2, \dots) / \sim, \quad \mathfrak{C} \in \mathcal{B}_0^*(\mathcal{S}_1).$$

As a variation of [\(1.3\)](#), for a *homogeneous chain*  $\mathcal{S}_1 \subset \mathcal{S}_2 \subset \dots \subset \mathcal{S}_n$  (see [\\*\\*§4.1](#)), we have

$$(1.4) \quad \mathcal{B}_m^*(\mathcal{S}_1 < \mathcal{S}_2 < \dots) := \mathcal{B}_m^*(\mathcal{S}_1, \mathcal{S}_2 \setminus \mathcal{S}_1, \dots).$$

---

*Key words and phrases.* K3-surface, quartic surface, conic, Niemeier lattice, Leech lattice.

The author was partially supported by the T  B  TAK grant 123F111.

Note, though, that in this latter case, instead of starting from scratch  $\mathcal{B}_0^*$  in (1.3), by **\*\*Lemma 4.3** we can start from  $\mathcal{B}_{m_{i-1}}^*(\mathcal{S}_{i-1})$  when computing the next set  $\mathcal{B}_{m_i}^*(\mathcal{S}_i)$ , where

$$m_n := m, \quad m_{i-1} := \kappa_i \left\lceil m_i \frac{|\mathcal{S}_{i-1}|}{\kappa_i |\mathcal{S}_i|} \right\rceil \quad \text{for } i = n \text{ down to } 2; \quad \kappa_i \in \{1, 2\};$$

here,  $\kappa_i = 2$  iff  $\mathcal{S}_{i-1}$  is self-dual: then, so is any  $\mathcal{S}_{i-1}$ -saturated subset  $\mathfrak{C} \subset \mathcal{S}_{i-1}$  and  $|\mathfrak{C}|$  is even.

Thanks to the punctuation, we can combine these constructs and describe a long computation and its result by means of a single equation like

$$\mathcal{B}_{m,n}^*(\mathcal{P}, \mathcal{Q} < \mathcal{R}; \mathcal{S}_1, \mathcal{S}_2) = \emptyset.$$

The deciphering is left to the reader.

**Convention 1.5.** Clearly, most algorithms boil down to the following problem, *cf.* (1.1):

$$\text{compute } \mathcal{B}_n^*(\mathfrak{C}; \mathcal{S} \setminus \mathcal{Q}) \text{ for each set } \mathfrak{C} \in \mathcal{B}_m^*(\mathcal{Q})$$

or iterations thereof. To reduce the overcounting, we assume that the fixed set  $\mathfrak{C}$  no longer changes. That is, we consider only

$$\text{extensions } \mathfrak{C} \subset \mathfrak{C}' \subset \mathcal{S} \text{ such that } \text{sat}_{\mathcal{Q}} \mathfrak{C}' = \mathfrak{C};$$

otherwise  $\mathfrak{C}'$  would appear as an extension of the other set  $\text{sat}_{\mathcal{Q}} \mathfrak{C}' \in \mathcal{B}_m^*(\mathcal{Q})$ .

With the exception of §1.4 below, we assume all sets  $\mathcal{S}_i$  self dual; hence, so are saturated subsets  $\mathfrak{C} \subset \bigcup \mathcal{S}_i$ . Furthermore, often  $\mathcal{S}_i$  are unions of orbits. We introduce the shortcut

$$\bar{\mathfrak{o}}_n^+ := \bar{\mathfrak{o}}_n \text{ if } \bar{\mathfrak{o}}_n^* = \bar{\mathfrak{o}}_n \quad \text{or} \quad \bar{\mathfrak{o}}_n^+ := \bar{\mathfrak{o}}_n \cup \bar{\mathfrak{o}}_n^* \text{ otherwise.}$$

Only one of each pair of dual orbits is used in the computation, but the goals  $m, \dots$  in  $\mathcal{B}_{m,\dots}^*$  take both into account. Due to the duality, all cardinalities are even. Hence, the sets (1.3) are merely a means of estimating the reduced bounds as follows:

$$(1.6) \quad \mathcal{B}_m^*(\mathcal{S}_1, \dots) = \emptyset \quad \text{implies that} \quad \bar{b}(\mathcal{S}_1 \cup \dots) \leq m - 2.$$

On the other hand, the sets (1.2) may be much easier to compute if  $m_1$  is large enough. Typically, these sets are used in the form of the following obvious statement:

$$(1.7) \quad \text{if } \mathcal{B}_{m,m+n-2}^*(\mathcal{S}; \mathcal{T}) = \mathcal{B}_{n,m+n-2}^*(\mathcal{T}; \mathcal{S}) = \emptyset, \quad \text{then} \quad \bar{b}(\mathcal{S}, \mathcal{T}) \leq m + n - 4.$$

More sophisticated implications are explained on a case-by-case basis, *cf.* the end of §4.4.3.

**1.2. Computation up to rank  $r$ .** One has  $\text{rk } \mathfrak{C} \leq 20$  for any geometric set  $\mathfrak{C} \subset \mathfrak{D}_h$ , see **\*\* (3.4)**, and this inequality plays a crucial rôle in our computation. For a subset  $\mathcal{S} \subset \mathfrak{D}_h$ , define

$$\mathcal{B}_m^r(\mathcal{S}) := \{\mathfrak{C} \in \mathcal{B}_m(\mathcal{S}) \mid \text{rk } \mathfrak{C} \leq 20 - r\}$$

and similar counterparts for the other sets (1.2)–(1.4). We use roman numerals for  $r$ , thus speaking about  $\mathcal{B}^0 = \mathcal{B}, \mathcal{B}', \mathcal{B}'', \mathcal{B}''', \mathcal{B}^{\text{iv}}$ . The reason is that, on the one hand,

- often  $\mathcal{B}_m(\mathcal{S}) \neq \emptyset$ , preventing us from making conclusion (1.6), (1.7); on the other hand,
- if  $\text{rk } \mathfrak{C}$  is large, it is relatively easy to list all saturated admissible oversets  $\mathfrak{C} \subset \mathfrak{C}' \subset \mathfrak{D}$  of  $\text{rank } \text{rk } \mathfrak{C} < \text{rk } \mathfrak{C}' \leq 20$  (*cf.* §1.3) and select the exceptional ones; others can be ignored.

More precisely, we can easily *push* the rank by up to units by listing all  $(\text{stab } \mathfrak{C})$ -orbits of lines or planes in  $N/\text{span } \mathfrak{C}$  generated by conics (*cf.* §1.3 below) and considering them one-by-one. We can also apply, at least partially, **Convention 1.5** and inhibit the appearance of new conics from a certain subset  $\mathcal{Q} \subset \mathcal{S}$  for which the intersection  $\mathfrak{C}' \cap \mathcal{Q} = \mathfrak{C} \cap \mathcal{Q}$  has already been fixed.

To save memory, in all algorithms we periodically apply this trick and discard all sets of rank  $\text{rk } \mathfrak{C} \geq 18$ , even before checking whether they would survive the subsequent steps; in other words, by default we always compute at most  $\mathcal{B}''$ . If, upon the computation, we find that  $\mathcal{B}''$  consists of reasonably few sets  $\mathfrak{C}$  of rank  $\text{rk } \mathfrak{C} = 16, 17$ , we push the rank in two increments, first up to 18, and

then up to 20. This works reasonably well for rank  $\text{rk } \mathfrak{C} = 17$ , but it is quite time consuming for  $\text{rk } \mathfrak{C} = 16$ ; we leave it as the last resort, only if very few such sets need to be ruled out.

In other words, in all equations below  $\mathcal{B}''$  is the default whereas the appearance of  $\mathcal{B}'''$  or  $\mathcal{B}^{\text{iv}}$  indicates the fact that  $\mathcal{B}'' \neq \emptyset$  but the few sets found have been analysed and discarded.

**1.3. Linear algebra vs. arithmetic.** In this paper, we consider *primitive* sublattices of  $N$  only; hence, when establishing the admissibility of a set  $\mathfrak{C} \subset \mathfrak{D}$  or computing its saturation, we can work over  $\mathbb{Q}$  rather than  $\mathbb{Z}$ . (See also the refined combinatorial bounds in [\\*\\*§3.5](#).) In fact, given a set  $\mathfrak{C} \subset \mathfrak{D}$ , we compute and store the matrix of the projection

$$p: N \rightarrow (N/\text{span } \mathfrak{C}) \otimes \mathbb{Q},$$

which can be applied (on demand) to the roots  $r \in N$  or other conics  $l \in \mathfrak{D}$ . The non-zero results are normalized and also stored; we denote the normalization by  $\bar{p}(l)$ .

This approach is faster than working with integral matrices and it reduces the number of essentially distinct sets  $\mathfrak{C} \subset \mathfrak{D}$  to be considered, *viz.*, (relatively) saturated sets only.

It also makes it easy to push the rank (*cf.* [§1.2](#) and [§1.6](#)) by up to two units. Indeed, assume that we are computing a certain set  $\mathcal{B}_n^*(\mathcal{S})$ , typically in the presence of a certain “fixed” subset  $\mathcal{Q} \subset \mathcal{S}$ , *cf.* [Convention 1.5](#). Then, the corank 1 extensions of an intermediate subset  $\mathfrak{C} \subset \mathcal{S}$  are essentially found together with  $\text{sat}_{\mathcal{S}} \mathfrak{C}$ : they are the elements of the set

$$\bar{P}_{\mathfrak{C}} := \{\bar{p}(l) \neq 0 \mid l \in \mathcal{S}\}$$

of normalized projections that are *not* of the form

$$\bar{p}(r) \text{ for a root } r \in N \quad \text{or} \quad \bar{p}(l) \text{ for } l \in \mathcal{Q}$$

(or otherwise prohibited, *cf.* [\(1.13\)](#) below). The sizes of these extensions are seen immediately from the data already stored and small sets can be discarded even before any further analysis.

The corank 2 extensions are slightly more involved but still doable: we need to consider pairs of valid projections  $p_1, p_2 \in \bar{P}_{\mathfrak{C}}$  and analyze the possible linear dependencies.

It is worth mentioning that each step of the brute force algorithm [§1.4](#) is essentially pushing the rank by one unit; thus, *de facto* it is performed at the end of the previous step, when computing the saturation.

**Remark 1.8.** Technically, the extra data such as the projection  $p$  or the set  $\bar{P}_{\mathfrak{C}}$  (computed on demand conic by conic) are stored in a separate record linked to  $\mathfrak{C}$  and can be reused. For example,  $\mathcal{B}_m(\mathcal{Q})$  is a list of  $\mathcal{Q}$ -saturated sets which are to be used as seeds in the computation of  $\mathcal{B}_n(\mathcal{S})$  for an overset (often more than one)  $\mathcal{S} \supset \mathcal{Q}$ . More precisely, the seeds are the saturations  $\text{sat}_{\mathcal{S}} \mathfrak{C}$ ,  $\mathfrak{C} \in \mathcal{B}_m(\mathcal{Q})$ . We use the data stored to compute  $\text{sat}_{\mathcal{S}} \mathfrak{C}$  and link to it *the same* data record.

**1.4. Brute force.** Whenever necessary, we compute the sets  $\mathcal{B}_m(\mathfrak{o})$  and estimate the bounds  $b(\mathfrak{o})$  for individual combinatorial orbits. For each orbit  $\bar{\mathfrak{o}}_n$ , at most one combinatorial orbit  $\mathfrak{o} \subset \bar{\mathfrak{o}}_n$  is considered, *viz.* the one presented in the tables; if necessary, *e.g.*, in [§1.5](#) below, the set  $\mathcal{B}_m(\mathfrak{o})$  is translated to other combinatorial orbits  $\mathfrak{o}' \subset \bar{\mathfrak{o}}$  *via* the group  $O_h(N)$ .

This computation is explained, in the form of a sequence of records

$n := \text{rec}(\dots)$ ,

at the beginning of the subsection dedicated to the particular polarization  $h \in N$ ; if an index  $n$  is not mentioned, the orbit  $\bar{\mathfrak{o}}_n$  is not considered. An empty record

$n := \text{rec}()$ ,

means computing from scratch the whole set  $\mathcal{B}_0(\mathfrak{o})$ . Otherwise, the algorithm is adjusted by the following parameters:

**fixed** :=  $\pm k$  (other parameters make no sense unless this one is set),

**min** :=  $m$  (ignored unless **fixed** is set),

**chain** :=  $c$  (ignored unless **fixed** and **min** are set),

whose meaning is explained below.

If `fixed := k` is set, we fix a vector  $a \in \mathfrak{o}_{|k|}$  and compute the set  $\mathcal{B}_m(\mathfrak{o}_k^- < \mathfrak{o})$  (in the notation of §1.1), where

$$\mathfrak{o}_k^- := \begin{cases} \{l \in \mathfrak{o} \mid l|_k = a\} & \text{if } k > 0, \\ \{l \in \mathfrak{o} \mid l|_{-k} = a \text{ or } l|_{-k} = h|_{-k} - a\} & \text{if } k < 0. \end{cases}$$

For this, we also need `min := m`. If  $m$  is not set, we merely compute  $\mathcal{B}_0(\mathfrak{o}_k^-)$  and invoke **Lemma 4.3** to draw a conclusion about  $b(\mathfrak{o})$ , see item  $\dagger$  in **Convention 2.3**.

If `chain := c` is also set, we insert one (if  $c$  is a positive integer) or more (if  $c = [c_1, \dots, c_n]$  is a list) extra sets

$$\mathfrak{o}_k^- =: \mathfrak{c}_0 \subset \mathfrak{c}_1 \subset \dots \subset \mathfrak{c}_n \subset \mathfrak{c}_{n+1} := \mathfrak{o},$$

where, for each  $i = 1, \dots, n$ , the set  $\mathfrak{c}_i$  is a union of  $c_i$  elements of the  $(\text{stab } \mathfrak{c}_{n+1})$ -orbit of  $\mathfrak{c}_{i-1}$  such that both  $\mathfrak{c}_{i-1} \subset \mathfrak{c}_i$  and  $\mathfrak{c}_i \subset \mathfrak{c}_{n+1}$  are homogeneous (see **§4.1**). These sets are computed automatically and, if more than one is found, one is chosen randomly, with a preference to those of smaller rank. (If none were found, **Error()**; would be raised.)

In §4–§6, after finding the bound  $b(\mathfrak{o})$ , we may also need the actual set  $\mathcal{B}_m(\mathfrak{o})$  to be used in the puzzle assembly algorithm (see §1.5 below), and that may require a lower goal `min := m` (cf. **Remark 1.10** below). These lower goals are shown as **GAP** comments:

`# min := m.`

The computation itself is straightforward brute force. When computing a set  $\mathcal{B}_m(\mathcal{S})$ , with  $\mathcal{S} = \mathfrak{o}$ ,  $\mathfrak{o}_k^-$ , or  $\mathfrak{c}_i$ , we consider  $\mathcal{S}$ -saturated subsets  $\mathfrak{C} \subset \mathcal{S}$  and increase the rank step-by-step, by one unit at a time, as explained in §1.3. All new sets are sorted to avoid repetitions, *i.e.*, a single representative of each  $(\text{stab } \mathcal{S})$ -orbit present is retained. We start with checking that  $\mathcal{S}$  itself is not admissible (as it never is) and, hence,

$$(1.9) \quad \text{rk } \mathfrak{C} \leq r_{\max} := \min\{20, \text{rk } \mathcal{S} - 1\}$$

for each geometric set  $\mathfrak{C} \subset \mathcal{S}$ . For subsets  $\mathfrak{C}$  of rank  $\text{rk } \mathfrak{C} \geq r_{\max} - 2$ , we push the rank by up to two units at once, also as explained in §1.3, and, before sorting, retain only those oversets  $\mathfrak{C}' \supset \mathfrak{C}$  that satisfy the goal  $|\mathfrak{C}'| \geq m$ .

**1.5. Puzzle assembly.** Let  $\mathcal{S}$  be a union of several combinatorial orbits, all within the same orbit  $\bar{\mathfrak{o}}$ . Then, instead of the brute force §1.4, the sets  $\mathcal{B}_m^*(\mathcal{S})$ ,  $\mathcal{B}_m^*(\mathfrak{C}; \mathcal{S})$ , *etc.* are computed by the *puzzle assembly*: intuitively, we try to put together as many and as large “pieces” as possible in order to fit a large number of conics into a limited rank.

The rôle of the “pieces” of the puzzle is played by the elements of  $\mathcal{B}_0(\mathfrak{o})$ ,  $\mathfrak{o} \subset \bar{\mathfrak{o}}$ . Clearly, it suffices to compute this set for one of the combinatorial orbits only (we use the one shown in the tables); the others are of the form  $\mathcal{B}_0(\mathfrak{o}) \cdot g$ ,  $g \in O_h(N)$ .

**Remark 1.10.** The computation of the full set  $\mathcal{B}_0(\mathfrak{o})$  may be expensive, and often it suffices to know a smaller set  $\mathcal{B}_n(\mathfrak{o})$ . Starting from a heuristic estimate, the precise value of  $n$  (indicated below *via* the **GAP** comments `# min := n`, cf. §1.4) is determined experimentally: at each step, the algorithm computes the minimal size of the pieces required to continue (see item (1) in the algorithm below) and, if a certain size is not available, an **Error()**; is raised.

Let  $G$  be the relevant stabilizer, *i.e.*,  $G := \text{stab } \mathcal{S}$ , or  $G := \text{stab}(\mathcal{S}, \text{stab } \mathfrak{C})$ , *etc.*

We start with the given set  $\mathfrak{C}$  (possibly  $\mathfrak{C} = \emptyset$ ) and extend it by a sequence

$$(1.11) \quad \mathfrak{C} =: \mathfrak{C}_0 \subset \mathfrak{C}_1 \subset \dots \subset \mathfrak{C}_n, \quad \mathfrak{C}_k := \mathfrak{C}_k \setminus \mathfrak{C}_{k-1} \subset \mathfrak{o}_k \text{ for } k \geq 1,$$

where  $(\mathfrak{o}_1^+, \dots, \mathfrak{o}_n^+)$  is a rearrangement of the (pairs of dual) combinatorial orbits constituting  $\mathcal{S}$ . (*De facto*, usually this process aborts prematurely *via* §1.6 below.) In order to keep the intermediate sets  $\mathfrak{C}_k$  as large as possible and reduce the overcounting, we always assume that

$$(1.12) \quad |\mathfrak{C}_1| \geq |\mathfrak{C}_2| \geq \dots \geq |\mathfrak{C}_n|,$$

and that is why the combinatorial orbits  $\mathfrak{o}_i \subset \mathcal{S}$  may have to be rearranged, see item (3) below.

Let  $\bar{\mathfrak{C}}_k := \text{sat}_{\mathcal{S}} \mathfrak{C}_k$ . In addition to [Convention 1.5](#) concerning the initial set  $\mathfrak{C}$ , if any, we also keep track of the combinatorial orbits already used and assume the intersections fixed, *i.e.*, at each step  $k$  we check that

$$(1.13) \quad |\bar{\mathfrak{C}}_k \cap \mathfrak{o}_i| = |\mathfrak{S}_i| \text{ for } i \leq k, \quad |\bar{\mathfrak{C}}_k \cap \mathfrak{o}_i| \leq |\mathfrak{S}_i| \text{ for } i > k, \text{ see (1.12).}$$

Thus, let  $\kappa := 2$  (if the combinatorial orbits in  $\bar{\mathfrak{o}}$  are self-dual) or  $\kappa := 1$  (otherwise), and let  $2n/\kappa$  be the number of combinatorial orbits constituting  $\mathcal{S}$ . Then step  $k$  of the algorithm proceeds as follows. (At this step, a set  $\mathfrak{C}_{k-1}$  and, hence, the sequence  $(\mathfrak{o}_1, \dots, \mathfrak{o}_{k-1})$  are fixed whereas the notation  $\mathfrak{o}_i$ ,  $i \geq k$  merely refers to all remaining combinatorial orbits.)

(1) Compute the size bounds

$$(1.14) \quad s_{\max} := |\mathfrak{S}_{k-1}| \text{ (if } k > 1), \quad s_{\min} := \kappa \left\lceil \frac{m - |\mathfrak{C}| - \kappa \sum_{i < k} |\mathfrak{S}_i|}{2(n - k - 1)} \right\rceil, \text{ see (1.12).}$$

It is at this point that we check the completeness of  $\mathcal{B}_n(\mathfrak{o})$ , see [Remark 1.10](#).

- (2) If there are combinatorial orbits  $\mathfrak{o}_i$ ,  $i \geq k$ , with  $|\bar{\mathfrak{C}}_{k-1} \cap \mathfrak{o}_i| > s_{\max}$ , abort; if there are those with  $|\bar{\mathfrak{C}}_{k-1} \cap \mathfrak{o}_i| = s_{\max}$ , add *all of them* to the list [\(1.11\)](#) and proceed to the corresponding subsequent step, retaining all auxiliary data computed in [§1.3](#), *cf.* [Remark 1.8](#).
- (3) Let  $G_k := \text{stab}(\bar{\mathfrak{C}}_{k-1}, G)$  and take for  $\mathfrak{o}_k$  a single representative  $\mathfrak{o}_k \subset \mathfrak{o}_k^+$  of each  $G_k$ -orbit on the set  $\{\mathfrak{o}_k^+, \dots, \mathfrak{o}_n^+\}$ . Proceed separately for each  $\mathfrak{o}_k$  chosen.
- (4) Consider all sets (not just orbits!)  $\mathfrak{S} \in \mathcal{B}_0(\mathfrak{o}_k)$  satisfying

$$s_{\min} \leq |\mathfrak{S}| < s_{\max}, \quad \mathfrak{S} \supset \bar{\mathfrak{C}}_{k-1} \cap \mathfrak{o}_k;$$

pick for  $\mathfrak{S}_k$  a single representative of each  $\text{stab}(\mathfrak{o}_k, G_k)$ -orbit of such sets  $\mathfrak{S}$ .

- (5) Let  $\mathfrak{C}_k := \mathfrak{C}_{k-1} \cup \mathfrak{S}_k$ , check the admissibility, compute  $\bar{\mathfrak{C}}_k$ , verify [\(1.13\)](#), [Convention 1.5](#), [\(1.19\)](#) below, *etc.* Optionally, we can also check if  $\mathfrak{C}_k$  is (sub-)geometric.
- (6) If  $\text{rk } \mathfrak{C}_k \geq r_{\max} - 2$ , analyze it immediately (see [§1.6](#) below) and discard; otherwise, add  $\mathfrak{C}_k$  to the master list *unless* the latter already has a set  $G$ -isomorphic to  $\mathfrak{S}_k$ .

A further analysis is performed upon the completion of each partial *pattern*  $|\mathfrak{S}_1| \geq \dots \geq |\mathfrak{S}_k|$ :

- analyze all sets  $\mathfrak{S}_k$  of rank  $\text{rk } \mathfrak{S}_k \geq r_{\max} - 2$  – **push**, see [§1.6](#) below;
- if sufficiently many (by default, at least 128) sets of rank  $\text{rk } \mathfrak{C}_k \geq 18$  have been collected, analyze and discard these sets as explained in [§1.2](#).

**Remark 1.15.** Here and in [§1.4](#), each steps concludes in *sorting*, *i.e.*, retaining, for the subsequent steps, a single representative of each orbit of the relevant symmetry group. When comparing two sets  $\mathfrak{C}'$ ,  $\mathfrak{C}''$ , we compare some “obvious” invariants first, such as ranks, sizes, sorted lists of the valencies of the vertices, *etc.*, upon which we invoke **RepresentativeAction**, which may be slow. Probably, better performance could be achieved by using the canonical labelling from the **digraph** package, *cf.* [\(7.4\)](#) below, but this has not been implemented yet.

**1.6. Rank pushing.** When computing  $\mathcal{B}_m^*(\mathcal{S})$ , we always keep in mind the maximal rank [\(1.9\)](#). By default, we seamlessly *push the rank* by up to two units: when a subset  $\mathfrak{C} \subset \mathcal{S}$  of rank

$$\text{rk } \mathfrak{C} \geq r_{\max} - 2$$

is discovered, we immediately analyze its corank 1 or 2 extensions  $\mathfrak{C} \subset \mathfrak{C}' \subset \mathcal{S}$  (see [§1.3](#)) and exclude  $\mathfrak{C}$  and the extensions found from the consideration, storing those of size  $|\mathfrak{C}'| \geq m$  in the output.

Occasionally, we set the **push** parameter of the **data** object (see [§4.1](#) below) to 1 or 2. In this case, after each “mini-step” of the algorithm, upon the preliminary sorting, the rank is pushed by up to, respectively, 3 or 4 units; this is done in two increments, similar to [§1.2](#).

In some cases, *cf.* [§5.1](#) below, in order to avoid the computation of the full set  $\mathcal{B}_0(\mathfrak{o})$ , we set **push** := 3 (or even 4), pushing the rank by up to 6 units: for each set  $\mathfrak{C}$  of rank  $\text{rk } \mathfrak{C} = r_{\max} - 3$  (or  $r_{\max} - 4$  if **push** = 4) we switch to the brute force algorithm [§1.4](#), extending  $\mathfrak{C}$  by individual conics  $l \in \mathcal{S}$  rather than (translates of) subsets of  $\mathfrak{o}$ . Experimentally, relatively few  $(\text{stab } \mathcal{S})$ -orbits of such sets are encountered but, on the other hand, the computation of  $\mathcal{B}_0(\mathfrak{o})$  is quite expensive.

**Remark 1.16.** When computing  $\mathcal{B}_*(\mathfrak{C}; \mathcal{S})$  for  $\mathfrak{C} \in \mathcal{B}_*(\mathcal{Q})$ , the circumstances may change and  $\mathfrak{C}$  itself may immediately be “eligible” for the rank pushing in  $\mathcal{S}$ . In this case, we skip the puzzle assembly algorithm for  $\mathfrak{C}$ , merely pushing its rank.

1.7. **Clusters.** Often, we have to break an orbit  $\bar{\mathfrak{o}}$  into *clusters*,

$$\bar{\mathfrak{o}} = \bigcup_k \mathfrak{c}_k,$$

where each cluster  $\mathfrak{c}_k$  is a union of several combinatorial orbits so that

- $\{\mathfrak{c}_k\}$  is the  $O_h(N)$ -orbit of (any of)  $\mathfrak{c}_k$ .

Note that the pair  $\mathfrak{c}_k \subset \bar{\mathfrak{o}}$  is automatically homogeneous (see \*\*§4.1).

Clusters are usually defined “geometrically”, in terms of support. To this end, we represent the Niemeier lattice in question as in \*\*§(3.1) (cf. also [Convention 2.2](#) below), with an index set  $\Omega$ , and define the *support* of a vector  $v \in N$  as

$$\text{supp } v := \{k \in \Omega \mid v|_k \neq 0\}.$$

The support  $\text{supp } \mathfrak{o}$  of a combinatorial orbit  $\mathfrak{o}$  is the common support of its conics  $l \in \mathfrak{o}$ .

We use the shortcut  $\bar{\Omega} := \Omega \setminus \text{supp } \bar{h}$ .

**Remark 1.17.** In the tables below, the support  $\text{supp } h$  is the set of columns *other* than  $[0]_0$ ; for the combinatorial orbits  $\mathfrak{o}$  shown,  $\text{supp } \mathfrak{o}$  is the set of columns *other* than  $[0]_0$ .

A “straightforward” application of clusters (typically used if there are but two or three clusters) is a computation of

$$\mathcal{B}_*(\mathfrak{c}_1 < \mathfrak{c}_1 \cup \mathfrak{c}_2 < \mathfrak{c}_1 \cup \mathfrak{c}_2 \cup \mathfrak{c}_3 < \dots),$$

see (1.4), with each step

$$(1.18) \quad \mathcal{B}_*(\mathfrak{C}_{k-1}, \mathfrak{c}_1 \cup \dots \cup \mathfrak{c}_k)$$

done by the puzzle assembly §1.5. In this case, similar to (1.12), for a set  $\mathfrak{C}$  to be constructed we always assume that

$$(1.19) \quad |\mathfrak{C} \cup \mathfrak{c}_1| \geq |\mathfrak{C} \cap \mathfrak{c}_2| \geq |\mathfrak{C} \cup \mathfrak{c}_3| \geq \dots$$

Then, at each step (1.18), we can impose both lower *and upper* bounds similar to (1.14); occasionally, we can further reduce the overcounting by checking an analogue of (1.13).

**Remark 1.20.** The drawback of (1.19) is the fact that, in (1.18), the order of the subsequent clusters  $\mathfrak{c}_k, \mathfrak{c}_{k+1}, \dots$  may depend on  $\mathfrak{C}_{k-1}$ , as they may not be in the same  $(\text{stab } \mathfrak{C}_{k-1})$ -orbit. It is here that we have to use the function `@select` from §4.1, cf., e.g., §4.4.4.

It is not uncommon to consider several nested systems of clusters  $\{\mathfrak{c}_i\}$ ,  $\{\mathfrak{c}'_k\}$ ,  $\{\mathfrak{c}''_m\}$ , etc. so that

- each  $\mathfrak{c}_i$  is a union of some of  $\mathfrak{o} \subset \bar{\mathfrak{o}}$ , each  $\mathfrak{c}'_k$  is a union of some of  $\mathfrak{c}_i$ , etc., and
- the chain  $\mathfrak{c}_i \subset \mathfrak{c}'_k \subset \mathfrak{c}''_m \subset \dots \subset \bar{\mathfrak{o}}$  is homogeneous (see \*\*§4.1).

A typical application is a computation of the form

$$\mathcal{B}_*(\mathfrak{c}_1 < \mathfrak{c}'_k < \mathfrak{c}''_m < \dots),$$

see (1.4) and the explanation/assumptions thereafter, and we use *pipes* as explained in §4.1. As in [Remark 1.20](#), the particular indices  $k, m, \dots$  may depend on the intermediate sets encountered, and we use `@select` from §4.1, cf., e.g.,  $\mathfrak{c}_o \subset \mathfrak{c}'_{o,o'} := \mathfrak{c}_o \cup \mathfrak{c}_{o'}$  in §4.3.3.

**Remark 1.21.** We try to define clusters so that, in the sequence

$$\text{rk } \mathfrak{o} < \text{rk } \mathfrak{c}_i < \text{rk } \mathfrak{c}'_k < \text{rk } \mathfrak{c}''_m < \dots < \text{rk } \bar{\mathfrak{o}}$$

each increment is by just a few units. This way, tweaking the `push` parameter, we can reduce most of the computation to the rank pushing §1.6 during or even before (see [Remark 1.16](#)) the puzzle assembly algorithm §1.5.

## 2. SUFFICIENT COMBINATORIAL BOUNDS

For 15 of the 24 Niemeier lattices, the bound  $b(\mathfrak{D}) < 720$  follows immediately from the rough combinatorial estimates found in [\\*\\*§3](#) (see also the examples worked out in [\\*\\*§4.3](#) through [\\*\\*§4.5](#)). This computation is presented in the tables below. The meaning of the columns is as follows:

(1) index (2) vectors  $h|_k$  or  $l|_k$  (3)  $n(\bar{\mathfrak{o}})$  (4) count (5) bound,

where

- (1) is the index (see [Convention 2.1](#)) of the class of  $h \in N$  in the row starting a block (the *h-row*; in bold) and, for each  $h$ , the indices of the  $O_h(N)$ -orbits in the other rows (*l-rows*);
- (2) are the components  $h|_k \in D_k^\vee$  or  $l|_k \in D_k^\vee$  in the notation of [Convention 2.2](#);
- (3) is the number  $n(\bar{\mathfrak{o}})$  of combinatorial orbits in orbit  $\bar{\mathfrak{o}}$ ; it is marked with a \* if  $\bar{\mathfrak{o}}$  is self-dual, and with a \*\* if each combinatorial orbit  $\mathfrak{o} \subset \bar{\mathfrak{o}}$  is self-dual;
- (4) is the count  $c(\mathfrak{D})$  (in an *h-row*) or  $c(\mathfrak{o})$ , *per combinatorial orbit* (in an *l-row*);
- (5) is an estimate on the bound  $b(\mathfrak{D})$  (in an *h-row*) or  $b(\mathfrak{o})$  (in an *l-row*), see [Convention 2.3](#).

**Convention 2.1.** For references, we assign an index to each automorphism class of 4-polarizations  $h \in N$ ; a description of these classes (the *h-row*) starts each block of the table and their indices are shown in bold. The remaining rows of each block (the *l-rows*) correspond to the  $O_h(N)$ -orbits  $\bar{\mathfrak{o}}_1, \bar{\mathfrak{o}}_2, \dots$ , also indexed in a certain way, and show a “typical” combinatorial orbit  $\mathfrak{o} \subset \bar{\mathfrak{o}}_n$ . If an orbit  $\bar{\mathfrak{o}}_n$  is not self-dual (no \* or \*\* in the third column), it is understood that  $\bar{\mathfrak{o}}_n^* = \bar{\mathfrak{o}}_{n+1}$  and the latter orbit is omitted from the tables. This fact explains the gaps in the indexing.

**Convention 2.2.** The second column splits into several subcolumns, one for each block  $D_k$  in the decomposition

$$N := N(D) = N\left(\bigoplus_k D_k\right), \quad k \in \Omega,$$

see [\\*\\*§3.1](#). In the *l-rows*, we show a representative  $l$  of one of the combinatorial orbits constituting the given orbit, in terms of the invariants described in [\\*\\*§3.4](#).

For the components  $h|_k \in D_k^\vee$  of  $h$  we use the notation  $[h|_k^2]_d$ , whereas for those of a conic  $l$  we use  $[l|_k \cdot h|_k]_d$ . The subscript  $d$  is either 0,  $\circ$ , or  $\bullet$  if the argument ( $h|_k$  or  $l|_k$ ) is an integral vector of square 0, 2, or 4, respectively, *cf.* [\\*\\*§3.3](#), or a positive integer if the argument is a shortest vector in the discriminant class  $\underline{d}$ , in the notation of [\\*\\*§3.3](#) again.

*For short vectors*, these data mostly determine the pair  $(h|_k, l|_k)$  up to  $R(D_k)$ , and the occasional superscripts are mainly artifacts left over from other papers where longer vectors  $h$  were considered. A notable exception is the pair  $\begin{smallmatrix} 2 \\ \bullet \end{smallmatrix}$  representing a square 4 vector  $\pm 2e_i \in \mathbf{D}_n$  (as opposed to  $\mathbf{1}_u$ ,  $|u| = 4$ ), see the description of  $\mathbf{D}_n$  in [\\*\\*§3.3](#).

**Convention 2.3.** Shown in the fifth column is an estimate on  $b(\mathfrak{o})$  *per single combinatorial orbit*. The original estimates are given by [\\*\\*§3.14](#). Occasionally, this naïve estimate can be reduced; this fact is indicated *via*

$$(\text{old bound}) \rightarrow (\text{new bound})(\text{reason}),$$

with a reference to one of the following reasons:

- \* the bound has been reduced by [\\*\\*Lemma 3.37](#);
- ✓ the sharp bound has been obtained by brute force [§1.4](#);
- † a partial computation has been performed, without the goal  $\min := m$  set, see [§1.4](#);
- ‡ a full computation as in [§1.4](#) has been performed, but the  $\min := m$  goal has not been achieved, so that the sharp bound is still not known.

The bounds  $b(\mathfrak{o})$  known to be sharp are underlined.

Needless to say that the tables were compiled by GAP as one of the outcomes of the algorithm; in particular, that is why we do not have full control over the superscripts in [Convention 2.2](#).

2.1. **The lattice  $N(\mathbf{D}_{24})$ .** There are 2 classes;  $b(\mathfrak{O}) \leq 337$ .

|           |                   |          |       |     |
|-----------|-------------------|----------|-------|-----|
| <b>1:</b> | $[4]_{\bullet}^2$ |          | 14168 | 337 |
| <b>1:</b> | $[2]_{\bullet}^-$ | $1^{**}$ | 14168 | 337 |
| <b>2:</b> | $[4]_{\bullet}$   |          | 4568  | 122 |
| <b>1:</b> | $[2]_{\bullet}^+$ | $1^{**}$ | 4560  | 120 |
| <b>2:</b> | $[2]_{\bullet}^2$ | 1        | 4     | 1   |

2.2. **The lattice  $N(\mathbf{D}_{16} \oplus \mathbf{E}_8)$ .** There are 5 classes;  $b(\mathfrak{O}) \leq 370$ .

|           |                   |                 |          |       |     |
|-----------|-------------------|-----------------|----------|-------|-----|
| <b>1:</b> | $[4]_{\bullet}^2$ | $[0]_0$         |          | 10840 | 370 |
| <b>1:</b> | $[2]_{\bullet}^-$ | $[0]_0$         | $1^{**}$ | 3640  | 130 |
| <b>2:</b> | $[2]_{\circ}$     | $[0]_{\circ}$   | $1^{**}$ | 7200  | 240 |
| <b>2:</b> | $[4]_1$           | $[0]_0$         |          | 3640  | 280 |
| <b>1:</b> | $[2]_1$           | $[0]_0$         | 1        | 1820  | 140 |
| <b>3:</b> | $[4]_{\bullet}$   | $[0]_0$         |          | 5080  | 250 |
| <b>1:</b> | $[2]_1$           | $[0]_0$         | $1^{**}$ | 2048  | 128 |
| <b>2:</b> | $[2]_{\bullet}^+$ | $[0]_0$         | $1^{**}$ | 1584  | 72  |
| <b>3:</b> | $[2]_{\circ}$     | $[0]_{\circ}$   | $1^{**}$ | 1440  | 48  |
| <b>4:</b> | $[2]_{\bullet}^2$ | $[0]_0$         | 1        | 4     | 1   |
| <b>4:</b> | $[0]_0$           | $[4]_{\bullet}$ |          | 7000  | 240 |
| <b>1:</b> | $[0]_{\circ}$     | $[2]_{\circ}$   | $1^{**}$ | 6720  | 224 |
| <b>2:</b> | $[0]_0$           | $[2]_{\bullet}$ | $1^{**}$ | 280   | 16  |
| <b>5:</b> | $[2]_{\circ}$     | $[2]_{\circ}$   |          | 4120  | 212 |
| <b>1:</b> | $[1]_{\circ}$     | $[1]_{\circ}$   | $1^{**}$ | 3136  | 168 |
| <b>2:</b> | $[2]_{\bullet}$   | $[0]_0$         | 1        | 364   | 14  |
| <b>4:</b> | $[2]_{\bullet}^2$ | $[0]_0$         | 1        | 2     | 1   |
| <b>6:</b> | $[2]_{\circ}$     | $[0]_{\circ}$   | 1        | 126   | 7   |



2.3. **The lattice  $N(3E_8)$ .** There are 2 classes;  $b(\mathfrak{O}) \leq 240$ .

|           |                 |         |         |          |     |
|-----------|-----------------|---------|---------|----------|-----|
| <b>1:</b> | $[4]_{\bullet}$ | $[0]_0$ | $[0]_0$ | 7000     | 240 |
| 1:        | $[2]_{\bullet}$ | $[0]_0$ | $[0]_0$ | 1** 280  | 16  |
| 2:        | $[2]_0$         | $[0]_0$ | $[0]_0$ | 2** 3360 | 112 |
| <b>2:</b> | $[2]_0$         | $[2]_0$ | $[0]_0$ | 4120     | 212 |
| 1:        | $[2]_0$         | $[0]_0$ | $[0]_0$ | 2* 240   | 8   |
| 2:        | $[1]_0$         | $[1]_0$ | $[0]_0$ | 1** 3136 | 168 |
| 3:        | $[2]_{\bullet}$ | $[0]_0$ | $[0]_0$ | 2 126    | 7   |

2.4. **The lattice  $N(A_{24})$ .** There are 2 classes;  $b(\mathfrak{O}) \leq 240$ .

|           |                   |          |     |
|-----------|-------------------|----------|-----|
| <b>1:</b> | $[4]_{\bullet}$   | 4760     | 240 |
| 1:        | $[2]_{20}$        | 2* 1330  | 70  |
| 2:        | $[2]_{\bullet}^+$ | 2* 210   | 10  |
| 3:        | $[2]_{\bullet}^-$ | 1** 1680 | 80  |
| <b>2:</b> | $[4]_{20}$        | 3800     | 200 |
| 1:        | $[2]_{20}$        | 1 1900   | 100 |

2.5. **The lattice  $N(2D_{12})$ .** There are 4 classes;  $b(\mathfrak{O}) \leq 458$ .

|           |                   |         |          |                         |
|-----------|-------------------|---------|----------|-------------------------|
| <b>1:</b> | $[4]_{\bullet}^2$ | $[0]_0$ | 9176     | 458                     |
| 1:        | $[2]_{\bullet}^-$ | $[0]_0$ | 1** 1320 | 66                      |
| 2:        | $[2]_0$           | $[0]_0$ | 1** 5808 | 264                     |
| 3:        | $[2]_2$           | $[0]_1$ | 1** 2048 | 128                     |
| <b>2:</b> | $[2]_0$           | $[2]_0$ | 4376     | 292                     |
| 1:        | $[1]_1$           | $[1]_2$ | 2** 1024 | 64                      |
| 2:        | $[1]_0$           | $[1]_0$ | 1** 1600 | 120                     |
| 3:        | $[2]_{\bullet}$   | $[0]_0$ | 2 180    | 10                      |
| 5:        | $[2]_{\bullet}^2$ | $[0]_0$ | 2 2      | 1                       |
| <b>3:</b> | $[4]_{\bullet}$   | $[0]_0$ | 5336     | 314 $\rightarrow$ 258   |
| 1:        | $[2]_{\bullet}^+$ | $[0]_0$ | 1** 672  | 48                      |
| 2:        | $[2]_1$           | $[0]_2$ | 1** 3072 | 192 $\rightarrow$ 136 * |
| 3:        | $[2]_0$           | $[0]_0$ | 1** 1584 | 72                      |
| 4:        | $[2]_{\bullet}^2$ | $[0]_0$ | 1 4      | 1                       |

---

|    |                   |               |   |      |     |               |      |
|----|-------------------|---------------|---|------|-----|---------------|------|
| 4: | $[1]_2$           | $[3]_1$       |   | 3896 | 362 | $\rightarrow$ | 242  |
| 1: | $[2]_{\bullet}^2$ | $[0]_0$       | 1 |      | 1   |               | 1    |
| 3: | $[1]_{\circ}$     | $[1]_{\circ}$ | 1 | 1452 | 132 | $\rightarrow$ | 72 * |
| 5: | $[1]_2$           | $[1]_1$       | 1 | 495  | 48  |               |      |

---

2.6. **The lattice  $N(\mathbf{A}_{17} \oplus \mathbf{E}_7)$ .** There are 5 classes;  $b(\mathfrak{O}) \leq 372$ .

---

|    |               |                   |     |      |     |
|----|---------------|-------------------|-----|------|-----|
| 1: | $[0]_0$       | $[4]_{\bullet}$   |     | 6424 | 372 |
| 1: | $[0]_{15}$    | $[2]_1$           | 2*  | 1632 | 96  |
| 2: | $[0]_{\circ}$ | $[2]_{\circ}$     | 1** | 3060 | 170 |
| 3: | $[0]_0$       | $[2]_{\bullet}^+$ | 1** | 80   | 8   |
| 4: | $[0]_0$       | $[2]_{\bullet}^-$ | 1** | 20   | 2   |

---

|    |                   |               |     |      |     |
|----|-------------------|---------------|-----|------|-----|
| 2: | $[4]_{\bullet}$   | $[0]_0$       |     | 4984 | 360 |
| 1: | $[2]_{12}$        | $[0]_0$       | 2*  | 1001 | 91  |
| 2: | $[2]_{\bullet}^+$ | $[0]_0$       | 2*  | 91   | 7   |
| 3: | $[2]_{\bullet}^-$ | $[0]_0$       | 1** | 728  | 52  |
| 4: | $[2]_{15}$        | $[0]_1$       | 2*  | 784  | 42  |
| 5: | $[2]_{\circ}$     | $[0]_{\circ}$ | 1** | 504  | 28  |

---

|    |            |         |     |      |     |
|----|------------|---------|-----|------|-----|
| 3: | $[4]_{12}$ | $[0]_0$ |     | 4024 | 332 |
| 1: | $[2]_6$    | $[0]_0$ | 1** | 924  | 92  |
| 2: | $[2]_{15}$ | $[0]_1$ | 1** | 1120 | 60  |
| 3: | $[2]_{12}$ | $[0]_0$ | 1   | 990  | 90  |

---

|    |                 |               |    |      |     |
|----|-----------------|---------------|----|------|-----|
| 4: | $[2]_{\circ}$   | $[2]_{\circ}$ |    | 4504 | 298 |
| 1: | $[1]_{15}$      | $[1]_1$       | 2* | 1440 | 96  |
| 2: | $[1]_{\circ}^+$ | $[1]_{\circ}$ | 2* | 512  | 32  |
| 3: | $[2]_{\bullet}$ | $[0]_0$       | 1  | 240  | 15  |
| 5: | $[2]_{\circ}$   | $[0]_{\circ}$ | 1  | 60   | 6   |

---

|    |                      |                   |   |      |     |
|----|----------------------|-------------------|---|------|-----|
| 5: | $[\frac{5}{2}]_{15}$ | $[\frac{3}{2}]_1$ |   | 4024 | 280 |
| 1: | $[2]_{12}$           | $[0]_0$           | 1 | 455  | 35  |
| 3: | $[2]_{\bullet}$      | $[0]_0$           | 1 | 315  | 21  |
| 5: | $[\frac{5}{2}]_{15}$ | $[\frac{1}{2}]_1$ | 1 | 27   | 3   |
| 7: | $[\frac{3}{2}]_{15}$ | $[\frac{1}{2}]_1$ | 1 | 1215 | 81  |

---

2.7. **The lattice  $N(\mathbf{D}_{10} \oplus 2\mathbf{E}_7)$ .** There are 7 classes;  $b(\mathfrak{O}) \leq 462$ .

|           |                   |                   |                   |          |                         |
|-----------|-------------------|-------------------|-------------------|----------|-------------------------|
| <b>1:</b> | $[4]_{\bullet}^2$ | $[0]_0$           | $[0]_0$           | 8344     | 462                     |
| 1:        | $[2]_{\bullet}^-$ | $[0]_0$           | $[0]_0$           | 1** 672  | 42                      |
| 2:        | $[2]_{\circ}$     | $[0]_{\circ}$     | $[0]_0$           | 2** 2268 | 126                     |
| 3:        | $[2]_2$           | $[0]_1$           | $[0]_1$           | 1** 3136 | 168                     |
| <b>2:</b> | $[\frac{5}{2}]_3$ | $[0]_0$           | $[\frac{3}{2}]_1$ | 4024     | 378                     |
| 1:        | $[2]_{\bullet}$   | $[0]_0$           | $[0]_0$           | 1 210    | 21                      |
| 3:        | $[\frac{5}{2}]_3$ | $[0]_0$           | $[\frac{1}{2}]_1$ | 1 27     | 3                       |
| 5:        | $[2]_1$           | $[0]_1$           | $[0]_0$           | 1 560    | 30                      |
| 7:        | $[\frac{3}{2}]_3$ | $[0]_0$           | $[\frac{1}{2}]_1$ | 1 1215   | 135                     |
| <b>3:</b> | $[0]_0$           | $[4]_{\bullet}$   | $[0]_0$           | 6424     | 364 $\rightarrow$ 362   |
| 1:        | $[0]_1$           | $[2]_1$           | $[0]_0$           | 1** 1024 | 64                      |
| 2:        | $[0]_{\circ}$     | $[2]_{\circ}$     | $[0]_0$           | 1** 1800 | 100                     |
| 3:        | $[0]_2$           | $[2]_1$           | $[0]_1$           | 1** 2240 | 120 $\rightarrow$ 118 * |
| 4:        | $[0]_0$           | $[2]_{\bullet}^+$ | $[0]_0$           | 1** 80   | 8                       |
| 5:        | $[0]_0$           | $[2]_{\bullet}^-$ | $[0]_0$           | 1** 20   | 2                       |
| 6:        | $[0]_0$           | $[2]_{\circ}$     | $[0]_{\circ}$     | 1** 1260 | 70                      |
| <b>4:</b> | $[1]_2$           | $[\frac{3}{2}]_1$ | $[\frac{3}{2}]_1$ | 4024     | 424 $\rightarrow$ 328   |
| 1:        | $[\frac{1}{2}]_3$ | $[0]_0$           | $[\frac{3}{2}]_1$ | 2* 256   | 16                      |
| 2:        | $[2]_{\bullet}^2$ | $[0]_0$           | $[0]_0$           | 1 1      | 1                       |
| 4:        | $[1]_{\circ}$     | $[1]_{\circ}$     | $[0]_0$           | 2 486    | 54 $\rightarrow$ 30 *   |
| 6:        | $[1]_2$           | $[\frac{3}{2}]_1$ | $[\frac{1}{2}]_1$ | 2 27     | 3                       |
| 8:        | $[1]_2$           | $[\frac{1}{2}]_1$ | $[\frac{1}{2}]_1$ | 1 729    | 81                      |
| <b>5:</b> | $[4]_{\bullet}$   | $[0]_0$           | $[0]_0$           | 5464     | 314                     |
| 1:        | $[2]_{\bullet}^+$ | $[0]_0$           | $[0]_0$           | 1** 360  | 36                      |
| 2:        | $[2]_3$           | $[0]_0$           | $[0]_1$           | 2** 1792 | 96                      |
| 3:        | $[2]_{\circ}$     | $[0]_{\circ}$     | $[0]_0$           | 2** 756  | 42                      |
| 4:        | $[2]_{\bullet}^2$ | $[0]_0$           | $[0]_0$           | 1 4      | 1                       |
| <b>6:</b> | $[0]_0$           | $[2]_{\circ}$     | $[2]_{\circ}$     | 4504     | 428 $\rightarrow$ 308   |
| 1:        | $[0]_{\circ}$     | $[2]_{\circ}$     | $[0]_0$           | 2* 180   | 10                      |
| 2:        | $[0]_2$           | $[1]_1$           | $[1]_1$           | 1** 2880 | 288 $\rightarrow$ 168 * |
| 3:        | $[0]_0$           | $[1]_{\circ}$     | $[1]_{\circ}$     | 1** 1024 | 96                      |
| 4:        | $[0]_0$           | $[2]_{\bullet}$   | $[0]_0$           | 2 60     | 6                       |
| <b>7:</b> | $[2]_{\circ}$     | $[2]_{\circ}$     | $[0]_0$           | 4504     | 308                     |
| 1:        | $[1]_1$           | $[1]_1$           | $[0]_0$           | 1** 1536 | 96                      |

|     |                   |               |               |          |      |    |
|-----|-------------------|---------------|---------------|----------|------|----|
| 2:  | $[1]_{\circ}$     | $[1]_{\circ}$ | $[0]_0$       | $1^{**}$ | 1024 | 96 |
| 3:  | $[1]_2$           | $[1]_1$       | $[0]_1$       | $1^{**}$ | 1344 | 72 |
| 4:  | $[2]_{\bullet}$   | $[0]_0$       | $[0]_0$       | 1        | 112  | 8  |
| 6:  | $[2]_{\bullet}^2$ | $[0]_0$       | $[0]_0$       | 1        | 2    | 1  |
| 8:  | $[2]_{\circ}$     | $[0]_{\circ}$ | $[0]_0$       | 1        | 60   | 6  |
| 10: | $[2]_{\circ}$     | $[0]_0$       | $[0]_{\circ}$ | 1        | 126  | 7  |

2.8. **The lattice  $N(\mathbf{A}_{15} \oplus \mathbf{D}_9)$ .** There are 7 classes;  $b(\mathfrak{D}) \leq 550$ .

|           |                      |                   |          |      |                        |
|-----------|----------------------|-------------------|----------|------|------------------------|
| <b>1:</b> | $[0]_0$              | $[4]_{\bullet}^2$ |          | 7928 | 550                    |
| 1:        | $[0]_{12}$           | $[2]_2$           | $2^*$    | 1820 | 140                    |
| 2:        | $[0]_{\circ}$        | $[2]_{\circ}$     | $1^{**}$ | 3840 | 240                    |
| 3:        | $[0]_0$              | $[2]_{\bullet}^-$ | $1^{**}$ | 448  | 30                     |
| <b>2:</b> | $[4]_8$              | $[0]_0$           |          | 4088 | $504 \rightarrow 380$  |
| 1:        | $[2]_{12}$           | $[0]_2$           | $2^{**}$ | 1260 | $140 \rightarrow 78^*$ |
| 2:        | $[2]_8$              | $[0]_0$           | 1        | 784  | 112                    |
| <b>3:</b> | $[0]_0$              | $[4]_{\bullet}$   |          | 5528 | 378                    |
| 1:        | $[0]_{\circ}$        | $[2]_{\circ}$     | $1^{**}$ | 1440 | 90                     |
| 2:        | $[0]_{14}$           | $[2]_3$           | $2^*$    | 1920 | 128                    |
| 3:        | $[0]_0$              | $[2]_{\bullet}^+$ | $1^{**}$ | 240  | 30                     |
| 4:        | $[0]_0$              | $[2]_{\bullet}^2$ | 1        | 4    | 1                      |
| <b>4:</b> | $[4]_{\bullet}$      | $[0]_0$           |          | 5048 | $432 \rightarrow 360$  |
| 1:        | $[2]_8$              | $[0]_0$           | $1^{**}$ | 924  | 92                     |
| 2:        | $[2]_{\bullet}^+$    | $[0]_0$           | $2^*$    | 66   | 6                      |
| 3:        | $[2]_{\bullet}^-$    | $[0]_0$           | $1^{**}$ | 528  | 44                     |
| 4:        | $[2]_{12}$           | $[0]_2$           | $2^*$    | 1188 | $108 \rightarrow 72^*$ |
| 5:        | $[2]_{\circ}$        | $[0]_{\circ}$     | $1^{**}$ | 576  | 36                     |
| 6:        | $[2]_{14}$           | $[0]_3$           | $2^*$    | 256  | 16                     |
| <b>5:</b> | $[2]_{\circ}$        | $[2]_{\circ}$     |          | 4568 | 338                    |
| 1:        | $[1]_{12}$           | $[1]_2$           | $2^*$    | 728  | 56                     |
| 2:        | $[1]_{\circ}^+$      | $[1]_{\circ}$     | $2^*$    | 392  | 28                     |
| 3:        | $[1]_{14}$           | $[1]_3$           | $2^*$    | 896  | 64                     |
| 4:        | $[2]_{\bullet}$      | $[0]_0$           | 1        | 182  | 13                     |
| 6:        | $[2]_{\circ}$        | $[0]_{\circ}^+$   | 1        | 84   | 7                      |
| 8:        | $[2]_{\circ}$        | $[0]_{\circ}^-$   | 1        | 2    | 1                      |
| <b>6:</b> | $[3]_{12}$           | $[1]_2$           |          | 4088 | $346 \rightarrow 322$  |
| 1:        | $[\frac{3}{2}]_{14}$ | $[\frac{1}{2}]_3$ | $1^{**}$ | 768  | 48                     |

|       |                      |                   |   |      |                       |
|-------|----------------------|-------------------|---|------|-----------------------|
| 2:    | $[2]_8$              | $[0]_0$           | 1 | 495  | 48                    |
| 4:    | $[2]_\bullet$        | $[0]_0$           | 1 | 396  | 36                    |
| 6:    | $[3]_{12}$           | $[-1]_2$          | 1 | 1    | 1                     |
| 8:    | $[2]_{12}$           | $[0]_2$           | 1 | 768  | $64 \rightarrow 52^*$ |
| <hr/> |                      |                   |   |      |                       |
| 7:    | $[\frac{7}{4}]_{14}$ | $[\frac{9}{4}]_3$ |   | 4088 | 310                   |
| 1:    | $[2]_\bullet$        | $[0]_0$           | 1 | 91   | 7                     |
| 3:    | $[\frac{3}{2}]_{12}$ | $[\frac{1}{2}]_2$ | 1 | 819  | 63                    |
| 5:    | $[1]_\circ$          | $[1]_\circ$       | 1 | 1008 | 72                    |
| 7:    | $[\frac{7}{4}]_{14}$ | $[\frac{1}{4}]_3$ | 1 | 126  | 13                    |

2.9. **The lattice  $N(2\mathbf{A}_{12})$ .** There are 4 classes;  $b(\mathfrak{D}) \leq 436$ .

|       |                        |                        |          |      |     |
|-------|------------------------|------------------------|----------|------|-----|
| 1:    | $[2]_\circ$            | $[2]_\circ$            |          | 4664 | 436 |
| 1:    | $[1]_8$                | $[1]_1$                | $4^*$    | 330  | 33  |
| 2:    | $[1]_{10}$             | $[1]_{11}$             | $4^*$    | 605  | 55  |
| 3:    | $[1]_\circ^+$          | $[1]_\circ^+$          | $4^*$    | 121  | 11  |
| 4:    | $[2]_\bullet$          | $[0]_0$                | 2        | 110  | 10  |
| <hr/> |                        |                        |          |      |     |
| 2:    | $[4]_\bullet$          | $[0]_0$                |          | 5144 | 416 |
| 1:    | $[2]_\bullet^+$        | $[0]_0$                | $2^*$    | 36   | 4   |
| 2:    | $[2]_\bullet^-$        | $[0]_0$                | $1^{**}$ | 288  | 32  |
| 3:    | $[2]_8$                | $[0]_1$                | $2^*$    | 1092 | 84  |
| 4:    | $[2]_{10}$             | $[0]_{11}$             | $2^*$    | 702  | 54  |
| 5:    | $[2]_\circ$            | $[0]_\circ$            | $1^{**}$ | 624  | 48  |
| 6:    | $[2]_{11}$             | $[0]_3$                | $2^*$    | 286  | 26  |
| <hr/> |                        |                        |          |      |     |
| 3:    | $[\frac{22}{13}]_{11}$ | $[\frac{30}{13}]_3$    |          | 4184 | 398 |
| 1:    | $[\frac{11}{13}]_{12}$ | $[\frac{15}{13}]_8$    | $1^{**}$ | 504  | 52  |
| 2:    | $[2]_\bullet$          | $[0]_0$                | 1        | 55   | 5   |
| 4:    | $[\frac{16}{13}]_8$    | $[\frac{10}{13}]_1$    | 1        | 495  | 48  |
| 6:    | $[\frac{20}{13}]_{10}$ | $[\frac{6}{13}]_{11}$  | 1        | 495  | 45  |
| 8:    | $[1]_\circ$            | $[1]_\circ$            | 1        | 660  | 60  |
| 10:   | $[\frac{22}{13}]_{11}$ | $[\frac{4}{13}]_3$     | 1        | 135  | 15  |
| <hr/> |                        |                        |          |      |     |
| 4:    | $[\frac{12}{13}]_{12}$ | $[\frac{40}{13}]_8$    |          | 4184 | 392 |
| 1:    | $[\frac{10}{13}]_{10}$ | $[\frac{16}{13}]_{11}$ | 1        | 660  | 60  |
| 3:    | $[1]_\circ$            | $[1]_\circ$            | 1        | 480  | 40  |
| 5:    | $[\frac{11}{13}]_{11}$ | $[\frac{15}{13}]_3$    | 1        | 672  | 56  |
| 7:    | $[\frac{12}{13}]_{12}$ | $[\frac{14}{13}]_8$    | 1        | 280  | 40  |

2.10. **The lattice  $N(\mathbf{A}_{11} \oplus \mathbf{D}_7 \oplus \mathbf{E}_6)$ .** There are 12 classes;  $b(\mathfrak{D}) \leq 632$ .

|           |                   |                   |                   |          |                       |
|-----------|-------------------|-------------------|-------------------|----------|-----------------------|
| <b>1:</b> | $[0]_0$           | $[4]_{\bullet}^2$ | $[0]_0$           | 7096     | 632                   |
| 1:        | $[0]_6$           | $[2]_2$           | $[0]_0$           | 1** 924  | 92                    |
| 2:        | $[0]_{\circ}$     | $[2]_{\circ}$     | $[0]_0$           | 1** 1584 | 132                   |
| 3:        | $[0]_{10}$        | $[2]_2$           | $[0]_1$           | 2* 1782  | 162                   |
| 4:        | $[0]_0$           | $[2]_{\bullet}^-$ | $[0]_0$           | 1** 160  | 12                    |
| 5:        | $[0]_0$           | $[2]_{\circ}$     | $[0]_{\circ}$     | 1** 864  | 72                    |
| <b>2:</b> | $[0]_0$           | $[0]_0$           | $[4]_{\bullet}$   | 6136     | 534 $\rightarrow$ 510 |
| 1:        | $[0]_8$           | $[0]_0$           | $[2]_2$           | 2* 495   | 48                    |
| 2:        | $[0]_{\circ}$     | $[0]_0$           | $[2]_{\circ}$     | 1** 1056 | 88                    |
| 3:        | $[0]_{10}$        | $[0]_2$           | $[2]_1$           | 2* 924   | 84 $\rightarrow$ 72*  |
| 4:        | $[0]_{11}$        | $[0]_3$           | $[2]_2$           | 2* 768   | 60                    |
| 5:        | $[0]_0$           | $[0]_{\circ}$     | $[2]_{\circ}$     | 1** 672  | 56                    |
| 6:        | $[0]_0$           | $[0]_0$           | $[2]_{\bullet}^+$ | 2* 1     | 1                     |
| 7:        | $[0]_0$           | $[0]_0$           | $[2]_{\bullet}^-$ | 1** 32   | 4                     |
| <b>3:</b> | $[2]_{\circ}$     | $[2]_{\circ}$     | $[0]_0$           | 4696     | 498                   |
| 1:        | $[1]_6$           | $[1]_2$           | $[0]_0$           | 1** 504  | 52                    |
| 2:        | $[1]_9$           | $[1]_1$           | $[0]_0$           | 2* 720   | 80                    |
| 3:        | $[1]_{\circ}^+$   | $[1]_{\circ}$     | $[0]_0$           | 2* 200   | 20                    |
| 4:        | $[1]_{10}$        | $[1]_2$           | $[0]_1$           | 2* 540   | 54                    |
| 5:        | $[1]_{11}$        | $[1]_3$           | $[0]_2$           | 2* 432   | 48                    |
| 6:        | $[2]_{\bullet}$   | $[0]_0$           | $[0]_0$           | 1 90     | 9                     |
| 8:        | $[2]_{\circ}$     | $[0]_{\circ}^+$   | $[0]_0$           | 1 40     | 5                     |
| 10:       | $[2]_{\circ}$     | $[0]_{\circ}^-$   | $[0]_0$           | 1 2      | 1                     |
| 12:       | $[2]_{\circ}$     | $[0]_0$           | $[0]_{\circ}$     | 1 72     | 6                     |
| <b>4:</b> | $[0]_0$           | $[4]_{\bullet}$   | $[0]_0$           | 5656     | 490                   |
| 1:        | $[0]_9$           | $[2]_1$           | $[0]_0$           | 2* 880   | 80                    |
| 2:        | $[0]_{\circ}$     | $[2]_{\circ}$     | $[0]_0$           | 1** 792  | 66                    |
| 3:        | $[0]_{11}$        | $[2]_3$           | $[0]_2$           | 2* 1296  | 108                   |
| 4:        | $[0]_0$           | $[2]_{\bullet}^+$ | $[0]_0$           | 1** 72   | 10                    |
| 5:        | $[0]_0$           | $[2]_{\circ}$     | $[0]_{\circ}$     | 1** 432  | 36                    |
| 6:        | $[0]_0$           | $[2]_{\bullet}^2$ | $[0]_0$           | 1 4      | 1                     |
| <b>5:</b> | $[3]_6$           | $[1]_2$           | $[0]_0$           | 4216     | 536 $\rightarrow$ 476 |
| 1:        | $[\frac{3}{2}]_9$ | $[\frac{1}{2}]_1$ | $[0]_0$           | 2** 640  | 60                    |
| 2:        | $[2]_{\bullet}$   | $[0]_0$           | $[0]_0$           | 1 225    | 45                    |
| 4:        | $[3]_6$           | $[-1]_2$          | $[0]_0$           | 1 1      | 1                     |

|            |                      |                   |                   |          |      |                        |
|------------|----------------------|-------------------|-------------------|----------|------|------------------------|
| 6:         | $[2]_6$              | $[0]_2$           | $[0]_0$           | 1        | 432  | $72 \rightarrow 42 *$  |
| 8:         | $[2]_8$              | $[0]_0$           | $[0]_2$           | 2        | 405  | 45                     |
| <hr/>      |                      |                   |                   |          |      |                        |
| <b>6:</b>  | $[4]_{\bullet}$      | $[0]_0$           | $[0]_0$           |          | 5176 | $532 \rightarrow 474$  |
| 1:         | $[2]_{\bullet}^+$    | $[0]_0$           | $[0]_0$           | $2^*$    | 28   | 4                      |
| 2:         | $[2]_{\bullet}^-$    | $[0]_0$           | $[0]_0$           | $1^{**}$ | 224  | 28                     |
| 3:         | $[2]_6$              | $[0]_2$           | $[0]_0$           | $1^{**}$ | 980  | $112 \rightarrow 78 *$ |
| 4:         | $[2]_8$              | $[0]_0$           | $[0]_2$           | $2^*$    | 756  | 84                     |
| 5:         | $[2]_9$              | $[0]_1$           | $[0]_0$           | $2^*$    | 512  | 40                     |
| 6:         | $[2]_{\circ}$        | $[0]_{\circ}$     | $[0]_0$           | $1^{**}$ | 336  | 28                     |
| 7:         | $[2]_{\circ}$        | $[0]_0$           | $[0]_{\circ}$     | $1^{**}$ | 288  | 24                     |
| 8:         | $[2]_{10}$           | $[0]_2$           | $[0]_1$           | $2^*$    | 378  | $42 \rightarrow 30 *$  |
| <hr/>      |                      |                   |                   |          |      |                        |
| <b>7:</b>  | $[\frac{9}{4}]_9$    | $[\frac{7}{4}]_1$ | $[0]_0$           |          | 4216 | 466                    |
| 1:         | $[2]_{\bullet}$      | $[0]_0$           | $[0]_0$           | 1        | 108  | 12                     |
| 3:         | $[\frac{3}{2}]_6$    | $[\frac{1}{2}]_2$ | $[0]_0$           | 1        | 588  | 63                     |
| 5:         | $[2]_8$              | $[0]_0$           | $[0]_2$           | 1        | 243  | 27                     |
| 7:         | $[\frac{9}{4}]_9$    | $[\frac{1}{4}]_1$ | $[0]_0$           | 1        | 35   | 5                      |
| 9:         | $[\frac{5}{4}]_9$    | $[\frac{3}{4}]_1$ | $[0]_0$           | 1        | 567  | 63                     |
| 11:        | $[\frac{3}{2}]_{10}$ | $[\frac{1}{2}]_2$ | $[0]_1$           | 1        | 567  | 63                     |
| <hr/>      |                      |                   |                   |          |      |                        |
| <b>8:</b>  | $[0]_0$              | $[2]_{\circ}$     | $[2]_{\circ}$     |          | 4696 | 440                    |
| 1:         | $[0]_{10}$           | $[1]_2$           | $[1]_1$           | $2^*$    | 792  | 72                     |
| 2:         | $[0]_{11}$           | $[1]_3$           | $[1]_2$           | $2^*$    | 1152 | 96                     |
| 3:         | $[0]_0$              | $[1]_{\circ}$     | $[1]_{\circ}$     | $1^{**}$ | 400  | 60                     |
| 4:         | $[0]_{\circ}$        | $[2]_{\circ}$     | $[0]_0$           | 1        | 132  | 11                     |
| 6:         | $[0]_0$              | $[2]_{\bullet}$   | $[0]_0$           | 1        | 40   | 5                      |
| 8:         | $[0]_0$              | $[2]_{\bullet}^2$ | $[0]_0$           | 1        | 2    | 1                      |
| 10:        | $[0]_0$              | $[2]_{\circ}$     | $[0]_{\circ}$     | 1        | 30   | 5                      |
| <hr/>      |                      |                   |                   |          |      |                        |
| <b>9:</b>  | $[\frac{8}{3}]_8$    | $[0]_0$           | $[\frac{4}{3}]_2$ |          | 4216 | $532 \rightarrow 436$  |
| 1:         | $[\frac{4}{3}]_4$    | $[0]_0$           | $[\frac{2}{3}]_1$ | $1^{**}$ | 700  | 80                     |
| 2:         | $[\frac{4}{3}]_{10}$ | $[0]_2$           | $[\frac{2}{3}]_1$ | $1^{**}$ | 840  | $120 \rightarrow 72 *$ |
| 3:         | $[2]_{\bullet}$      | $[0]_0$           | $[0]_0$           | 1        | 168  | 24                     |
| 5:         | $[2]_6$              | $[0]_2$           | $[0]_0$           | 1        | 392  | $56 \rightarrow 32 *$  |
| 7:         | $[\frac{8}{3}]_8$    | $[0]_0$           | $[\frac{2}{3}]_2$ | 1        | 10   | 2                      |
| 9:         | $[\frac{5}{3}]_8$    | $[0]_0$           | $[\frac{1}{3}]_2$ | 1        | 512  | 64                     |
| 11:        | $[2]_9$              | $[0]_1$           | $[0]_0$           | 1        | 256  | 20                     |
| <hr/>      |                      |                   |                   |          |      |                        |
| <b>10:</b> | $[\frac{5}{3}]_{10}$ | $[1]_2$           | $[\frac{4}{3}]_1$ |          | 4216 | $438 \rightarrow 422$  |
| 1:         | $[\frac{5}{6}]_{11}$ | $[\frac{1}{2}]_3$ | $[\frac{2}{3}]_2$ | $1^{**}$ | 640  | 60                     |

|       |                        |                   |                   |       |      |                       |
|-------|------------------------|-------------------|-------------------|-------|------|-----------------------|
| 2:    | $[2]_{\bullet}$        | $[0]_0$           | $[0]_0$           | 1     | 45   | 5                     |
| 4:    | $[1]_6$                | $[1]_2$           | $[0]_0$           | 1     | 210  | 21                    |
| 6:    | $[\frac{4}{3}]_8$      | $[0]_0$           | $[\frac{2}{3}]_2$ | 1     | 450  | 50                    |
| 8:    | $[\frac{3}{2}]_9$      | $[\frac{1}{2}]_1$ | $[0]_0$           | 1     | 320  | 30                    |
| 10:   | $[1]_{\circ}$          | $[1]_{\circ}$     | $[0]_0$           | 1     | 240  | $24 \rightarrow 22 *$ |
| 12:   | $[1]_{\circ}$          | $[0]_0$           | $[1]_{\circ}$     | 1     | 320  | 32                    |
| 14:   | $[\frac{5}{3}]_{10}$   | $[1]_2$           | $[\frac{2}{3}]_1$ | 1     | 10   | 2                     |
| 16:   | $[\frac{5}{3}]_{10}$   | $[0]_2$           | $[\frac{1}{3}]_1$ | 1     | 192  | $24 \rightarrow 18 *$ |
| 18:   | $[\frac{5}{3}]_{10}$   | $[-1]_2$          | $[\frac{4}{3}]_1$ | 1     | 1    | 1                     |
| <hr/> |                        |                   |                   |       |      |                       |
| 11:   | $[2]_{\circ}$          | $[0]_0$           | $[2]_{\circ}$     |       | 4696 | $454 \rightarrow 418$ |
| 1:    | $[1]_8$                | $[0]_0$           | $[1]_2$           | $2^*$ | 720  | 72                    |
| 2:    | $[1]_{\circ}^+$        | $[0]_0$           | $[1]_{\circ}$     | $2^*$ | 200  | 20                    |
| 3:    | $[1]_{10}$             | $[0]_2$           | $[1]_1$           | $2^*$ | 840  | $84 \rightarrow 66 *$ |
| 4:    | $[1]_{11}$             | $[0]_3$           | $[1]_2$           | $2^*$ | 384  | 30                    |
| 5:    | $[2]_{\bullet}$        | $[0]_0$           | $[0]_0$           | 1     | 90   | 9                     |
| 7:    | $[2]_{\circ}$          | $[0]_{\circ}$     | $[0]_0$           | 1     | 84   | 7                     |
| 9:    | $[2]_{\circ}$          | $[0]_0$           | $[0]_{\circ}$     | 1     | 30   | 5                     |
| <hr/> |                        |                   |                   |       |      |                       |
| 12:   | $[\frac{11}{12}]_{11}$ | $[\frac{7}{4}]_3$ | $[\frac{4}{3}]_2$ |       | 4216 | 414                   |
| 1:    | $[\frac{2}{3}]_8$      | $[0]_0$           | $[\frac{4}{3}]_2$ | 1     | 165  | 16                    |
| 3:    | $[\frac{3}{4}]_9$      | $[\frac{5}{4}]_1$ | $[0]_0$           | 1     | 385  | 35                    |
| 5:    | $[1]_{\circ}$          | $[1]_{\circ}$     | $[0]_0$           | 1     | 231  | 21                    |
| 7:    | $[1]_{\circ}$          | $[0]_0$           | $[1]_{\circ}$     | 1     | 176  | 16                    |
| 9:    | $[\frac{5}{6}]_{10}$   | $[\frac{1}{2}]_2$ | $[\frac{2}{3}]_1$ | 1     | 770  | 70                    |
| 11:   | $[\frac{11}{12}]_{11}$ | $[\frac{7}{4}]_3$ | $[\frac{2}{3}]_2$ | 1     | 10   | 2                     |
| 13:   | $[\frac{11}{12}]_{11}$ | $[\frac{3}{4}]_3$ | $[\frac{1}{3}]_2$ | 1     | 336  | 42                    |
| 15:   | $[\frac{11}{12}]_{11}$ | $[\frac{1}{4}]_3$ | $[\frac{4}{3}]_2$ | 1     | 35   | 5                     |

2.11. **The lattice  $N(4\mathbf{E}_6)$ .** There are 3 classes;  $b(\mathfrak{O}) \leq 636$ .

|       |                   |                   |                   |         |          |      |     |
|-------|-------------------|-------------------|-------------------|---------|----------|------|-----|
| 1:    | $[4]_{\bullet}$   | $[0]_0$           | $[0]_0$           | $[0]_0$ |          | 6136 | 636 |
| 1:    | $[2]_{\bullet}^+$ | $[0]_0$           | $[0]_0$           | $[0]_0$ | $2^*$    | 1    | 1   |
| 2:    | $[2]_{\bullet}^-$ | $[0]_0$           | $[0]_0$           | $[0]_0$ | $1^{**}$ | 32   | 4   |
| 3:    | $[2]_{\circ}$     | $[0]_{\circ}$     | $[0]_0$           | $[0]_0$ | $3^{**}$ | 576  | 48  |
| 4:    | $[2]_2$           | $[0]_2$           | $[0]_1$           | $[0]_0$ | $6^*$    | 729  | 81  |
| <hr/> |                   |                   |                   |         |          |      |     |
| 2:    | $[\frac{4}{3}]_2$ | $[\frac{4}{3}]_2$ | $[\frac{4}{3}]_1$ | $[0]_0$ |          | 4216 | 584 |
| 1:    | $[\frac{4}{3}]_2$ | $[\frac{2}{3}]_1$ | $[0]_0$           | $[0]_2$ | $6^*$    | 270  | 30  |
| 2:    | $[\frac{2}{3}]_1$ | $[\frac{2}{3}]_1$ | $[\frac{2}{3}]_2$ | $[0]_0$ | $1^{**}$ | 1000 | 200 |



|           |                 |               |               |         |          |      |     |
|-----------|-----------------|---------------|---------------|---------|----------|------|-----|
| 3:        | $[2]_{\bullet}$ | $[0]_0$       | $[0]_0$       | $[0]_0$ | 3        | 10   | 2   |
| 5:        | $[1]_{\circ}$   | $[1]_{\circ}$ | $[0]_0$       | $[0]_0$ | 3        | 256  | 32  |
| <hr/>     |                 |               |               |         |          |      |     |
| <b>3:</b> | $[2]_{\circ}$   | $[2]_{\circ}$ | $[0]_0$       | $[0]_0$ |          | 4696 | 536 |
| 1:        | $[2]_{\circ}$   | $[0]_0$       | $[0]_{\circ}$ | $[0]_0$ | $4^*$    | 72   | 6   |
| 2:        | $[1]_{\circ}$   | $[1]_{\circ}$ | $[0]_0$       | $[0]_0$ | $1^{**}$ | 400  | 60  |
| 3:        | $[1]_2$         | $[1]_2$       | $[0]_1$       | $[0]_0$ | $4^*$    | 972  | 108 |
| 4:        | $[2]_{\bullet}$ | $[0]_0$       | $[0]_0$       | $[0]_0$ | 2        | 30   | 5   |

2.12. **The lattice  $N(2\mathbf{A}_9 \oplus \mathbf{D}_6)$ .** There are 9 classes;  $b(\mathfrak{D}) \leq 668$ .

|           |                   |               |                   |          |      |                       |
|-----------|-------------------|---------------|-------------------|----------|------|-----------------------|
| <b>1:</b> | $[0]_0$           | $[0]_0$       | $[4]_{\bullet}^2$ |          | 6680 | 668                   |
| 1:        | $[0]_7$           | $[0]_9$       | $[2]_2$           | $4^*$    | 1200 | 120                   |
| 2:        | $[0]_{\circ}$     | $[0]_0$       | $[2]_{\circ}$     | $2^{**}$ | 900  | 90                    |
| 3:        | $[0]_0$           | $[0]_0$       | $[2]_{\bullet}^-$ | $1^{**}$ | 80   | 8                     |
| <hr/>     |                   |               |                   |          |      |                       |
| <b>2:</b> | $[0]_0$           | $[0]_0$       | $[4]_{\bullet}$   |          | 5720 | 578                   |
| 1:        | $[0]_5$           | $[0]_0$       | $[2]_1$           | $2^{**}$ | 504  | 52                    |
| 2:        | $[0]_{\circ}$     | $[0]_0$       | $[2]_{\circ}$     | $2^{**}$ | 540  | 54                    |
| 3:        | $[0]_8$           | $[0]_1$       | $[2]_3$           | $4^*$    | 900  | 90                    |
| 4:        | $[0]_0$           | $[0]_0$       | $[2]_{\bullet}^+$ | $2^{**}$ | 12   | 2                     |
| 5:        | $[0]_0$           | $[0]_0$       | $[2]_{\bullet}^2$ | 1        | 4    | 1                     |
| <hr/>     |                   |               |                   |          |      |                       |
| <b>3:</b> | $[\frac{5}{2}]_5$ | $[0]_0$       | $[\frac{3}{2}]_1$ |          | 4280 | 536                   |
| 1:        | $[2]_{\bullet}$   | $[0]_0$       | $[0]_0$           | 1        | 100  | 20                    |
| 3:        | $[\frac{5}{2}]_5$ | $[0]_0$       | $[\frac{1}{2}]_1$ | 1        | 15   | 3                     |
| 5:        | $[\frac{3}{2}]_5$ | $[0]_0$       | $[\frac{1}{2}]_1$ | 1        | 375  | 75                    |
| 7:        | $[2]_6$           | $[0]_2$       | $[0]_0$           | 2        | 225  | 25                    |
| 9:        | $[\frac{3}{2}]_7$ | $[0]_9$       | $[\frac{1}{2}]_2$ | 2        | 600  | 60                    |
| <hr/>     |                   |               |                   |          |      |                       |
| <b>4:</b> | $[4]_{\bullet}$   | $[0]_0$       | $[0]_0$           |          | 5240 | $542 \rightarrow 530$ |
| 1:        | $[2]_{\bullet}^+$ | $[0]_0$       | $[0]_0$           | $2^*$    | 15   | 3                     |
| 2:        | $[2]_{\bullet}^-$ | $[0]_0$       | $[0]_0$           | $1^{**}$ | 120  | 20                    |
| 3:        | $[2]_5$           | $[0]_0$       | $[0]_1$           | $1^{**}$ | 640  | 60                    |
| 4:        | $[2]_6$           | $[0]_2$       | $[0]_0$           | $2^*$    | 675  | 75                    |
| 5:        | $[2]_7$           | $[0]_9$       | $[0]_2$           | $2^*$    | 720  | $72 \rightarrow 66^*$ |
| 6:        | $[2]_{\circ}$     | $[0]_{\circ}$ | $[0]_0$           | $1^{**}$ | 360  | 36                    |
| 7:        | $[2]_{\circ}$     | $[0]_0$       | $[0]_{\circ}$     | $1^{**}$ | 240  | 24                    |
| 8:        | $[2]_8$           | $[0]_6$       | $[0]_0$           | $2^*$    | 210  | 21                    |
| 9:        | $[2]_8$           | $[0]_1$       | $[0]_3$           | $2^*$    | 320  | 30                    |

|           |                    |                     |                   |          |      |                       |
|-----------|--------------------|---------------------|-------------------|----------|------|-----------------------|
| <b>5:</b> | $[2]_{\circ}$      | $[0]_0$             | $[2]_{\circ}$     |          | 4760 | 506                   |
| 1:        | $[1]_5$            | $[0]_0$             | $[1]_1$           | $1^{**}$ | 560  | 64                    |
| 2:        | $[1]_7$            | $[0]_9$             | $[1]_2$           | $2^*$    | 560  | 56                    |
| 3:        | $[1]_{\circ}^+$    | $[0]_0$             | $[1]_{\circ}$     | $2^*$    | 128  | 16                    |
| 4:        | $[1]_8$            | $[0]_1$             | $[1]_3$           | $2^*$    | 640  | 64                    |
| 5:        | $[1]_9$            | $[0]_3$             | $[1]_2$           | $2^*$    | 240  | 24                    |
| 6:        | $[1]_9$            | $[0]_8$             | $[1]_1$           | $2^*$    | 360  | 40                    |
| 7:        | $[2]_{\bullet}$    | $[0]_0$             | $[0]_0$           | 1        | 56   | 7                     |
| 9:        | $[2]_{\circ}$      | $[0]_{\circ}$       | $[0]_0$           | 1        | 90   | 9                     |
| 11:       | $[2]_{\circ}$      | $[0]_0$             | $[0]_{\circ}^+$   | 1        | 24   | 4                     |
| 13:       | $[2]_{\circ}$      | $[0]_0$             | $[0]_{\circ}^-$   | 1        | 2    | 1                     |
| <b>6:</b> | $[\frac{8}{5}]_8$  | $[\frac{12}{5}]_6$  | $[0]_0$           |          | 4280 | $548 \rightarrow 498$ |
| 1:        | $[\frac{4}{5}]_4$  | $[\frac{6}{5}]_8$   | $[0]_0$           | $1^{**}$ | 420  | 48                    |
| 2:        | $[\frac{4}{5}]_9$  | $[\frac{6}{5}]_3$   | $[0]_2$           | $1^{**}$ | 480  | $72 \rightarrow 46^*$ |
| 3:        | $[\frac{4}{5}]_9$  | $[\frac{6}{5}]_8$   | $[0]_1$           | $1^{**}$ | 384  | 36                    |
| 4:        | $[2]_{\bullet}$    | $[0]_0$             | $[0]_0$           | 1        | 28   | 4                     |
| 6:        | $[\frac{6}{5}]_6$  | $[\frac{4}{5}]_2$   | $[0]_0$           | 1        | 420  | 60                    |
| 8:        | $[\frac{7}{5}]_7$  | $[\frac{3}{5}]_9$   | $[0]_2$           | 1        | 384  | $48 \rightarrow 36^*$ |
| 10:       | $[1]_{\circ}$      | $[1]_{\circ}$       | $[0]_0$           | 1        | 384  | 48                    |
| 12:       | $[\frac{8}{5}]_8$  | $[\frac{2}{5}]_6$   | $[0]_0$           | 1        | 90   | 18                    |
| 14:       | $[\frac{8}{5}]_8$  | $[\frac{2}{5}]_1$   | $[0]_3$           | 1        | 192  | 18                    |
| <b>7:</b> | $[\frac{9}{10}]_9$ | $[\frac{21}{10}]_3$ | $[1]_2$           |          | 4280 | $502 \rightarrow 490$ |
| 1:        | $[\frac{3}{5}]_6$  | $[\frac{7}{5}]_2$   | $[0]_0$           | 1        | 252  | 27                    |
| 3:        | $[\frac{7}{10}]_7$ | $[\frac{3}{10}]_9$  | $[1]_2$           | 1        | 252  | 28                    |
| 5:        | $[1]_{\circ}$      | $[1]_{\circ}$       | $[0]_0$           | 1        | 189  | 21                    |
| 7:        | $[1]_{\circ}$      | $[0]_0$             | $[1]_{\circ}$     | 1        | 90   | 10                    |
| 9:        | $[\frac{4}{5}]_8$  | $[\frac{6}{5}]_6$   | $[0]_0$           | 1        | 315  | 35                    |
| 11:       | $[\frac{4}{5}]_8$  | $[\frac{7}{10}]_1$  | $[\frac{1}{2}]_3$ | 1        | 432  | 48                    |
| 13:       | $[\frac{9}{10}]_9$ | $[\frac{21}{10}]_3$ | $[-1]_2$          | 1        | 1    | 1                     |
| 15:       | $[\frac{9}{10}]_9$ | $[\frac{11}{10}]_3$ | $[0]_2$           | 1        | 210  | $30 \rightarrow 24^*$ |
| 17:       | $[\frac{9}{10}]_9$ | $[\frac{1}{10}]_3$  | $[1]_2$           | 1        | 63   | 9                     |
| 19:       | $[\frac{9}{10}]_9$ | $[\frac{3}{5}]_8$   | $[\frac{1}{2}]_1$ | 1        | 336  | 42                    |
| <b>8:</b> | $[2]_{\circ}$      | $[2]_{\circ}$       | $[0]_0$           |          | 4760 | $552 \rightarrow 488$ |
| 1:        | $[1]_6$            | $[1]_2$             | $[0]_0$           | $4^*$    | 448  | 48                    |
| 2:        | $[1]_7$            | $[1]_9$             | $[0]_2$           | $4^*$    | 336  | $48 \rightarrow 32^*$ |
| 3:        | $[2]_{\circ}$      | $[0]_0$             | $[0]_{\circ}$     | $2^*$    | 60   | 6                     |

|           |                    |                   |                   |         |      |     |
|-----------|--------------------|-------------------|-------------------|---------|------|-----|
| 4:        | $[1]_{\circ}^{+}$  | $[1]_{\circ}^{+}$ | $[0]_0$           | $4^{*}$ | 64   | 8   |
| 5:        | $[1]_8$            | $[1]_1$           | $[0]_3$           | $4^{*}$ | 256  | 24  |
| 6:        | $[2]_{\bullet}$    | $[0]_0$           | $[0]_0$           | 2       | 56   | 7   |
| <hr/>     |                    |                   |                   |         |      |     |
| <b>9:</b> | $[\frac{9}{10}]_9$ | $[\frac{8}{5}]_8$ | $[\frac{3}{2}]_1$ |         | 4280 | 482 |
| 1:        | $[\frac{1}{2}]_5$  | $[0]_0$           | $[\frac{3}{2}]_1$ | 1       | 126  | 13  |
| 3:        | $[\frac{7}{10}]_7$ | $[\frac{4}{5}]_9$ | $[\frac{1}{2}]_2$ | 1       | 432  | 48  |
| 5:        | $[1]_{\circ}$      | $[1]_{\circ}$     | $[0]_0$           | 1       | 144  | 16  |
| 7:        | $[1]_{\circ}$      | $[0]_0$           | $[1]_{\circ}$     | 1       | 135  | 15  |
| 9:        | $[\frac{4}{5}]_8$  | $[\frac{6}{5}]_6$ | $[0]_0$           | 1       | 252  | 28  |
| 11:       | $[\frac{4}{5}]_8$  | $[\frac{1}{5}]_1$ | $[1]_3$           | 1       | 432  | 48  |
| 13:       | $[\frac{9}{10}]_9$ | $[\frac{3}{5}]_3$ | $[\frac{1}{2}]_2$ | 1       | 336  | 36  |
| 15:       | $[\frac{9}{10}]_9$ | $[\frac{8}{5}]_8$ | $[\frac{1}{2}]_1$ | 1       | 15   | 3   |
| 17:       | $[\frac{9}{10}]_9$ | $[\frac{3}{5}]_8$ | $[\frac{1}{2}]_1$ | 1       | 240  | 30  |
| 19:       | $[\frac{9}{10}]_9$ | $[\frac{2}{5}]_8$ | $[\frac{3}{2}]_1$ | 1       | 28   | 4   |

2.13. **The lattice  $N(3A_8)$ .** There are 5 classes;  $b(\mathfrak{O}) \leq 588$ .

|           |                     |                    |                    |          |      |     |
|-----------|---------------------|--------------------|--------------------|----------|------|-----|
| <b>1:</b> | $[4]_{\bullet}$     | $[0]_0$            | $[0]_0$            |          | 5272 | 588 |
| 1:        | $[2]_{\bullet}^{+}$ | $[0]_0$            | $[0]_0$            | $2^{*}$  | 10   | 2   |
| 2:        | $[2]_{\bullet}^{-}$ | $[0]_0$            | $[0]_0$            | $1^{**}$ | 80   | 16  |
| 3:        | $[2]_5$             | $[0]_8$            | $[0]_8$            | $2^{*}$  | 810  | 90  |
| 4:        | $[2]_6$             | $[0]_3$            | $[0]_0$            | $4^{*}$  | 420  | 45  |
| 5:        | $[2]_{\circ}$       | $[0]_{\circ}$      | $[0]_0$            | $2^{**}$ | 288  | 32  |
| 6:        | $[2]_7$             | $[0]_7$            | $[0]_1$            | $4^{*}$  | 324  | 36  |
| <hr/>     |                     |                    |                    |          |      |     |
| <b>2:</b> | $[\frac{8}{9}]_8$   | $[\frac{14}{9}]_2$ | $[\frac{14}{9}]_2$ |          | 4312 | 576 |
| 1:        | $[\frac{4}{9}]_4$   | $[\frac{7}{9}]_1$  | $[\frac{7}{9}]_1$  | $1^{**}$ | 280  | 32  |
| 2:        | $[1]_{\circ}$       | $[1]_{\circ}$      | $[0]_0$            | 2        | 112  | 14  |
| 4:        | $[\frac{2}{3}]_6$   | $[\frac{4}{3}]_3$  | $[0]_0$            | 2        | 196  | 28  |
| 6:        | $[\frac{7}{9}]_7$   | $[\frac{4}{9}]_7$  | $[\frac{7}{9}]_1$  | 2        | 336  | 42  |
| 8:        | $[\frac{8}{9}]_8$   | $[\frac{8}{9}]_5$  | $[\frac{2}{9}]_8$  | 2        | 245  | 35  |
| 10:       | $[\frac{8}{9}]_8$   | $[\frac{14}{9}]_2$ | $[\frac{4}{9}]_2$  | 2        | 21   | 3   |
| 12:       | $[\frac{8}{9}]_8$   | $[\frac{5}{9}]_2$  | $[\frac{5}{9}]_2$  | 1        | 196  | 28  |
| <hr/>     |                     |                    |                    |          |      |     |
| <b>3:</b> | $[2]_{\circ}$       | $[2]_{\circ}$      | $[0]_0$            |          | 4792 | 570 |
| 1:        | $[1]_5$             | $[1]_8$            | $[0]_8$            | $4^{*}$  | 315  | 35  |
| 2:        | $[2]_{\circ}$       | $[0]_0$            | $[0]_{\circ}$      | $2^{*}$  | 72   | 8   |
| 3:        | $[1]_6$             | $[1]_3$            | $[0]_0$            | $2^{*}$  | 441  | 63  |
| 4:        | $[1]_{\circ}^{+}$   | $[1]_{\circ}^{+}$  | $[0]_0$            | $2^{*}$  | 49   | 7   |

|       |                   |                   |                    |     |      |     |
|-------|-------------------|-------------------|--------------------|-----|------|-----|
| 5:    | $[1]_{\circ}^{+}$ | $[1]_{\circ}^{-}$ | $[0]_0$            | 2*  | 49   | 7   |
| 6:    | $[1]_7$           | $[1]_7$           | $[0]_1$            | 2*  | 441  | 49  |
| 7:    | $[1]_7$           | $[1]_1$           | $[0]_7$            | 4*  | 252  | 28  |
| 8:    | $[1]_8$           | $[1]_8$           | $[0]_5$            | 2*  | 126  | 13  |
| 9:    | $[2]_{\bullet}$   | $[0]_0$           | $[0]_0$            | 2   | 42   | 6   |
| <hr/> |                   |                   |                    |     |      |     |
| 4:    | $[\frac{8}{9}]_8$ | $[\frac{8}{9}]_8$ | $[\frac{20}{9}]_5$ |     | 4312 | 552 |
| 1:    | $[\frac{7}{9}]_7$ | $[\frac{1}{9}]_1$ | $[\frac{10}{9}]_7$ | 2*  | 384  | 48  |
| 2:    | $[\frac{5}{9}]_5$ | $[\frac{8}{9}]_8$ | $[\frac{5}{9}]_8$  | 2   | 224  | 24  |
| 4:    | $[1]_{\circ}$     | $[1]_{\circ}$     | $[0]_0$            | 1   | 64   | 8   |
| 6:    | $[1]_{\circ}$     | $[0]_0$           | $[1]_{\circ}$      | 2   | 160  | 20  |
| 8:    | $[\frac{2}{3}]_6$ | $[0]_0$           | $[\frac{4}{3}]_3$  | 2   | 280  | 40  |
| 10:   | $[\frac{7}{9}]_7$ | $[\frac{7}{9}]_7$ | $[\frac{4}{9}]_1$  | 1   | 320  | 40  |
| 12:   | $[\frac{8}{9}]_8$ | $[\frac{8}{9}]_8$ | $[\frac{2}{9}]_5$  | 1   | 60   | 12  |
| <hr/> |                   |                   |                    |     |      |     |
| 5:    | $[2]_6$           | $[2]_3$           | $[0]_0$            |     | 4312 | 546 |
| 1:    | $[\frac{5}{3}]_5$ | $[\frac{1}{3}]_8$ | $[0]_8$            | 2*  | 324  | 36  |
| 2:    | $[2]_6$           | $[0]_0$           | $[0]_3$            | 2*  | 84   | 9   |
| 3:    | $[1]_3$           | $[1]_6$           | $[0]_0$            | 1** | 400  | 60  |
| 4:    | $[\frac{4}{3}]_7$ | $[\frac{2}{3}]_1$ | $[0]_7$            | 2*  | 324  | 36  |
| 5:    | $[2]_{\bullet}$   | $[0]_0$           | $[0]_0$            | 2   | 45   | 9   |
| 7:    | $[\frac{4}{3}]_4$ | $[\frac{2}{3}]_1$ | $[0]_1$            | 2   | 405  | 45  |
| 9:    | $[1]_6$           | $[1]_3$           | $[0]_0$            | 1   | 324  | 54  |

2.14. **The lattice  $N(3\mathbf{D}_8)$ .** There are 5 classes;  $b(\mathfrak{O}) \leq 498$ .

|       |                   |                   |               |     |      |                        |
|-------|-------------------|-------------------|---------------|-----|------|------------------------|
| 1:    | $[4]_{\bullet}^2$ | $[0]_0$           | $[0]_0$       |     | 7512 | 498                    |
| 1:    | $[2]_{\bullet}$   | $[0]_0$           | $[0]_0$       | 1** | 280  | 18                     |
| 2:    | $[2]_{\circ}$     | $[0]_{\circ}$     | $[0]_0$       | 2** | 1568 | 112                    |
| 3:    | $[2]_2$           | $[0]_1$           | $[0]_2$       | 2** | 2048 | 128                    |
| <hr/> |                   |                   |               |     |      |                        |
| 2:    | $[2]_3$           | $[2]_3$           | $[0]_0$       |     | 4152 | 528 $\rightarrow$ 416  |
| 1:    | $[2]_3$           | $[0]_0$           | $[0]_3$       | 2*  | 128  | 8                      |
| 2:    | $[\frac{3}{2}]_1$ | $[\frac{1}{2}]_2$ | $[0]_2$       | 2*  | 1024 | 128 $\rightarrow$ 72 * |
| 3:    | $[2]_{\bullet}$   | $[0]_0$           | $[0]_0$       | 2   | 70   | 8                      |
| 5:    | $[1]_3$           | $[1]_3$           | $[0]_0$       | 1   | 784  | 112                    |
| <hr/> |                   |                   |               |     |      |                        |
| 3:    | $[2]_{\circ}$     | $[2]_{\circ}$     | $[0]_0$       |     | 4632 | 436 $\rightarrow$ 384  |
| 1:    | $[2]_{\circ}$     | $[0]_0$           | $[0]_{\circ}$ | 2*  | 112  | 8                      |
| 2:    | $[1]_3$           | $[1]_3$           | $[0]_0$       | 1** | 1024 | 96                     |
| 3:    | $[1]_1$           | $[1]_2$           | $[0]_2$       | 2** | 1024 | 96 $\rightarrow$ 70 *  |

|       |                   |               |                   |          |      |                         |
|-------|-------------------|---------------|-------------------|----------|------|-------------------------|
| 4:    | $[1]_{\circ}$     | $[1]_{\circ}$ | $[0]_0$           | $1^{**}$ | 576  | 72                      |
| 5:    | $[1]_2$           | $[1]_2$       | $[0]_1$           | $1^{**}$ | 512  | 32                      |
| 6:    | $[2]_{\bullet}$   | $[0]_0$       | $[0]_0$           | 2        | 60   | 6                       |
| 8:    | $[2]_{\bullet}^2$ | $[0]_0$       | $[0]_0$           | 2        | 2    | 1                       |
| <hr/> |                   |               |                   |          |      |                         |
| 4:    | $[4]_{\bullet}$   | $[0]_0$       | $[0]_0$           |          | 5592 | $498 \rightarrow 380$   |
| 1:    | $[2]_{\bullet}^+$ | $[0]_0$       | $[0]_0$           | $1^{**}$ | 144  | 16                      |
| 2:    | $[2]_3$           | $[0]_3$       | $[0]_0$           | $2^{**}$ | 1024 | 64                      |
| 3:    | $[2]_1$           | $[0]_2$       | $[0]_2$           | $1^{**}$ | 2048 | $256 \rightarrow 138 *$ |
| 4:    | $[2]_{\circ}$     | $[0]_{\circ}$ | $[0]_0$           | $2^{**}$ | 672  | 48                      |
| 5:    | $[2]_{\bullet}^2$ | $[0]_0$       | $[0]_0$           | 1        | 4    | 1                       |
| <hr/> |                   |               |                   |          |      |                         |
| 5:    | $[1]_2$           | $[1]_2$       | $[2]_1$           |          | 4152 | $460 \rightarrow 340$   |
| 1:    | $[2]_{\bullet}^2$ | $[0]_0$       | $[0]_0$           | 2        | 1    | 1                       |
| 3:    | $[1]_{\circ}$     | $[1]_{\circ}$ | $[0]_0$           | 1        | 196  | $28 \rightarrow 16 *$   |
| 5:    | $[1]_{\circ}$     | $[0]_0$       | $[1]_{\circ}$     | 2        | 392  | $56 \rightarrow 32 *$   |
| 7:    | $[\frac{1}{2}]_3$ | $[0]_0$       | $[\frac{3}{2}]_3$ | 2        | 512  | 40                      |
| 9:    | $[1]_2$           | $[1]_2$       | $[0]_1$           | 1        | 70   | 8                       |

2.15. **The lattice  $N(4\mathbf{D}_6)$ .** There are 5 classes;  $b(\mathfrak{O}) \leq 634$ .

|       |                   |                   |                   |         |          |      |                         |
|-------|-------------------|-------------------|-------------------|---------|----------|------|-------------------------|
| 1:    | $[4]_{\bullet}^2$ | $[0]_0$           | $[0]_0$           | $[0]_0$ |          | 6680 | $764 \rightarrow 634$   |
| 1:    | $[2]_{\bullet}^-$ | $[0]_0$           | $[0]_0$           | $[0]_0$ | $1^{**}$ | 80   | 8                       |
| 2:    | $[2]_{\circ}$     | $[0]_{\circ}$     | $[0]_0$           | $[0]_0$ | $3^{**}$ | 600  | 60                      |
| 3:    | $[2]_2$           | $[0]_3$           | $[0]_0$           | $[0]_1$ | $3^{**}$ | 1024 | 96                      |
| 4:    | $[2]_2$           | $[0]_2$           | $[0]_2$           | $[0]_2$ | $1^{**}$ | 1728 | $288 \rightarrow 158 *$ |
| <hr/> |                   |                   |                   |         |          |      |                         |
| 2:    | $[1]_2$           | $[1]_2$           | $[1]_2$           | $[1]_2$ |          | 4280 | $632 \rightarrow 536$   |
| 1:    | $[\frac{1}{2}]_3$ | $[\frac{1}{2}]_1$ | $[0]_0$           | $[1]_2$ | $12^*$   | 256  | 32                      |
| 2:    | $[2]_{\bullet}^2$ | $[0]_0$           | $[0]_0$           | $[0]_0$ | 4        | 1    | 1                       |
| 4:    | $[1]_{\circ}$     | $[1]_{\circ}$     | $[0]_0$           | $[0]_0$ | 6        | 100  | $20 \rightarrow 12 *$   |
| <hr/> |                   |                   |                   |         |          |      |                         |
| 3:    | $[4]_{\bullet}$   | $[0]_0$           | $[0]_0$           | $[0]_0$ |          | 5720 | $546 \rightarrow 534$   |
| 1:    | $[2]_{\bullet}^+$ | $[0]_0$           | $[0]_0$           | $[0]_0$ | $2^{**}$ | 12   | 2                       |
| 2:    | $[2]_{\circ}$     | $[0]_{\circ}$     | $[0]_0$           | $[0]_0$ | $3^{**}$ | 360  | 36                      |
| 3:    | $[2]_3$           | $[0]_1$           | $[0]_0$           | $[0]_2$ | $6^{**}$ | 768  | $72 \rightarrow 70 *$   |
| 4:    | $[2]_{\bullet}^2$ | $[0]_0$           | $[0]_0$           | $[0]_0$ | 1        | 4    | 1                       |
| <hr/> |                   |                   |                   |         |          |      |                         |
| 4:    | $[\frac{3}{2}]_3$ | $[1]_2$           | $[\frac{3}{2}]_1$ | $[0]_0$ |          | 4280 | $632 \rightarrow 512$   |
| 1:    | $[\frac{3}{2}]_3$ | $[\frac{1}{2}]_1$ | $[0]_0$           | $[0]_2$ | $2^*$    | 192  | $24 \rightarrow 18 *$   |
| 2:    | $[1]_1$           | $[\frac{1}{2}]_3$ | $[\frac{1}{2}]_2$ | $[0]_0$ | $2^*$    | 576  | 72                      |
| 3:    | $[2]_{\bullet}$   | $[0]_0$           | $[0]_0$           | $[0]_0$ | 2        | 15   | 3                       |

|           |                   |               |                   |         |          |      |                        |
|-----------|-------------------|---------------|-------------------|---------|----------|------|------------------------|
| 5:        | $[1]_{\circ}$     | $[1]_{\circ}$ | $[0]_0$           | $[0]_0$ | 2        | 150  | $30 \rightarrow 18$ *  |
| 7:        | $[1]_{\circ}$     | $[0]_0$       | $[1]_{\circ}$     | $[0]_0$ | 1        | 225  | 45                     |
| 9:        | $[\frac{3}{2}]_3$ | $[-1]_2$      | $[\frac{3}{2}]_1$ | $[0]_0$ | 1        | 1    | 1                      |
| 11:       | $[\frac{3}{2}]_3$ | $[0]_0$       | $[\frac{1}{2}]_2$ | $[0]_1$ | 2        | 192  | 18                     |
| 13:       | $[1]_1$           | $[0]_0$       | $[1]_3$           | $[0]_2$ | 1        | 432  | $72 \rightarrow 42$ *  |
| <hr/>     |                   |               |                   |         |          |      |                        |
| <b>5:</b> | $[2]_{\circ}$     | $[2]_{\circ}$ | $[0]_0$           | $[0]_0$ |          | 4760 | $636 \rightarrow 498$  |
| 1:        | $[2]_{\circ}$     | $[0]_0$       | $[0]_{\circ}$     | $[0]_0$ | $4^*$    | 60   | 6                      |
| 2:        | $[1]_{\circ}$     | $[1]_{\circ}$ | $[0]_0$           | $[0]_0$ | $1^{**}$ | 256  | 48                     |
| 3:        | $[1]_3$           | $[1]_1$       | $[0]_0$           | $[0]_2$ | $2^{**}$ | 768  | $128 \rightarrow 80$ * |
| 4:        | $[1]_3$           | $[1]_2$       | $[0]_1$           | $[0]_0$ | $4^{**}$ | 512  | 48                     |
| 5:        | $[1]_2$           | $[1]_2$       | $[0]_2$           | $[0]_2$ | $1^{**}$ | 576  | $96 \rightarrow 54$ *  |
| 6:        | $[2]_{\bullet}$   | $[0]_0$       | $[0]_0$           | $[0]_0$ | 2        | 24   | 4                      |
| 8:        | $[2]_{\bullet}^2$ | $[0]_0$       | $[0]_0$           | $[0]_0$ | 2        | 2    | 1                      |

## 3. SUFFICIENT ESTIMATES ON COMBINATORIAL ORBITS

For three lattices, the naïve combinatorial estimates of [\\*\\*§3](#) do not suffice to establish the inequality  $b(\mathfrak{D}_h) < 720$ , and we need to compute (some of) the bounds  $b(\mathfrak{o})$  by brute force [§1.4](#). After each table, for each offending vector  $h$ , we indicate the choice of the parameters (in the notation of [§1.4](#)) used in the computation. These parameters are encoded in the function

$$(3.1) \quad 4\_ \langle \text{lattice name} \rangle\_h\_ \text{auto}() \quad \text{defined in the file "4RS.txt",}$$

$h$  referring to the index of the pair  $N \ni h$  in the tables.

Together with the previous section, these data constitute the proof of [\\*\\*Theorem 4.1](#).

3.1. **The lattice  $N(2\mathbf{A}_7 \oplus 2\mathbf{D}_5)$ .** There are 12 classes;  $b(\mathfrak{D}) \leq 702$ .

|           |                   |         |                   |                   |         |                              |
|-----------|-------------------|---------|-------------------|-------------------|---------|------------------------------|
| <b>1:</b> | $[0]_0$           | $[0]_0$ | $[4]_{\bullet}^2$ | $[0]_0$           | 6264    | 796 $\rightarrow$ 702        |
| 1:        | $[0]_4$           | $[0]_0$ | $[2]_2$           | $[0]_2$           | 2** 700 | 80 $\rightarrow$ <u>64</u> ✓ |
| 2:        | $[0]_{\circ}$     | $[0]_0$ | $[2]_{\circ}$     | $[0]_0$           | 2** 448 | 56 $\rightarrow$ <u>44</u> ✓ |
| 3:        | $[0]_6$           | $[0]_6$ | $[2]_2$           | $[0]_0$           | 2* 784  | 112                          |
| 4:        | $[0]_7$           | $[0]_1$ | $[2]_2$           | $[0]_3$           | 2* 1024 | 128 $\rightarrow$ 113 ‡      |
| 5:        | $[0]_0$           | $[0]_0$ | $[2]_{\bullet}^-$ | $[0]_0$           | 1** 32  | 4                            |
| 6:        | $[0]_0$           | $[0]_0$ | $[2]_{\circ}$     | $[0]_{\circ}$     | 1** 320 | 40 $\rightarrow$ <u>32</u> ✓ |
| <b>2:</b> | $[2]_4$           | $[0]_0$ | $[1]_2$           | $[1]_2$           | 4344    | 740 $\rightarrow$ 680        |
| 1:        | $[1]_6$           | $[0]_6$ | $[1]_2$           | $[0]_0$           | 4* 168  | 24                           |
| 2:        | $[1]_6$           | $[0]_0$ | $[\frac{1}{2}]_1$ | $[\frac{1}{2}]_1$ | 2** 384 | 96                           |
| 3:        | $[2]_{\bullet}$   | $[0]_0$ | $[0]_0$           | $[0]_0$           | 1 36    | 8                            |
| 5:        | $[2]_4$           | $[0]_4$ | $[0]_0$           | $[0]_0$           | 1 70    | 8                            |
| 7:        | $[2]_4$           | $[0]_0$ | $[1]_2$           | $[-1]_2$          | 2 1     | 1                            |
| 9:        | $[2]_4$           | $[0]_0$ | $[0]_2$           | $[0]_2$           | 1 64    | 16 $\rightarrow$ 10 *        |
| 11:       | $[1]_4$           | $[0]_0$ | $[1]_2$           | $[0]_2$           | 2 128   | 32 $\rightarrow$ 20 *        |
| 13:       | $[\frac{3}{2}]_5$ | $[0]_7$ | $[0]_0$           | $[\frac{1}{2}]_3$ | 4 256   | 32                           |
| <b>3:</b> | $[0]_0$           | $[0]_0$ | $[4]_{\bullet}$   | $[0]_0$           | 5784    | 692 $\rightarrow$ 676        |
| 1:        | $[0]_{\circ}$     | $[0]_0$ | $[2]_{\circ}$     | $[0]_0$           | 2** 336 | 42                           |
| 2:        | $[0]_5$           | $[0]_1$ | $[2]_3$           | $[0]_0$           | 4* 448  | 48                           |
| 3:        | $[0]_6$           | $[0]_0$ | $[2]_1$           | $[0]_1$           | 4* 448  | 56                           |
| 4:        | $[0]_7$           | $[0]_7$ | $[2]_3$           | $[0]_2$           | 2* 640  | 80 $\rightarrow$ 72 *        |
| 5:        | $[0]_0$           | $[0]_0$ | $[2]_{\circ}$     | $[0]_{\circ}$     | 1** 240 | 30                           |
| 6:        | $[0]_0$           | $[0]_0$ | $[2]_{\bullet}$   | $[0]_0$           | 1 4     | 1                            |
| <b>4:</b> | $[0]_0$           | $[0]_0$ | $[2]_{\circ}$     | $[2]_{\circ}$     | 4824    | 656                          |
| 1:        | $[0]_4$           | $[0]_0$ | $[1]_2$           | $[1]_2$           | 2** 280 | 32                           |
| 2:        | $[0]_{\circ}$     | $[0]_0$ | $[2]_{\circ}$     | $[0]_0$           | 4* 56   | 7                            |
| 3:        | $[0]_6$           | $[0]_0$ | $[1]_1$           | $[1]_1$           | 4* 448  | 64                           |
| 4:        | $[0]_7$           | $[0]_7$ | $[1]_3$           | $[1]_2$           | 4* 512  | 64                           |

|           |                   |                   |                   |                   |     |      |                        |
|-----------|-------------------|-------------------|-------------------|-------------------|-----|------|------------------------|
| 5:        | $[0]_0$           | $[0]_0$           | $[1]_0$           | $[1]_0$           | 1** | 144  | 36                     |
| 6:        | $[0]_0$           | $[0]_0$           | $[2]_\bullet$     | $[0]_0$           | 2   | 12   | 3                      |
| 8:        | $[0]_0$           | $[0]_0$           | $[2]_\bullet^2$   | $[0]_0$           | 2   | 2    | 1                      |
| <hr/>     |                   |                   |                   |                   |     |      |                        |
| <b>5:</b> | $[4]_\bullet$     | $[0]_0$           | $[0]_0$           | $[0]_0$           |     | 5304 | 730 $\rightarrow$ 646  |
| 1:        | $[2]_\bullet^+$   | $[0]_0$           | $[0]_0$           | $[0]_0$           | 2*  | 6    | 2                      |
| 2:        | $[2]_\bullet^-$   | $[0]_0$           | $[0]_0$           | $[0]_0$           | 1** | 48   | 10                     |
| 3:        | $[2]_4$           | $[0]_4$           | $[0]_0$           | $[0]_0$           | 1** | 420  | 48                     |
| 4:        | $[2]_4$           | $[0]_0$           | $[0]_2$           | $[0]_2$           | 1** | 600  | 120 $\rightarrow$ 68 * |
| 5:        | $[2]_0$           | $[0]_0$           | $[0]_0$           | $[0]_0$           | 1** | 224  | 28                     |
| 6:        | $[2]_0$           | $[0]_0$           | $[0]_0$           | $[0]_0$           | 2** | 160  | 20                     |
| 7:        | $[2]_5$           | $[0]_7$           | $[0]_0$           | $[0]_3$           | 4*  | 512  | 64                     |
| 8:        | $[2]_6$           | $[0]_6$           | $[0]_2$           | $[0]_0$           | 4*  | 280  | 40 $\rightarrow$ 32 *  |
| 9:        | $[2]_6$           | $[0]_0$           | $[0]_1$           | $[0]_1$           | 2*  | 256  | 32                     |
| <hr/>     |                   |                   |                   |                   |     |      |                        |
| <b>6:</b> | $[\frac{3}{2}]_6$ | $[0]_0$           | $[\frac{5}{4}]_1$ | $[\frac{5}{4}]_1$ |     | 4344 | 644                    |
| 1:        | $[\frac{3}{4}]_3$ | $[0]_7$           | $[\frac{5}{4}]_1$ | $[0]_0$           | 2*  | 160  | 20                     |
| 2:        | $[\frac{3}{4}]_7$ | $[0]_5$           | $[0]_0$           | $[\frac{5}{4}]_1$ | 2*  | 112  | 12                     |
| 3:        | $[\frac{3}{4}]_7$ | $[0]_7$           | $[\frac{3}{4}]_3$ | $[\frac{1}{2}]_2$ | 2*  | 400  | 50                     |
| 4:        | $[2]_\bullet$     | $[0]_0$           | $[0]_0$           | $[0]_0$           | 1   | 15   | 3                      |
| 6:        | $[1]_4$           | $[0]_0$           | $[\frac{1}{2}]_2$ | $[\frac{1}{2}]_2$ | 1   | 375  | 75                     |
| 8:        | $[1]_0$           | $[0]_0$           | $[1]_0$           | $[0]_0$           | 2   | 120  | 20                     |
| 10:       | $[\frac{5}{4}]_5$ | $[0]_7$           | $[0]_0$           | $[\frac{3}{4}]_3$ | 2   | 240  | 30                     |
| 12:       | $[\frac{3}{2}]_6$ | $[0]_6$           | $[\frac{1}{2}]_2$ | $[0]_0$           | 2   | 140  | 20                     |
| 14:       | $[\frac{3}{2}]_6$ | $[0]_0$           | $[\frac{5}{4}]_1$ | $[\frac{3}{4}]_1$ | 2   | 5    | 1                      |
| 16:       | $[\frac{3}{2}]_6$ | $[0]_0$           | $[\frac{1}{4}]_1$ | $[\frac{1}{4}]_1$ | 1   | 100  | 20                     |
| <hr/>     |                   |                   |                   |                   |     |      |                        |
| <b>7:</b> | $[\frac{3}{2}]_6$ | $[\frac{3}{2}]_6$ | $[1]_2$           | $[0]_0$           |     | 4344 | 720 $\rightarrow$ 640  |
| 1:        | $[\frac{5}{4}]_5$ | $[\frac{1}{4}]_1$ | $[\frac{1}{2}]_3$ | $[0]_0$           | 2*  | 288  | 48                     |
| 2:        | $[\frac{3}{4}]_3$ | $[\frac{3}{4}]_7$ | $[\frac{1}{2}]_1$ | $[0]_0$           | 2** | 320  | 48                     |
| 3:        | $[\frac{3}{2}]_6$ | $[0]_0$           | $[\frac{1}{2}]_1$ | $[0]_1$           | 2*  | 128  | 16                     |
| 4:        | $[\frac{3}{4}]_7$ | $[\frac{3}{4}]_7$ | $[\frac{1}{2}]_3$ | $[0]_2$           | 1** | 320  | 64 $\rightarrow$ 40 *  |
| 5:        | $[2]_\bullet$     | $[0]_0$           | $[0]_0$           | $[0]_0$           | 2   | 15   | 3                      |
| 7:        | $[1]_4$           | $[1]_4$           | $[0]_0$           | $[0]_0$           | 1   | 225  | 45                     |
| 9:        | $[1]_4$           | $[0]_0$           | $[1]_2$           | $[0]_2$           | 2   | 150  | 30 $\rightarrow$ 18 *  |
| 11:       | $[1]_0$           | $[1]_0$           | $[0]_0$           | $[0]_0$           | 1   | 144  | 24                     |
| 13:       | $[1]_0$           | $[0]_0$           | $[1]_0$           | $[0]_0$           | 2   | 96   | 16 $\rightarrow$ 14 *  |
| 15:       | $[\frac{5}{4}]_5$ | $[\frac{3}{4}]_7$ | $[0]_0$           | $[0]_3$           | 2   | 192  | 24                     |
| 17:       | $[\frac{3}{2}]_6$ | $[\frac{3}{2}]_6$ | $[-1]_2$          | $[0]_0$           | 1   | 1    | 1                      |



|       |                   |                   |                   |                   |         |                       |
|-------|-------------------|-------------------|-------------------|-------------------|---------|-----------------------|
| 8:    | $[2]_4$           | $[2]_4$           | $[0]_0$           | $[0]_0$           | 4344    | 744 $\rightarrow$ 632 |
| 1:    | $[2]_4$           | $[0]_0$           | $[0]_2$           | $[0]_2$           | 2* 100  | 20 $\rightarrow$ 12 * |
| 2:    | $[\frac{3}{2}]_5$ | $[\frac{1}{2}]_7$ | $[0]_0$           | $[0]_3$           | 8* 256  | 32                    |
| 3:    | $[1]_6$           | $[1]_6$           | $[0]_2$           | $[0]_0$           | 4** 360 | 72 $\rightarrow$ 48 * |
| 4:    | $[2]_\bullet$     | $[0]_0$           | $[0]_0$           | $[0]_0$           | 2 36    | 8                     |
| 6:    | $[1]_4$           | $[1]_4$           | $[0]_0$           | $[0]_0$           | 1 256   | 64                    |
| <hr/> |                   |                   |                   |                   |         |                       |
| 9:    | $[\frac{7}{8}]_7$ | $[\frac{7}{8}]_7$ | $[\frac{5}{4}]_3$ | $[1]_2$           | 4344    | 632 $\rightarrow$ 624 |
| 1:    | $[1]_\circ$       | $[1]_\circ$       | $[0]_0$           | $[0]_0$           | 1 49    | 7                     |
| 3:    | $[1]_\circ$       | $[0]_0$           | $[1]_\circ$       | $[0]_0$           | 2 70    | 10                    |
| 5:    | $[1]_\circ$       | $[0]_0$           | $[0]_0$           | $[1]_\circ$       | 2 56    | 8                     |
| 7:    | $[\frac{1}{2}]_4$ | $[0]_0$           | $[\frac{1}{2}]_2$ | $[1]_2$           | 2 175   | 25                    |
| 9:    | $[\frac{5}{8}]_5$ | $[\frac{7}{8}]_7$ | $[0]_0$           | $[\frac{1}{2}]_3$ | 2 168   | 24                    |
| 11:   | $[\frac{5}{8}]_5$ | $[\frac{1}{8}]_1$ | $[\frac{5}{4}]_3$ | $[0]_0$           | 2 147   | 21                    |
| 13:   | $[\frac{3}{4}]_6$ | $[\frac{3}{4}]_6$ | $[\frac{1}{2}]_2$ | $[0]_0$           | 1 245   | 35                    |
| 15:   | $[\frac{3}{4}]_6$ | $[0]_0$           | $[\frac{3}{4}]_1$ | $[\frac{1}{2}]_1$ | 2 280   | 40                    |
| 17:   | $[\frac{7}{8}]_7$ | $[\frac{7}{8}]_7$ | $[\frac{5}{4}]_3$ | $[-1]_2$          | 1 1     | 1                     |
| 19:   | $[\frac{7}{8}]_7$ | $[\frac{7}{8}]_7$ | $[\frac{1}{4}]_3$ | $[0]_2$           | 1 80    | 16 $\rightarrow$ 12 * |
| 21:   | $[\frac{7}{8}]_7$ | $[\frac{7}{8}]_7$ | $[\frac{3}{4}]_3$ | $[1]_2$           | 1 5     | 1                     |
| <hr/> |                   |                   |                   |                   |         |                       |
| 10:   | $[2]_\circ$       | $[0]_0$           | $[2]_\circ$       | $[0]_0$           | 4824    | 630 $\rightarrow$ 608 |
| 1:    | $[1]_4$           | $[0]_0$           | $[1]_2$           | $[0]_2$           | 1** 400 | 60 $\rightarrow$ 46 * |
| 2:    | $[1]_\circ^+$     | $[0]_0$           | $[1]_\circ$       | $[0]_0$           | 2* 72   | 12                    |
| 3:    | $[1]_5$           | $[0]_1$           | $[1]_3$           | $[0]_0$           | 2* 480  | 60                    |
| 4:    | $[1]_6$           | $[0]_6$           | $[1]_2$           | $[0]_0$           | 2* 336  | 48                    |
| 5:    | $[1]_6$           | $[0]_0$           | $[1]_1$           | $[0]_1$           | 2* 384  | 48                    |
| 6:    | $[1]_7$           | $[0]_3$           | $[1]_1$           | $[0]_0$           | 2* 224  | 24                    |
| 7:    | $[1]_7$           | $[0]_7$           | $[1]_3$           | $[0]_2$           | 2* 320  | 40 $\rightarrow$ 36 * |
| 8:    | $[1]_7$           | $[0]_1$           | $[1]_2$           | $[0]_3$           | 2* 256  | 32                    |
| 9:    | $[2]_\bullet$     | $[0]_0$           | $[0]_0$           | $[0]_0$           | 1 30    | 5                     |
| 11:   | $[2]_\circ$       | $[0]_\circ$       | $[0]_0$           | $[0]_0$           | 1 56    | 7                     |
| 13:   | $[2]_\circ$       | $[0]_0$           | $[0]_\circ^+$     | $[0]_0$           | 1 12    | 3                     |
| 15:   | $[2]_\circ$       | $[0]_0$           | $[0]_\circ^-$     | $[0]_0$           | 1 2     | 1                     |
| 17:   | $[2]_\circ$       | $[0]_0$           | $[0]_0$           | $[0]_\circ$       | 1 40    | 5                     |
| <hr/> |                   |                   |                   |                   |         |                       |
| 11:   | $[2]_\circ$       | $[2]_\circ$       | $[0]_0$           | $[0]_0$           | 4824    | 684 $\rightarrow$ 604 |
| 1:    | $[2]_\circ$       | $[0]_0$           | $[0]_\circ$       | $[0]_0$           | 4* 40   | 5                     |
| 2:    | $[1]_4$           | $[1]_4$           | $[0]_0$           | $[0]_0$           | 1** 400 | 60                    |
| 3:    | $[1]_\circ^+$     | $[1]_\circ$       | $[0]_0$           | $[0]_0$           | 4* 36   | 6                     |
| 4:    | $[1]_5$           | $[1]_7$           | $[0]_0$           | $[0]_3$           | 8* 240  | 30                    |

|            |                                              |                                           |                                        |                                          |    |      |           |
|------------|----------------------------------------------|-------------------------------------------|----------------------------------------|------------------------------------------|----|------|-----------|
| 5:         | $\begin{bmatrix} 1 \\ 6 \end{bmatrix}$       | $\begin{bmatrix} 1 \\ 6 \end{bmatrix}$    | $\begin{bmatrix} 0 \\ 2 \end{bmatrix}$ | $\begin{bmatrix} 0 \\ 0 \end{bmatrix}$   | 4* | 360  | 60 → 42*  |
| 6:         | $\begin{bmatrix} 1 \\ 7 \end{bmatrix}$       | $\begin{bmatrix} 1 \\ 7 \end{bmatrix}$    | $\begin{bmatrix} 0 \\ 3 \end{bmatrix}$ | $\begin{bmatrix} 0 \\ 2 \end{bmatrix}$   | 4* | 160  | 20 → 18*  |
| 7:         | $\begin{bmatrix} 2 \\ \bullet \end{bmatrix}$ | $\begin{bmatrix} 0 \\ 0 \end{bmatrix}$    | $\begin{bmatrix} 0 \\ 0 \end{bmatrix}$ | $\begin{bmatrix} 0 \\ 0 \end{bmatrix}$   | 2  | 30   | 5         |
| <b>12:</b> | $\begin{bmatrix} 7 \\ 8 \end{bmatrix}_7$     | $\begin{bmatrix} 15 \\ 8 \end{bmatrix}_5$ | $\begin{bmatrix} 0 \\ 0 \end{bmatrix}$ | $\begin{bmatrix} 5 \\ 4 \end{bmatrix}_1$ |    | 4344 | 652 → 600 |
| 1:         | $\begin{bmatrix} 1 \\ 0 \end{bmatrix}$       | $\begin{bmatrix} 1 \\ 0 \end{bmatrix}$    | $\begin{bmatrix} 0 \\ 0 \end{bmatrix}$ | $\begin{bmatrix} 0 \\ 0 \end{bmatrix}$   | 1  | 105  | 15        |
| 3:         | $\begin{bmatrix} 1 \\ 0 \end{bmatrix}$       | $\begin{bmatrix} 0 \\ 0 \end{bmatrix}$    | $\begin{bmatrix} 0 \\ 0 \end{bmatrix}$ | $\begin{bmatrix} 1 \\ 0 \end{bmatrix}$   | 1  | 70   | 10        |
| 5:         | $\begin{bmatrix} 1 \\ 2 \end{bmatrix}_4$     | $\begin{bmatrix} 3 \\ 2 \end{bmatrix}_4$  | $\begin{bmatrix} 0 \\ 0 \end{bmatrix}$ | $\begin{bmatrix} 0 \\ 0 \end{bmatrix}$   | 1  | 175  | 25        |
| 7:         | $\begin{bmatrix} 5 \\ 8 \end{bmatrix}_5$     | $\begin{bmatrix} 5 \\ 8 \end{bmatrix}_7$  | $\begin{bmatrix} 0 \\ 0 \end{bmatrix}$ | $\begin{bmatrix} 3 \\ 4 \end{bmatrix}_3$ | 1  | 315  | 45        |
| 9:         | $\begin{bmatrix} 3 \\ 4 \end{bmatrix}_6$     | $\begin{bmatrix} 5 \\ 4 \end{bmatrix}_6$  | $\begin{bmatrix} 0 \\ 2 \end{bmatrix}$ | $\begin{bmatrix} 0 \\ 0 \end{bmatrix}$   | 1  | 210  | 30 → 24*  |
| 11:        | $\begin{bmatrix} 3 \\ 4 \end{bmatrix}_6$     | $\begin{bmatrix} 3 \\ 4 \end{bmatrix}_2$  | $\begin{bmatrix} 0 \\ 0 \end{bmatrix}$ | $\begin{bmatrix} 1 \\ 2 \end{bmatrix}_2$ | 1  | 350  | 50        |
| 13:        | $\begin{bmatrix} 3 \\ 4 \end{bmatrix}_6$     | $\begin{bmatrix} 0 \\ 0 \end{bmatrix}$    | $\begin{bmatrix} 0 \\ 1 \end{bmatrix}$ | $\begin{bmatrix} 5 \\ 4 \end{bmatrix}_1$ | 1  | 112  | 14        |
| 15:        | $\begin{bmatrix} 7 \\ 8 \end{bmatrix}_7$     | $\begin{bmatrix} 15 \\ 8 \end{bmatrix}_5$ | $\begin{bmatrix} 0 \\ 0 \end{bmatrix}$ | $\begin{bmatrix} 3 \\ 4 \end{bmatrix}_1$ | 1  | 5    | 1         |
| 17:        | $\begin{bmatrix} 7 \\ 8 \end{bmatrix}_7$     | $\begin{bmatrix} 9 \\ 8 \end{bmatrix}_3$  | $\begin{bmatrix} 0 \\ 1 \end{bmatrix}$ | $\begin{bmatrix} 0 \\ 0 \end{bmatrix}$   | 1  | 160  | 20        |
| 19:        | $\begin{bmatrix} 7 \\ 8 \end{bmatrix}_7$     | $\begin{bmatrix} 7 \\ 8 \end{bmatrix}_5$  | $\begin{bmatrix} 0 \\ 0 \end{bmatrix}$ | $\begin{bmatrix} 1 \\ 4 \end{bmatrix}_1$ | 1  | 150  | 30        |
| 21:        | $\begin{bmatrix} 7 \\ 8 \end{bmatrix}_7$     | $\begin{bmatrix} 1 \\ 8 \end{bmatrix}_5$  | $\begin{bmatrix} 0 \\ 0 \end{bmatrix}$ | $\begin{bmatrix} 5 \\ 4 \end{bmatrix}_1$ | 1  | 30   | 6         |
| 23:        | $\begin{bmatrix} 7 \\ 8 \end{bmatrix}_7$     | $\begin{bmatrix} 5 \\ 8 \end{bmatrix}_7$  | $\begin{bmatrix} 0 \\ 3 \end{bmatrix}$ | $\begin{bmatrix} 1 \\ 2 \end{bmatrix}_2$ | 1  | 240  | 30        |
| 25:        | $\begin{bmatrix} 7 \\ 8 \end{bmatrix}_7$     | $\begin{bmatrix} 3 \\ 8 \end{bmatrix}_1$  | $\begin{bmatrix} 0 \\ 2 \end{bmatrix}$ | $\begin{bmatrix} 3 \\ 4 \end{bmatrix}_3$ | 1  | 250  | 50 → 30*  |

3.1.1. *Vector 1.*

```

1 := rec(fixed := 4, min := 64, chain := 3),
2 := rec(fixed := -3, min := 44, chain := 2),
4 := rec(fixed := 4, min := 114, chain := 2),
6 := rec(fixed := -3, min := 32),

```

3.2. **The lattice  $N(4\mathbf{A}_6)$ .** There are 4 classes;  $b(\mathfrak{D}) \leq 704$ .

|           |                   |                    |                    |                    |          |                                  |
|-----------|-------------------|--------------------|--------------------|--------------------|----------|----------------------------------|
| <b>1:</b> | $[4]_{\bullet}$   | $[0]_0$            | $[0]_0$            | $[0]_0$            | 5336     | 766 $\rightarrow$ 628            |
| 1:        | $[2]_{\bullet}^+$ | $[0]_0$            | $[0]_0$            | $[0]_0$            | $2^*$    | 3 <u>1</u>                       |
| 2:        | $[2]_{\bullet}^-$ | $[0]_0$            | $[0]_0$            | $[0]_0$            | $1^{**}$ | 24 <u>6</u>                      |
| 3:        | $[2]_{\circ}$     | $[0]_{\circ}$      | $[0]_0$            | $[0]_0$            | $3^{**}$ | 168 24 $\rightarrow$ <u>22</u> ✓ |
| 4:        | $[2]_4$           | $[0]_2$            | $[0]_6$            | $[0]_0$            | $6^*$    | 441 63 $\rightarrow$ <u>49</u> ✓ |
| 5:        | $[2]_5$           | $[0]_4$            | $[0]_0$            | $[0]_6$            | $6^*$    | 245 35 $\rightarrow$ <u>27</u> ✓ |
| 6:        | $[2]_5$           | $[0]_1$            | $[0]_1$            | $[0]_1$            | $2^*$    | 343 49                           |
| <b>2:</b> | $[\frac{6}{7}]_6$ | $[\frac{6}{7}]_6$  | $[\frac{6}{7}]_1$  | $[\frac{10}{7}]_5$ | 4376     | 748 $\rightarrow$ 604            |
| 1:        | $[1]_{\circ}$     | $[1]_{\circ}$      | $[0]_0$            | $[0]_0$            | 3        | 36 <u>6</u>                      |
| 3:        | $[1]_{\circ}$     | $[0]_0$            | $[0]_0$            | $[1]_{\circ}$      | 3        | 60 <u>10</u>                     |
| 5:        | $[\frac{4}{7}]_4$ | $[\frac{6}{7}]_6$  | $[0]_0$            | $[\frac{4}{7}]_2$  | 3        | 150 30 $\rightarrow$ <u>20</u> ✓ |
| 7:        | $[\frac{4}{7}]_4$ | $[0]_0$            | $[\frac{5}{7}]_2$  | $[\frac{5}{7}]_6$  | 3        | 180 30 $\rightarrow$ <u>24</u> ✓ |
| 9:        | $[\frac{3}{7}]_3$ | $[\frac{5}{7}]_5$  | $[\frac{6}{7}]_1$  | $[0]_0$            | 3        | 120 18 $\rightarrow$ <u>16</u> ✓ |
| 11:       | $[\frac{5}{7}]_5$ | $[\frac{1}{7}]_1$  | $[\frac{6}{7}]_1$  | $[\frac{2}{7}]_1$  | 3        | 180 30 $\rightarrow$ <u>24</u> ✓ |
| 13:       | $[\frac{6}{7}]_6$ | $[\frac{6}{7}]_6$  | $[\frac{6}{7}]_1$  | $[\frac{4}{7}]_5$  | 1        | 10 <u>2</u>                      |
| <b>3:</b> | $[2]_{\circ}$     | $[2]_{\circ}$      | $[0]_0$            | $[0]_0$            | 4856     | 704                              |
| 1:        | $[1]_{\circ}^+$   | $[1]_{\circ}^+$    | $[0]_0$            | $[0]_0$            | $4^*$    | 25 5                             |
| 2:        | $[1]_4$           | $[1]_2$            | $[0]_6$            | $[0]_0$            | $4^*$    | 350 50                           |
| 3:        | $[1]_4$           | $[1]_6$            | $[0]_0$            | $[0]_2$            | $4^*$    | 210 30                           |
| 4:        | $[1]_5$           | $[1]_6$            | $[0]_4$            | $[0]_0$            | $4^*$    | 175 25                           |
| 5:        | $[1]_5$           | $[1]_1$            | $[0]_1$            | $[0]_1$            | $4^*$    | 245 35                           |
| 6:        | $[1]_6$           | $[1]_6$            | $[0]_1$            | $[0]_5$            | $4^*$    | 147 21                           |
| 7:        | $[2]_{\bullet}$   | $[0]_0$            | $[0]_0$            | $[0]_0$            | 2        | 20 4                             |
| 9:        | $[2]_{\circ}$     | $[0]_0$            | $[0]_{\circ}$      | $[0]_0$            | 2        | 42 6                             |
| <b>4:</b> | $[\frac{6}{7}]_6$ | $[\frac{12}{7}]_3$ | $[\frac{10}{7}]_2$ | $[0]_0$            | 4376     | 688                              |
| 1:        | $[\frac{3}{7}]_3$ | $[\frac{6}{7}]_5$  | $[\frac{5}{7}]_1$  | $[0]_0$            | $1^{**}$ | 240 36                           |
| 2:        | $[1]_{\circ}$     | $[1]_{\circ}$      | $[0]_0$            | $[0]_0$            | 1        | 72 12                            |
| 4:        | $[1]_{\circ}$     | $[0]_0$            | $[1]_{\circ}$      | $[0]_0$            | 1        | 60 10                            |
| 6:        | $[\frac{4}{7}]_4$ | $[\frac{8}{7}]_2$  | $[\frac{2}{7}]_6$  | $[0]_0$            | 1        | 225 45                           |
| 8:        | $[\frac{4}{7}]_4$ | $[0]_0$            | $[\frac{10}{7}]_2$ | $[0]_6$            | 1        | 105 15                           |
| 10:       | $[\frac{5}{7}]_5$ | $[\frac{9}{7}]_4$  | $[0]_0$            | $[0]_6$            | 1        | 168 24                           |
| 12:       | $[\frac{5}{7}]_5$ | $[\frac{4}{7}]_1$  | $[\frac{5}{7}]_1$  | $[0]_1$            | 1        | 252 36                           |
| 14:       | $[\frac{5}{7}]_5$ | $[\frac{3}{7}]_6$  | $[\frac{6}{7}]_4$  | $[0]_0$            | 1        | 240 40                           |
| 16:       | $[\frac{6}{7}]_6$ | $[\frac{12}{7}]_3$ | $[\frac{4}{7}]_2$  | $[0]_0$            | 1        | 10 2                             |
| 18:       | $[\frac{6}{7}]_6$ | $[\frac{5}{7}]_3$  | $[\frac{3}{7}]_2$  | $[0]_0$            | 1        | 120 24                           |

|     |                              |                              |                               |         |   |     |    |
|-----|------------------------------|------------------------------|-------------------------------|---------|---|-----|----|
| 20: | $\left[\frac{6}{7}\right]_6$ | $\left[\frac{2}{7}\right]_3$ | $\left[\frac{10}{7}\right]_2$ | $[0]_0$ | 1 | 18  | 4  |
| 22: | $\left[\frac{6}{7}\right]_6$ | $\left[\frac{8}{7}\right]_2$ | $[0]_0$                       | $[0]_3$ | 1 | 105 | 15 |
| 24: | $\left[\frac{6}{7}\right]_6$ | $\left[\frac{6}{7}\right]_5$ | $\left[\frac{2}{7}\right]_6$  | $[0]_1$ | 1 | 210 | 30 |
| 26: | $\left[\frac{6}{7}\right]_6$ | $\left[\frac{4}{7}\right]_1$ | $\left[\frac{4}{7}\right]_5$  | $[0]_6$ | 1 | 210 | 30 |
| 28: | $\left[\frac{6}{7}\right]_6$ | $\left[\frac{3}{7}\right]_6$ | $\left[\frac{5}{7}\right]_1$  | $[0]_5$ | 1 | 168 | 24 |
| 30: | $\left[\frac{6}{7}\right]_6$ | $[0]_0$                      | $\left[\frac{8}{7}\right]_3$  | $[0]_2$ | 1 | 105 | 15 |

---

### 3.2.1. *Vector 1.*

```

1 := rec(),
2 := rec(),
3 := rec(),
4 := rec(fixed := 3, min := 49, chain := [2, 2]),
5 := rec(fixed := 4, min := 27, chain := [3, 2]),

```

### 3.2.2. *Vector 2.*

```

1 := rec(),
3 := rec(),
5 := rec(fixed := 4, min := 20, chain := 3),
7 := rec(fixed := 1, min := 24, chain := [3, 3]),
9 := rec(fixed := 1, min := 16, chain := [3, 3]),
11 := rec(fixed := 4, min := 24, chain := [2, 2]),
13 := rec(),

```

3.3. **The lattice  $N(4\mathbf{A}_5 \oplus \mathbf{D}_4)$ .** There are 8 classes;  $b(\mathfrak{Q}) \leq 716$ .

|           |                   |                   |                   |         |                   |          |                                  |
|-----------|-------------------|-------------------|-------------------|---------|-------------------|----------|----------------------------------|
| <b>1:</b> | $[0]_0$           | $[0]_0$           | $[0]_0$           | $[0]_0$ | $[4]_{\bullet}^3$ | 5848     | 962 $\rightarrow$ 706            |
| 1:        | $[0]_{\circ}$     | $[0]_0$           | $[0]_0$           | $[0]_0$ | $[2]_{\circ}$     | $4^{**}$ | 180 30 $\rightarrow$ <u>24</u> ✓ |
| 2:        | $[0]_3$           | $[0]_0$           | $[0]_0$           | $[0]_3$ | $[2]_3$           | $2^{**}$ | 400 60 $\rightarrow$ <u>48</u> ✓ |
| 3:        | $[0]_4$           | $[0]_1$           | $[0]_5$           | $[0]_0$ | $[2]_3$           | $8^*$    | 540 90 $\rightarrow$ <u>64</u> ✓ |
| 4:        | $[0]_0$           | $[0]_0$           | $[0]_0$           | $[0]_0$ | $[2]_{\bullet}^2$ | $2^*$    | 4 <u>1</u>                       |
| <b>2:</b> | $[4]_{\bullet}$   | $[0]_0$           | $[0]_0$           | $[0]_0$ | $[0]_0$           | 5368     | 926 $\rightarrow$ 690            |
| 1:        | $[2]_{\bullet}^+$ | $[0]_0$           | $[0]_0$           | $[0]_0$ | $[0]_0$           | $2^*$    | 1 <u>1</u>                       |
| 2:        | $[2]_{\bullet}^-$ | $[0]_0$           | $[0]_0$           | $[0]_0$ | $[0]_0$           | $1^{**}$ | 8 <u>2</u>                       |
| 3:        | $[2]_{\circ}$     | $[0]_{\circ}$     | $[0]_0$           | $[0]_0$ | $[0]_0$           | $3^{**}$ | 120 20 $\rightarrow$ <u>18</u> ✓ |
| 4:        | $[2]_{\circ}$     | $[0]_0$           | $[0]_0$           | $[0]_0$ | $[0]_{\circ}$     | $1^{**}$ | 96 16 $\rightarrow$ <u>14</u> ✓  |
| 5:        | $[2]_3$           | $[0]_3$           | $[0]_0$           | $[0]_0$ | $[0]_1$           | $3^{**}$ | 320 48 $\rightarrow$ <u>40</u> ✓ |
| 6:        | $[2]_3$           | $[0]_5$           | $[0]_5$           | $[0]_5$ | $[0]_0$           | $2^*$    | 432 72 $\rightarrow$ <u>54</u> ✓ |
| 7:        | $[2]_4$           | $[0]_4$           | $[0]_2$           | $[0]_0$ | $[0]_0$           | $6^*$    | 225 45 $\rightarrow$ <u>29</u> ✓ |
| 8:        | $[2]_4$           | $[0]_5$           | $[0]_0$           | $[0]_1$ | $[0]_2$           | $6^*$    | 288 48 $\rightarrow$ <u>36</u> ✓ |
| <b>3:</b> | $[\frac{5}{6}]_5$ | $[\frac{5}{6}]_5$ | $[\frac{4}{3}]_4$ | $[0]_0$ | $[1]_1$           | 4408     | 824 $\rightarrow$ 704            |
| 1:        | $[\frac{2}{3}]_4$ | $[\frac{1}{6}]_1$ | $[\frac{2}{3}]_5$ | $[0]_0$ | $[\frac{1}{2}]_3$ | $2^*$    | 200 40 $\rightarrow$ <u>32</u> ✓ |
| 2:        | $[\frac{5}{6}]_5$ | $[0]_0$           | $[\frac{2}{3}]_2$ | $[0]_1$ | $[\frac{1}{2}]_3$ | $2^*$    | 144 24 $\rightarrow$ <u>22</u> ✓ |
| 3:        | $[\frac{5}{6}]_5$ | $[0]_0$           | $[\frac{2}{3}]_5$ | $[0]_4$ | $[\frac{1}{2}]_2$ | $2^*$    | 120 24 $\rightarrow$ <u>18</u> ✓ |
| 4:        | $[1]_{\circ}$     | $[1]_{\circ}$     | $[0]_0$           | $[0]_0$ | $[0]_0$           | 1        | 25 <u>5</u>                      |
| 6:        | $[1]_{\circ}$     | $[0]_0$           | $[1]_{\circ}$     | $[0]_0$ | $[0]_0$           | 2        | 40 <u>8</u>                      |
| 8:        | $[1]_{\circ}$     | $[0]_0$           | $[0]_0$           | $[0]_0$ | $[1]_{\circ}$     | 2        | 30 <u>6</u>                      |
| 10:       | $[\frac{1}{2}]_3$ | $[\frac{1}{2}]_3$ | $[0]_0$           | $[0]_0$ | $[1]_1$           | 1        | 100 20 $\rightarrow$ <u>16</u> ✓ |
| 12:       | $[\frac{1}{2}]_3$ | $[\frac{5}{6}]_5$ | $[\frac{2}{3}]_5$ | $[0]_5$ | $[0]_0$           | 2        | 120 20 $\rightarrow$ <u>18</u> ✓ |
| 14:       | $[\frac{1}{2}]_3$ | $[0]_0$           | $[1]_3$           | $[0]_0$ | $[\frac{1}{2}]_2$ | 2        | 160 32 $\rightarrow$ <u>26</u> ✓ |
| 16:       | $[\frac{2}{3}]_4$ | $[\frac{2}{3}]_4$ | $[\frac{2}{3}]_2$ | $[0]_0$ | $[0]_0$           | 1        | 150 30 $\rightarrow$ <u>24</u> ✓ |
| 18:       | $[\frac{2}{3}]_4$ | $[\frac{5}{6}]_5$ | $[0]_0$           | $[0]_1$ | $[\frac{1}{2}]_2$ | 2        | 120 20 $\rightarrow$ <u>18</u> ✓ |
| 20:       | $[\frac{2}{3}]_4$ | $[0]_0$           | $[\frac{4}{3}]_4$ | $[0]_2$ | $[0]_0$           | 2        | 75 15 $\rightarrow$ <u>11</u> ✓  |
| 22:       | $[\frac{2}{3}]_4$ | $[0]_0$           | $[\frac{1}{3}]_1$ | $[0]_5$ | $[1]_1$           | 2        | 120 20 $\rightarrow$ <u>18</u> ✓ |
| 24:       | $[\frac{5}{6}]_5$ | $[\frac{5}{6}]_5$ | $[\frac{4}{3}]_4$ | $[0]_0$ | $[-1]_1$          | 1        | 1 <u>1</u>                       |
| 26:       | $[\frac{5}{6}]_5$ | $[\frac{5}{6}]_5$ | $[\frac{1}{3}]_4$ | $[0]_0$ | $[0]_1$           | 1        | 48 12 $\rightarrow$ <u>10</u> *  |
| 28:       | $[\frac{5}{6}]_5$ | $[\frac{5}{6}]_5$ | $[\frac{2}{3}]_4$ | $[0]_0$ | $[1]_1$           | 1        | 6 <u>2</u>                       |
| 30:       | $[\frac{5}{6}]_5$ | $[\frac{5}{6}]_5$ | $[\frac{1}{3}]_1$ | $[0]_3$ | $[0]_0$           | 1        | 80 <u>12</u>                     |
| <b>4:</b> | $[2]_{\circ}$     | $[0]_0$           | $[0]_0$           | $[0]_0$ | $[2]_{\circ}$     | 4888     | 814 $\rightarrow$ 688            |
| 1:        | $[1]_{\circ}^+$   | $[0]_0$           | $[0]_0$           | $[0]_0$ | $[1]_{\circ}$     | $2^*$    | 32 <u>8</u>                      |
| 2:        | $[1]_3$           | $[0]_3$           | $[0]_0$           | $[0]_0$ | $[1]_1$           | $3^{**}$ | 240 36 $\rightarrow$ <u>34</u> ✓ |

|       |                   |                   |                   |                   |                   |          |      |                                   |
|-------|-------------------|-------------------|-------------------|-------------------|-------------------|----------|------|-----------------------------------|
| 3:    | $[1]_4$           | $[0]_5$           | $[0]_0$           | $[0]_1$           | $[1]_2$           | $6^*$    | 288  | $48 \rightarrow \underline{40}$ ✓ |
| 4:    | $[1]_5$           | $[0]_4$           | $[0]_0$           | $[0]_5$           | $[1]_3$           | $12^*$   | 180  | $30 \rightarrow \underline{24}$ ✓ |
| 5:    | $[2]_\bullet$     | $[0]_0$           | $[0]_0$           | $[0]_0$           | $[0]_0$           | 1        | 12   | $\underline{3}$                   |
| 7:    | $[2]_\circ$       | $[0]_\circ$       | $[0]_0$           | $[0]_0$           | $[0]_0$           | 3        | 30   | $\underline{5}$                   |
| 9:    | $[2]_\circ$       | $[0]_0$           | $[0]_0$           | $[0]_0$           | $[0]_\circ^+$     | 3        | 2    | $\underline{1}$                   |
| <hr/> |                   |                   |                   |                   |                   |          |      |                                   |
| 5:    | $[\frac{3}{2}]_3$ | $[\frac{3}{2}]_3$ | $[0]_0$           | $[0]_0$           | $[1]_1$           |          | 4408 | $836 \rightarrow 712$             |
| 1:    | $[\frac{3}{2}]_3$ | $[0]_0$           | $[0]_3$           | $[0]_0$           | $[\frac{1}{2}]_2$ | $4^*$    | 80   | $\underline{12}$                  |
| 2:    | $[1]_4$           | $[\frac{1}{2}]_5$ | $[0]_0$           | $[0]_1$           | $[\frac{1}{2}]_2$ | $8^*$    | 216  | $36 \rightarrow \underline{34}$ ✓ |
| 3:    | $[2]_\bullet$     | $[0]_0$           | $[0]_0$           | $[0]_0$           | $[0]_0$           | 2        | 9    | $3 \rightarrow \underline{2}$ ✓   |
| 5:    | $[1]_\circ$       | $[1]_\circ$       | $[0]_0$           | $[0]_0$           | $[0]_0$           | 1        | 81   | $27 \rightarrow \underline{19}$ ✓ |
| 7:    | $[1]_\circ$       | $[0]_0$           | $[0]_0$           | $[0]_0$           | $[1]_\circ$       | 2        | 54   | $18 \rightarrow \underline{12}^*$ |
| 9:    | $[\frac{3}{2}]_3$ | $[\frac{3}{2}]_3$ | $[0]_0$           | $[0]_0$           | $[-1]_1$          | 1        | 1    | $\underline{1}$                   |
| 11:   | $[\frac{3}{2}]_3$ | $[\frac{1}{2}]_5$ | $[0]_5$           | $[0]_5$           | $[0]_0$           | 4        | 108  | $18 \rightarrow \underline{16}$ ✓ |
| 13:   | $[1]_4$           | $[1]_4$           | $[0]_2$           | $[0]_0$           | $[0]_0$           | 4        | 135  | $27 \rightarrow \underline{21}$ ✓ |
| <hr/> |                   |                   |                   |                   |                   |          |      |                                   |
| 6:    | $[2]_\circ$       | $[2]_\circ$       | $[0]_0$           | $[0]_0$           | $[0]_0$           |          | 4888 | $888 \rightarrow 690$             |
| 1:    | $[2]_\circ$       | $[0]_0$           | $[0]_\circ$       | $[0]_0$           | $[0]_0$           | $4^*$    | 30   | $\underline{5}$                   |
| 2:    | $[2]_\circ$       | $[0]_0$           | $[0]_0$           | $[0]_0$           | $[0]_\circ$       | $2^*$    | 24   | $\underline{4}$                   |
| 3:    | $[1]_\circ^+$     | $[1]_\circ^+$     | $[0]_0$           | $[0]_0$           | $[0]_0$           | $4^*$    | 16   | $\underline{4}$                   |
| 4:    | $[1]_3$           | $[1]_3$           | $[0]_0$           | $[0]_0$           | $[0]_1$           | $1^{**}$ | 288  | $72 \rightarrow \underline{42}$ ✓ |
| 5:    | $[1]_3$           | $[1]_5$           | $[0]_5$           | $[0]_5$           | $[0]_0$           | $4^*$    | 216  | $36 \rightarrow \underline{30}$ ✓ |
| 6:    | $[1]_4$           | $[1]_4$           | $[0]_2$           | $[0]_0$           | $[0]_0$           | $4^*$    | 240  | $48 \rightarrow \underline{34}$ ✓ |
| 7:    | $[1]_4$           | $[1]_5$           | $[0]_0$           | $[0]_1$           | $[0]_2$           | $8^*$    | 192  | $32 \rightarrow \underline{26}$ ✓ |
| 8:    | $[1]_5$           | $[1]_5$           | $[0]_4$           | $[0]_0$           | $[0]_1$           | $4^*$    | 120  | $24 \rightarrow \underline{16}$ ✓ |
| 9:    | $[1]_5$           | $[1]_5$           | $[0]_1$           | $[0]_3$           | $[0]_0$           | $4^*$    | 120  | $18 \rightarrow \underline{16}$ ✓ |
| 10:   | $[2]_\bullet$     | $[0]_0$           | $[0]_0$           | $[0]_0$           | $[0]_0$           | 2        | 12   | $\underline{3}$                   |
| <hr/> |                   |                   |                   |                   |                   |          |      |                                   |
| 7:    | $[\frac{4}{3}]_4$ | $[\frac{4}{3}]_4$ | $[\frac{4}{3}]_2$ | $[0]_0$           | $[0]_0$           |          | 4408 | $936 \rightarrow 716$             |
| 1:    | $[1]_3$           | $[\frac{2}{3}]_5$ | $[\frac{1}{3}]_5$ | $[0]_5$           | $[0]_0$           | $6^*$    | 192  | $32 \rightarrow \underline{30}$ ✓ |
| 2:    | $[\frac{4}{3}]_4$ | $[\frac{2}{3}]_2$ | $[0]_0$           | $[0]_4$           | $[0]_0$           | $6^*$    | 90   | $18 \rightarrow \underline{14}$ ✓ |
| 3:    | $[\frac{4}{3}]_4$ | $[\frac{2}{3}]_5$ | $[0]_0$           | $[0]_1$           | $[0]_2$           | $6^*$    | 96   | $16 \rightarrow \underline{14}^*$ |
| 4:    | $[\frac{2}{3}]_2$ | $[\frac{2}{3}]_2$ | $[\frac{2}{3}]_4$ | $[0]_0$           | $[0]_0$           | $1^{**}$ | 216  | $72 \rightarrow \underline{38}$ ✓ |
| 5:    | $[\frac{2}{3}]_2$ | $[\frac{2}{3}]_5$ | $[\frac{2}{3}]_1$ | $[0]_0$           | $[0]_3$           | $3^{**}$ | 192  | $48 \rightarrow \underline{30}$ ✓ |
| 6:    | $[\frac{2}{3}]_5$ | $[\frac{2}{3}]_5$ | $[\frac{2}{3}]_1$ | $[0]_3$           | $[0]_0$           | $1^{**}$ | 160  | $\underline{24}$                  |
| 7:    | $[2]_\bullet$     | $[0]_0$           | $[0]_0$           | $[0]_0$           | $[0]_0$           | 3        | 6    | $\underline{2}$                   |
| 9:    | $[1]_\circ$       | $[1]_\circ$       | $[0]_0$           | $[0]_0$           | $[0]_0$           | 3        | 64   | $16 \rightarrow \underline{14}$ ✓ |
| 11:   | $[1]_3$           | $[1]_3$           | $[0]_0$           | $[0]_0$           | $[0]_1$           | 3        | 128  | $32 \rightarrow \underline{20}^*$ |
| <hr/> |                   |                   |                   |                   |                   |          |      |                                   |
| 8:    | $[\frac{5}{6}]_5$ | $[\frac{5}{6}]_5$ | $[\frac{5}{6}]_1$ | $[\frac{3}{2}]_3$ | $[0]_0$           |          | 4408 | $884 \rightarrow 702$             |

|     |                                                    |                                                    |                                                    |                                                    |                                          |   |     |                                            |
|-----|----------------------------------------------------|----------------------------------------------------|----------------------------------------------------|----------------------------------------------------|------------------------------------------|---|-----|--------------------------------------------|
| 1:  | $\begin{bmatrix} 1 \\ 0 \end{bmatrix}_0$           | $\begin{bmatrix} 1 \\ 0 \end{bmatrix}_0$           | $\begin{bmatrix} 0 \\ 0 \end{bmatrix}_0$           | $\begin{bmatrix} 0 \\ 0 \end{bmatrix}_0$           | $\begin{bmatrix} 0 \\ 0 \end{bmatrix}_0$ | 3 | 25  | $\underline{5}$                            |
| 3:  | $\begin{bmatrix} 1 \\ 0 \end{bmatrix}_0$           | $\begin{bmatrix} 0 \\ 0 \end{bmatrix}_0$           | $\begin{bmatrix} 0 \\ 0 \end{bmatrix}_0$           | $\begin{bmatrix} 1 \\ 0 \end{bmatrix}_0$           | $\begin{bmatrix} 0 \\ 0 \end{bmatrix}_0$ | 3 | 45  | $\underline{9}$                            |
| 5:  | $\begin{bmatrix} \frac{1}{2} \\ 3 \end{bmatrix}_3$ | $\begin{bmatrix} \frac{5}{6} \\ 5 \end{bmatrix}_5$ | $\begin{bmatrix} \frac{1}{6} \\ 5 \end{bmatrix}_5$ | $\begin{bmatrix} \frac{1}{2} \\ 5 \end{bmatrix}_5$ | $\begin{bmatrix} 0 \\ 0 \end{bmatrix}_0$ | 6 | 150 | $30 \rightarrow \underline{24} \checkmark$ |
| 7:  | $\begin{bmatrix} \frac{1}{2} \\ 3 \end{bmatrix}_3$ | $\begin{bmatrix} 0 \\ 0 \end{bmatrix}_0$           | $\begin{bmatrix} 0 \\ 0 \end{bmatrix}_0$           | $\begin{bmatrix} \frac{3}{2} \\ 3 \end{bmatrix}_3$ | $\begin{bmatrix} 0 \\ 3 \end{bmatrix}_3$ | 3 | 80  | $16 \rightarrow \underline{12} *$          |
| 9:  | $\begin{bmatrix} \frac{2}{3} \\ 4 \end{bmatrix}_4$ | $\begin{bmatrix} \frac{2}{3} \\ 4 \end{bmatrix}_4$ | $\begin{bmatrix} \frac{2}{3} \\ 2 \end{bmatrix}_2$ | $\begin{bmatrix} 0 \\ 0 \end{bmatrix}_0$           | $\begin{bmatrix} 0 \\ 0 \end{bmatrix}_0$ | 1 | 125 | $25 \rightarrow \underline{19} \checkmark$ |
| 11: | $\begin{bmatrix} \frac{2}{3} \\ 4 \end{bmatrix}_4$ | $\begin{bmatrix} \frac{5}{6} \\ 5 \end{bmatrix}_5$ | $\begin{bmatrix} 0 \\ 0 \end{bmatrix}_0$           | $\begin{bmatrix} \frac{1}{2} \\ 1 \end{bmatrix}_1$ | $\begin{bmatrix} 0 \\ 2 \end{bmatrix}_2$ | 6 | 120 | $24 \rightarrow \underline{18} *$          |
| 13: | $\begin{bmatrix} \frac{5}{6} \\ 5 \end{bmatrix}_5$ | $\begin{bmatrix} \frac{5}{6} \\ 5 \end{bmatrix}_5$ | $\begin{bmatrix} \frac{5}{6} \\ 1 \end{bmatrix}_1$ | $\begin{bmatrix} \frac{1}{2} \\ 3 \end{bmatrix}_3$ | $\begin{bmatrix} 0 \\ 0 \end{bmatrix}_0$ | 1 | 9   | $3 \rightarrow \underline{2} \checkmark$   |

3.3.1. *Vector 1.*

```

1 := rec(fixed := -5, min := 24),
2 := rec(fixed := -1, min := 48, chain := 3),
3 := rec(fixed := 2, min := 64, chain := 2),
4 := rec(),

```

3.3.2. *Vector 2.*

```

1 := rec(),
2 := rec(),
3 := rec(),
4 := rec(),
5 := rec(fixed := -5, min := 40),
6 := rec(fixed := 2, min := 54, chain := [2, 2]),
7 := rec(fixed := 2, min := 29, chain := [3, 2]),
8 := rec(fixed := -5, min := 36, chain := 2),

```

3.3.3. *Vector 3.*

```

1 := rec(fixed := 5, min := 32, chain := 2),
2 := rec(fixed := -3, min := 22),
3 := rec(fixed := 3, min := 18),
4 := rec(),
6 := rec(),
8 := rec(),
10 := rec(fixed := 1, min := 16, chain := 2),
12 := rec(fixed := 3, min := 18),
14 := rec(fixed := 3, min := 26),
16 := rec(fixed := 1, min := 24, chain := 2),
18 := rec(fixed := 5, min := 18, chain := 2),
20 := rec(fixed := 1, min := 11),
22 := rec(fixed := 3, min := 18, chain := 2),
24 := rec(),
26 := rec(),
28 := rec(),
30 := rec(fixed := 3, min := 12),

```

3.3.4. *Vector 4.*

```

1 := rec(),
2 := rec(fixed := -1, min := 34),
3 := rec(fixed := 1, min := 40, chain := 2),
4 := rec(fixed := 4, min := 24, chain := 3),
5 := rec(),
7 := rec(),
9 := rec(),

```

3.3.5. *Vector 5.*

```

1 := rec(fixed := 5, min := 12),
2 := rec(fixed := 5, min := 34),
3 := rec(),
5 := rec(fixed := 1, min := 19),
7 := rec(),
9 := rec(),
11 := rec(fixed := 2, min := 16),
13 := rec(fixed := 1, min := 21)

```

3.3.6. *Vector 6.*

```

1 := rec(),
2 := rec(),
3 := rec(),
4 := rec(fixed := 1, min := 42, chain := 2),
5 := rec(fixed := -1, min := 30, chain := 2),
6 := rec(fixed := 1, min := 34),
7 := rec(fixed := 1, min := 26, chain := 2),
8 := rec(fixed := -5, min := 16, chain := 2),
9 := rec(fixed := 3, min := 16, chain := 3),
10 := rec(),

```

3.3.7. *Vector 7.*

```

1 := rec(fixed := 1, min := 30),
2 := rec(fixed := -2, min := 14),
3 := rec(fixed := -5, min := 14),
4 := rec(fixed := 1, min := 38),
5 := rec(fixed := -5, min := 30),
6 := rec(),
7 := rec(),
9 := rec(fixed := 1, min := 14),
11 := rec(fixed := -5, min := 20, chain := 2),

```

3.3.8. *Vector 8.*

```

1 := rec(),
3 := rec(),
5 := rec(fixed := 4, min := 24),
7 := rec(fixed := -5, min := 12),
9 := rec(fixed := 1, min := 19, chain := 3),
11 := rec(fixed := -5, min := 18, chain := 2),
13 := rec(),

```



## 4. FURTHER WORK REQUIRED

The next three sections deal with the remaining five Niemeier lattices rationally generated by roots, constituting the proof of **Theorem 5.1**.

Even after the exact bounds  $b(\mathfrak{o})$  for all combinatorial orbits have been computed by brute force §1.4, the cumulative bound  $b(\mathfrak{D}_h)$  still exceeds 720, sometimes more than twice. (These offending bounds are shown in bold in the tables.) Hence, we need to use the puzzle assembly §1.5 to obtain better reduced bounds  $\bar{b}$  for some of the orbits or unions thereof.

Each subsection below starts with the computation of the sets  $\mathcal{B}_m(\mathfrak{o})$  and, hence, bounds  $b(\mathfrak{o})$ , in the same notation as in §3 (see §1.4). Then, some of these sets need to be recomputed with a lower goal  $m$ , indicated as a GAP comment

# min := m.

Upon that, we outline the major steps of the further computation, in the  $\mathcal{B}_*(\dots)$ -notation of §1.1. (The order of the arguments is crucial as it may affect the convergence.) If clusters are used (see §1.7), they are described “geometrically”, usually in terms of the supports  $\text{supp } \mathfrak{o}$ .

**Convention 4.1.** We summarize the result indicating the final bound on  $\bar{b}(\mathfrak{D}_h)$  and its ingredients. Thus, the last line

$$\bar{b}(\mathfrak{D}) \leq 142_{1,6} + 480_2 + 88_3 + 8_4 = 718$$

in §4.2.2 means that, *modulo sets of large rank that have been handled separately* (see §1.2 and §1.6), for a geometric subset  $\mathfrak{C} \subset \mathfrak{D}_h$  one has

$$|\mathfrak{C} \cap (\bar{\mathfrak{o}}_1 \cup \bar{\mathfrak{o}}_6^+)| \leq 142, \quad |\mathfrak{C} \cap \bar{\mathfrak{o}}_2| \leq 480, \quad |\mathfrak{C} \cap \bar{\mathfrak{o}}_3| \leq 88, \quad |\mathfrak{C} \cap \bar{\mathfrak{o}}_4^+| \leq 8$$

and, therefore,  $|\mathfrak{C}| \leq 718$ . Note that here  $\bar{\mathfrak{o}}_4^+ = \bar{\mathfrak{o}}_4 \cup \bar{\mathfrak{o}}_5$  and  $\bar{\mathfrak{o}}_6^+ = \bar{\mathfrak{o}}_6 \cup \bar{\mathfrak{o}}_7$ , even though only  $\bar{\mathfrak{o}}_4$  and  $\bar{\mathfrak{o}}_6$  are used in the computation.

**4.1. The code.** In the subsequent sections, upon a brief verbal explanation, we present also the uppermost layer of the code, primarily so that the author himself does not forget how the results can be reproduced. The general paradigm is that, for each set  $\mathcal{B}_m^*(\dots, \mathcal{S})$  to be computed, a dedicated data object is created which holds the necessary input and a number of parameters fine-tuning the algorithm. The puzzle assembly algorithm §1.5 itself is invoked *via*

`update(<data>, m);` where  $m$  is the goal in  $\mathcal{B}_m^*$ ,

upon which `<data>.RES` is the output (with the exception of some “large” sets discarded as in §1.2, §1.6 and stored in the global variable `\\saved`). Thus, the working horse is the function

`@data(n, [src | c]);` here and below  $n$  refers to the relevant orbit  $\bar{\mathfrak{o}}_n$  as in the tables.

The optional arguments may include a reference to a previously updated data object `src` and/or a cluster `c`  $\subset \bar{\mathfrak{o}}_n$ . Most other parameters, including the minimal and maximal goals as functions of  $m$  and a particular set  $\mathfrak{C} \in \text{src.RES}$ , are set automatically; this is controlled by the function `\\rc.spp` called from within `@data`, which *may* be defined in (3.1). Clusters are created by `@(arg)` or `@@(arg)` referring, respectively, to `\\rc.dm` or `\\rc.dmm` also defined in (3.1). Their arguments are case specific; typically, `@(n)` returns the list of the “smallest” clusters for the orbit  $\bar{\mathfrak{o}}_n$ , whereas `@(c)` returns the “next level” clusters containing the given cluster `c`.

To save memory and avoid mistakes, we often use *pipes*: upon the completion of a chunk of the computation, a data object sends its partial output to the next one. A pipe is updated by a single call to `update`, and the ultimate goal  $m$  is recomputed for each pipe member on the fly (hence, no mistakes). Most pipes are created automatically in `\\rc.spp`; a simplest pipe is constructed by

`@chain(n1, n2, ...);` a straightforward computation of  $\mathcal{B}_m^*(\bar{\mathfrak{o}}_{n_1}, \bar{\mathfrak{o}}_{n_2}, \dots)$ , see (1.3).

As explained in §1.2, by default we compute  $\mathcal{B}''$ . For  $\mathcal{B}'''$  or  $\mathcal{B}^{iv}$ , we use the function

`@extend(src, δ);` after `update`, pushes the rank by  $\delta = 1$  (default) or 2 units, see §1.2.

Finally, option **(2)** in **Warning 4.5** (cf. Remark 1.20) is implemented *via*

`@select(n, S-set, src);` creates several data objects updated by a single call to `update`; the input of one of the objects contains all sets  $\mathfrak{C} \in \text{src.RES}$ , the others—only the “necessary” ones.

4.2. **The lattice  $N(6\mathbf{D}_4)$ .** There are 3 classes;  $b(\mathfrak{D}) \leq 732$ .

|           |                   |                   |                   |                   |         |         |           |      |                   |             |
|-----------|-------------------|-------------------|-------------------|-------------------|---------|---------|-----------|------|-------------------|-------------|
| <b>1:</b> | $[4]_{\bullet}^3$ | $[0]_0$           | $[0]_0$           | $[0]_0$           | $[0]_0$ | $[0]_0$ | 5848      | 1402 | $\rightarrow$     | <b>722</b>  |
| 1:        | $[2]_{\bullet}^2$ | $[0]_0$           | $[0]_0$           | $[0]_0$           | $[0]_0$ | $[0]_0$ | $2^*$     | 4    |                   | <u>1</u>    |
| 2:        | $[2]_0$           | $[0]_0$           | $[0]_0$           | $[0]_0$           | $[0]_0$ | $[0]_0$ | $5^{**}$  | 144  | $24 \rightarrow$  | <u>20</u> ✓ |
| 3:        | $[2]_3$           | $[0]_3$           | $[0]_3$           | $[0]_3$           | $[0]_0$ | $[0]_0$ | $10^{**}$ | 512  | $128 \rightarrow$ | <u>62</u> ✓ |
| <b>2:</b> | $[1]_3$           | $[1]_3$           | $[1]_3$           | $[1]_3$           | $[0]_0$ | $[0]_0$ | 4408      | 1144 | $\rightarrow$     | <b>732</b>  |
| 1:        | $[1]_3$           | $[1]_3$           | $[0]_0$           | $[0]_0$           | $[0]_3$ | $[0]_3$ | $6^*$     | 64   | $16 \rightarrow$  | <u>10</u> * |
| 2:        | $[1]_3$           | $[\frac{1}{2}]_2$ | $[\frac{1}{2}]_1$ | $[0]_0$           | $[0]_1$ | $[0]_0$ | $24^*$    | 128  | $32 \rightarrow$  | <u>20</u> * |
| 3:        | $[\frac{1}{2}]_2$ | $[\frac{1}{2}]_2$ | $[\frac{1}{2}]_2$ | $[\frac{1}{2}]_2$ | $[0]_0$ | $[0]_0$ | $2^*$     | 256  | $64 \rightarrow$  | <u>44</u> ✓ |
| 4:        | $[2]_{\bullet}^3$ | $[0]_0$           | $[0]_0$           | $[0]_0$           | $[0]_0$ | $[0]_0$ | 4         | 1    |                   | <u>1</u>    |
| 6:        | $[1]_0$           | $[1]_0$           | $[0]_0$           | $[0]_0$           | $[0]_0$ | $[0]_0$ | 6         | 36   | $12 \rightarrow$  | <u>8</u> *  |
| <b>3:</b> | $[2]_0$           | $[2]_0$           | $[0]_0$           | $[0]_0$           | $[0]_0$ | $[0]_0$ | 4888      | 1220 | $\rightarrow$     | 712         |
| 1:        | $[2]_0$           | $[0]_0$           | $[0]_0$           | $[0]_0$           | $[0]_0$ | $[0]_0$ | $8^*$     | 24   |                   | <u>4</u>    |
| 2:        | $[1]_0$           | $[1]_0$           | $[0]_0$           | $[0]_0$           | $[0]_0$ | $[0]_0$ | $1^{**}$  | 64   | $24 \rightarrow$  | <u>20</u> ✓ |
| 3:        | $[1]_3$           | $[1]_3$           | $[0]_3$           | $[0]_3$           | $[0]_0$ | $[0]_0$ | $18^{**}$ | 256  | $64 \rightarrow$  | <u>36</u> ✓ |
| 4:        | $[2]_{\bullet}^3$ | $[0]_0$           | $[0]_0$           | $[0]_0$           | $[0]_0$ | $[0]_0$ | 6         | 2    |                   | 1           |

4.2.1. *Vector 1.*

```

1 := rec(),
2 := rec(),
3 := rec(fixed := 2, min := 62, chain := 2),

```

Besides, by the puzzle assembly §1.5 we show that  $\mathcal{B}_{90}(\bar{\mathfrak{o}}_2) = \emptyset$ , reducing the bound by 12:

```

ds := @data(2);;      update(ds, 90);;

```

4.2.2. *Vector 2.*

```

1 := rec(),
2 := rec(fixed := 2, min := 20, chain := 2),
3 := rec(fixed := 1, min := 44),
4 := rec(),
6 := rec(),

```

Besides, we use the puzzle assembly §1.5 to show that  $\mathcal{B}_{144}(\bar{\mathfrak{o}}_6^+, \bar{\mathfrak{o}}_1) = \emptyset$ :

```

ch := @chain(6, 1);;   update(ch, 144);;

```

Hence,

$$\bar{b}(\mathfrak{D}) \leq 142_{1,6} + 480_2 + 88_3 + 8_4 = 718.$$

4.2.3. *Vector 3.*

```

1 := rec(),
2 := rec(),
3 := rec(fixed := -3, min := 36, chain := 3),

```

4.3. **The lattice  $N(6\mathbf{A}_4)$ .** There are 4 classes;  $b(\mathfrak{D}) \leq 820$ .

|           |                   |                   |                   |                   |                   |                   |          |      |               |                           |
|-----------|-------------------|-------------------|-------------------|-------------------|-------------------|-------------------|----------|------|---------------|---------------------------|
| <b>1:</b> | $[4]_{\bullet}$   | $[0]_0$           | $[0]_0$           | $[0]_0$           | $[0]_0$           | $[0]_0$           | 5400     | 1080 | $\rightarrow$ | <b>790</b>                |
| 1:        | $[2]_0$           | $[0]_0$           | $[0]_0$           | $[0]_0$           | $[0]_0$           | $[0]_0$           | $5^{**}$ | 80   | 16            | $\rightarrow$ <u>14</u> ✓ |
| 2:        | $[2]_3$           | $[0]_3$           | $[0]_1$           | $[0]_0$           | $[0]_0$           | $[0]_1$           | $20^*$   | 250  | 50            | $\rightarrow$ <u>36</u> ✓ |
| <b>2:</b> | $[\frac{4}{5}]_4$ | $[\frac{4}{5}]_4$ | $[\frac{4}{5}]_1$ | $[\frac{4}{5}]_1$ | $[\frac{4}{5}]_4$ | $[0]_0$           | 4440     | 1000 | $\rightarrow$ | <b>820</b>                |
| 1:        | $[\frac{3}{5}]_3$ | $[\frac{2}{5}]_2$ | $[0]_0$           | $[\frac{1}{5}]_4$ | $[\frac{4}{5}]_4$ | $[0]_0$           | $20^*$   | 96   | 24            | $\rightarrow$ <u>18</u> ✓ |
| 2:        | $[\frac{2}{5}]_2$ | $[\frac{4}{5}]_4$ | $[0]_0$           | $[0]_0$           | $[\frac{4}{5}]_4$ | $[0]_2$           | $10^*$   | 60   | 12            | $\rightarrow$ <u>10</u> ✓ |
| 3:        | $[1]_0$           | $[1]_0$           | $[0]_0$           | $[0]_0$           | $[0]_0$           | $[0]_0$           | 10       | 16   |               | <u>4</u>                  |
| 5:        | $[\frac{3}{5}]_3$ | $[\frac{3}{5}]_3$ | $[\frac{4}{5}]_1$ | $[0]_0$           | $[0]_0$           | $[0]_1$           | 10       | 80   | 16            | $\rightarrow$ <u>14</u> ✓ |
| <b>3:</b> | $[2]_0$           | $[2]_0$           | $[0]_0$           | $[0]_0$           | $[0]_0$           | $[0]_0$           | 4920     | 992  | $\rightarrow$ | <b>800</b>                |
| 1:        | $[2]_0$           | $[0]_0$           | $[0]_0$           | $[0]_0$           | $[0]_0$           | $[0]_0$           | $8^*$    | 20   |               | <u>4</u>                  |
| 2:        | $[1]_0^+$         | $[1]_0^+$         | $[0]_0$           | $[0]_0$           | $[0]_0$           | $[0]_0$           | $4^*$    | 9    |               | <u>3</u>                  |
| 3:        | $[1]_3$           | $[1]_3$           | $[0]_1$           | $[0]_0$           | $[0]_0$           | $[0]_1$           | $4^*$    | 225  | 45            | $\rightarrow$ <u>37</u> ✓ |
| 4:        | $[1]_3$           | $[1]_4$           | $[0]_4$           | $[0]_0$           | $[0]_2$           | $[0]_0$           | $16^*$   | 150  | 30            | $\rightarrow$ <u>24</u> ✓ |
| 5:        | $[1]_4$           | $[1]_4$           | $[0]_3$           | $[0]_0$           | $[0]_0$           | $[0]_3$           | $4^*$    | 100  | 20            | $\rightarrow$ <u>16</u> ✓ |
| 6:        | $[1]_4$           | $[1]_4$           | $[0]_1$           | $[0]_1$           | $[0]_4$           | $[0]_0$           | $8^*$    | 125  | 25            | $\rightarrow$ <u>19</u> ✓ |
| 7:        | $[2]_{\bullet}$   | $[0]_0$           | $[0]_0$           | $[0]_0$           | $[0]_0$           | $[0]_0$           | 2        | 6    |               | <u>2</u>                  |
| <b>4:</b> | $[\frac{4}{5}]_4$ | $[\frac{4}{5}]_4$ | $[\frac{6}{5}]_3$ | $[0]_0$           | $[0]_0$           | $[\frac{6}{5}]_3$ | 4440     | 944  | $\rightarrow$ | <b>820</b>                |
| 1:        | $[\frac{3}{5}]_3$ | $[\frac{1}{5}]_1$ | $[\frac{6}{5}]_3$ | $[0]_1$           | $[0]_0$           | $[0]_0$           | $4^*$    | 80   | 16            | $\rightarrow$ <u>14</u> ✓ |
| 2:        | $[\frac{2}{5}]_2$ | $[\frac{2}{5}]_2$ | $[\frac{3}{5}]_4$ | $[0]_0$           | $[0]_0$           | $[\frac{3}{5}]_4$ | $1^{**}$ | 144  | 48            | $\rightarrow$ <u>28</u> ✓ |
| 3:        | $[\frac{4}{5}]_4$ | $[0]_0$           | $[\frac{6}{5}]_3$ | $[0]_4$           | $[0]_3$           | $[0]_0$           | $4^*$    | 50   | 10            | $\rightarrow$ <u>8</u> ✓  |
| 4:        | $[\frac{4}{5}]_4$ | $[0]_0$           | $[\frac{4}{5}]_2$ | $[0]_2$           | $[0]_0$           | $[\frac{2}{5}]_1$ | $4^*$    | 90   | 18            | $\rightarrow$ <u>16</u> ✓ |
| 5:        | $[\frac{4}{5}]_4$ | $[0]_0$           | $[\frac{3}{5}]_4$ | $[0]_1$           | $[0]_1$           | $[\frac{3}{5}]_4$ | $2^*$    | 100  | 20            | $\rightarrow$ <u>18</u> ✓ |
| 6:        | $[1]_0$           | $[1]_0$           | $[0]_0$           | $[0]_0$           | $[0]_0$           | $[0]_0$           | 1        | 16   |               | <u>4</u>                  |
| 8:        | $[1]_0$           | $[0]_0$           | $[1]_0$           | $[0]_0$           | $[0]_0$           | $[0]_0$           | 4        | 24   |               | <u>6</u>                  |
| 10:       | $[\frac{3}{5}]_3$ | $[\frac{3}{5}]_3$ | $[\frac{2}{5}]_1$ | $[0]_0$           | $[0]_0$           | $[\frac{2}{5}]_1$ | 1        | 144  | 36            | $\rightarrow$ <u>28</u> ✓ |
| 12:       | $[\frac{3}{5}]_3$ | $[\frac{4}{5}]_4$ | $[\frac{3}{5}]_4$ | $[0]_0$           | $[0]_2$           | $[0]_0$           | 4        | 80   | 16            | $\rightarrow$ <u>14</u> ✓ |
| 14:       | $[\frac{3}{5}]_3$ | $[0]_0$           | $[\frac{4}{5}]_2$ | $[0]_0$           | $[0]_4$           | $[\frac{3}{5}]_4$ | 4        | 120  | 24            | $\rightarrow$ <u>22</u> ✓ |
| 16:       | $[\frac{2}{5}]_2$ | $[\frac{4}{5}]_4$ | $[\frac{4}{5}]_2$ | $[0]_4$           | $[0]_0$           | $[0]_0$           | 4        | 90   | 18            | $\rightarrow$ <u>16</u> ✓ |
| 18:       | $[\frac{4}{5}]_4$ | $[\frac{4}{5}]_4$ | $[\frac{6}{5}]_3$ | $[0]_0$           | $[0]_0$           | $[\frac{4}{5}]_3$ | 2        | 3    |               | <u>1</u>                  |
| 20:       | $[\frac{4}{5}]_4$ | $[\frac{4}{5}]_4$ | $[\frac{1}{5}]_3$ | $[0]_0$           | $[0]_0$           | $[\frac{1}{5}]_3$ | 1        | 36   | 12            | $\rightarrow$ <u>10</u> ✓ |
| 22:       | $[\frac{4}{5}]_4$ | $[\frac{4}{5}]_4$ | $[\frac{2}{5}]_1$ | $[0]_1$           | $[0]_4$           | $[0]_0$           | 2        | 75   | 15            | $\rightarrow$ <u>13</u> ✓ |

4.3.1. *Vector 1.*

```
1 := rec(),
2 := rec(fixed := 3, min := 36),    # min := 34
```

By the puzzle assembly §1.5 we find that  $\mathcal{B}_{54}''(\bar{o}_1) = \mathcal{B}_{650}''(\bar{o}_2) = \emptyset$ :

```
ds := @data(1);;      update(ds, 54);;
ds := @data(2);;      update(ds, 668);;
```

Hence,

$$\bar{b}(\mathfrak{D}) \leq 52_1 + 666_2 = 718.$$

4.3.2. *Vector 2.*

```
1 := rec(fixed := 1, min := 16),
2 := rec(),
3 := rec(),
5 := rec(fixed := 1, min := 13),
```

By the puzzle assembly §1.5 we have

$$\mathcal{B}_{330}''(\bar{o}_1) = \mathcal{B}_{82}''(\bar{o}_2) = \mathcal{B}_{64}'''(\bar{o}_3^+) = \mathcal{B}_{250}''(\bar{o}_5^+) = \emptyset :$$

```
ds := @data(1);;      update(ds, 330);;
ds := @data(2);;      update(ds, 82);;
ds := @data(3);;      update(ds, 64);;      @extend(ds);
ds := @data(5);;      update(ds, 250);;
```

Hence,

$$\bar{b}(\mathfrak{D}) \leq 328_1 + 80_2 + 62_3 + 248_5 = 718.$$

4.3.3. *Vector 3.*

```
1 := rec(),
2 := rec(),
3 := rec(fixed := 3, min := 37, chain := 3),
4 := rec(fixed := 1, min := 24),      # min := 20
5 := rec(fixed := 3, min := 16, chain := 2),
6 := rec(fixed := 3, min := 19, chain := 3),    # min := 16
7 := rec(),
```

We subdivide  $\bar{o}_4$  into four pairwise disjoint clusters (see §1.7)

$$\mathbf{c}_o := \{\mathfrak{o} \in \bar{o}_4 \mid \text{supp } \mathfrak{o} \setminus \text{supp } \bar{h} = o\}, \quad o \subset \bar{\Omega},$$

where the 2-element set  $o$  takes the four values  $\{3, 4\}, \{3, 5\}, \{4, 6\}, \{5, 6\}$ . By the puzzle assembly §1.5 we show that

$$\mathcal{B}_{158}''(\mathbf{c}_{o'} < \mathbf{c}_{o''} \cup \mathbf{c}_{o''}) = \emptyset \quad \text{whenever } o' \cap o'' \neq \emptyset; \quad \text{hence, } \mathcal{B}_{314}''(\bar{o}_4) = \emptyset :$$

```
ds := @data(4, @ (4) [1]);;      update(ds, 314);;
ss := @select(4, @ (ds.dm), ds);; update(ss, 314);;
```

Next, we subdivide  $\bar{o}_6$  into two disjoint clusters (see §1.7)  $\mathbf{c}_=, \mathbf{c}_\neq$ , according to whether the discriminant classes at the two points of  $\text{supp } \bar{h} = \{1, 2\}$  are or are not equal. (The pair of classes can take values  $(4, 4), (1, 1)$  in  $\mathbf{c}_=$  or  $(4, 1), (1, 4)$  in  $\mathbf{c}_\neq$ .) By the puzzle assembly §1.5 we show that

$$\mathcal{B}_{130}''(\mathbf{c}_= < \bar{o}_6) = \emptyset :$$

```
ds := @data(6, @ (6) [1]);;      update(ds, 130);;    # a pipe is used
```

Thus,

$$\bar{b}(\mathfrak{D}) \leq 32_1 + 12_2 + 148_3 + 312_4 + 64_5 + 128_6 + 8_7 = 704.$$

4.3.4. *Vector 4.*

```

1 := rec(fixed := 1, min := 14, chain := 2),
2 := rec(),
3 := rec(),
4 := rec(fixed := 3, min := 16),
5 := rec(fixed := 3, min := 18),
6 := rec(),
8 := rec(),
10 := rec(fixed := 3, min := 28),
12 := rec(fixed := 3, min := 14),      # min := 10
14 := rec(fixed := 3, min := 22),      # min := 16
16 := rec(fixed := -1, min := 16),     # min := 12
18 := rec(),
20 := rec(),
22 := rec(fixed := 3, min := 13),

```

By the puzzle assembly §1.5 we establish that

$$\mathcal{B}_{96}''(\bar{o}_{12}^+) = \mathcal{B}_{138}''(\bar{o}_{14}^+) = \mathcal{B}_{104}''(\bar{o}_{16}^+) = \mathcal{B}_{96}(\bar{o}_8^+, \bar{o}_6^+, \bar{o}_{18}^+, \bar{o}_{20}^+, \bar{o}_3) = \emptyset :$$

```

ds := @data(12);;          update(ds, 96);;
ds := @data(14);;          update(ds, 138);;
ds := @data(16);;          update(ds, 104);;
ch := @chain(8, 6, 18, 20, 3);; update(ch, 96);

```

Hence,

$$\bar{b}(\mathfrak{O}) \leq 56_1 + 28_2 + 94_{3,6,8,18,20} + 64_4 + 36_5 + 56_{10} + 94_{12} + 136_{14} + 102_{16} + 52_{22} = 718.$$

4.4. **The lattice  $N(8\mathbf{A}_3)$ .** There are 4 classes;  $b(\mathfrak{D}) \leq 1024$ .

|           |                   |                   |                   |         |         |                   |                   |         |      |      |               |                           |
|-----------|-------------------|-------------------|-------------------|---------|---------|-------------------|-------------------|---------|------|------|---------------|---------------------------|
| <b>1:</b> | $[4]_{\bullet}$   | $[0]_0$           | $[0]_0$           | $[0]_0$ | $[0]_0$ | $[0]_0$           | $[0]_0$           |         | 5432 | 1484 | $\rightarrow$ | <b>952</b>                |
| 1:        | $[2]_0$           | $[0]_0$           | $[0]_0$           | $[0]_0$ | $[0]_0$ | $[0]_0$           | $[0]_0$           |         | 7**  | 48   | 12            | $\rightarrow$ <u>10</u> ✓ |
| 2:        | $[2]_2$           | $[0]_2$           | $[0]_2$           | $[0]_0$ | $[0]_0$ | $[0]_0$           | $[0]_2$           |         | 7**  | 216  | 72            | $\rightarrow$ <u>38</u> ✓ |
| 3:        | $[2]_2$           | $[0]_3$           | $[0]_3$           | $[0]_0$ | $[0]_3$ | $[0]_0$           | $[0]_0$           | $[0]_1$ | 14*  | 256  | 64            | $\rightarrow$ <u>44</u> ✓ |
| <b>2:</b> | $[2]_0$           | $[2]_0$           | $[0]_0$           | $[0]_0$ | $[0]_0$ | $[0]_0$           | $[0]_0$           |         | 4952 | 1280 | $\rightarrow$ | <b>948</b>                |
| 1:        | $[2]_0$           | $[0]_0$           | $[0]_0$           | $[0]_0$ | $[0]_0$ | $[0]_0$           | $[0]_0$           |         | 12*  | 12   | <u>3</u>      |                           |
| 2:        | $[1]_0^+$         | $[1]_0^+$         | $[0]_0$           | $[0]_0$ | $[0]_0$ | $[0]_0$           | $[0]_0$           |         | 4*   | 4    | <u>2</u>      |                           |
| 3:        | $[1]_2$           | $[1]_2$           | $[0]_2$           | $[0]_0$ | $[0]_0$ | $[0]_0$           | $[0]_2$           |         | 3**  | 144  | 48            | $\rightarrow$ <u>28</u> ✓ |
| 4:        | $[1]_2$           | $[1]_3$           | $[0]_3$           | $[0]_0$ | $[0]_3$ | $[0]_0$           | $[0]_0$           | $[0]_1$ | 16*  | 128  | 32            | $\rightarrow$ <u>24</u> ✓ |
| 5:        | $[1]_3$           | $[1]_3$           | $[0]_2$           | $[0]_3$ | $[0]_1$ | $[0]_0$           | $[0]_0$           |         | 24*  | 96   | 24            | $\rightarrow$ <u>18</u> ✓ |
| 6:        | $[2]_{\bullet}$   | $[0]_0$           | $[0]_0$           | $[0]_0$ | $[0]_0$ | $[0]_0$           | $[0]_0$           |         | 2    | 2    | <u>1</u>      |                           |
| <b>3:</b> | $[1]_2$           | $[1]_2$           | $[1]_2$           | $[0]_0$ | $[0]_0$ | $[0]_0$           | $[1]_2$           | $[0]_0$ | 4472 | 1272 | $\rightarrow$ | <b>1024</b>               |
| 1:        | $[1]_2$           | $[1]_2$           | $[0]_0$           | $[0]_2$ | $[0]_2$ | $[0]_0$           | $[0]_0$           |         | 12*  | 36   | 12            | $\rightarrow$ <u>8</u> ✓  |
| 2:        | $[1]_2$           | $[\frac{1}{2}]_3$ | $[\frac{1}{2}]_3$ | $[0]_0$ | $[0]_3$ | $[0]_0$           | $[0]_0$           | $[0]_1$ | 48*  | 64   | 16            | $\rightarrow$ <u>14</u> ✓ |
| 3:        | $[\frac{1}{2}]_3$ | $[\frac{1}{2}]_3$ | $[\frac{1}{2}]_3$ | $[0]_0$ | $[0]_0$ | $[0]_2$           | $[\frac{1}{2}]_1$ | $[0]_0$ | 8**  | 96   | 32            | $\rightarrow$ <u>22</u> ✓ |
| 4:        | $[2]_{\bullet}$   | $[0]_0$           | $[0]_0$           | $[0]_0$ | $[0]_0$ | $[0]_0$           | $[0]_0$           |         | 4    | 1    | <u>1</u>      |                           |
| 6:        | $[1]_0$           | $[1]_0$           | $[0]_0$           | $[0]_0$ | $[0]_0$ | $[0]_0$           | $[0]_0$           |         | 6    | 16   | 8             | $\rightarrow$ <u>6</u> ✓  |
| <b>4:</b> | $[\frac{3}{4}]_3$ | $[\frac{3}{4}]_3$ | $[\frac{3}{4}]_3$ | $[0]_0$ | $[0]_0$ | $[1]_2$           | $[\frac{3}{4}]_1$ | $[0]_0$ | 4472 | 1204 | $\rightarrow$ | <b>996</b>                |
| 1:        | $[\frac{1}{2}]_2$ | $[\frac{3}{4}]_3$ | $[\frac{1}{4}]_1$ | $[0]_1$ | $[0]_0$ | $[\frac{1}{2}]_1$ | $[0]_0$           |         | 24*  | 72   | 18            | $\rightarrow$ <u>16</u> ✓ |
| 2:        | $[\frac{3}{4}]_3$ | $[\frac{3}{4}]_3$ | $[0]_0$           | $[0]_2$ | $[0]_0$ | $[\frac{1}{2}]_3$ | $[0]_0$           | $[0]_1$ | 12*  | 48   | 12            | $\rightarrow$ <u>10</u> ✓ |
| 3:        | $[1]_0$           | $[1]_0$           | $[0]_0$           | $[0]_0$ | $[0]_0$ | $[0]_0$           | $[0]_0$           |         | 6    | 9    | <u>3</u>      |                           |
| 5:        | $[1]_0$           | $[0]_0$           | $[0]_0$           | $[0]_0$ | $[0]_0$ | $[1]_0$           | $[0]_0$           |         | 4    | 12   | <u>4</u>      |                           |
| 7:        | $[\frac{1}{2}]_2$ | $[\frac{1}{2}]_2$ | $[\frac{1}{2}]_2$ | $[0]_0$ | $[0]_0$ | $[0]_0$           | $[\frac{1}{2}]_2$ | $[0]_0$ | 1    | 81   | 27            | $\rightarrow$ <u>19</u> ✓ |
| 9:        | $[\frac{1}{2}]_2$ | $[\frac{1}{2}]_2$ | $[0]_0$           | $[0]_0$ | $[0]_0$ | $[1]_2$           | $[0]_0$           | $[0]_2$ | 6    | 54   | 18            | $\rightarrow$ <u>12</u> ✓ |
| 11:       | $[\frac{1}{2}]_2$ | $[\frac{3}{4}]_3$ | $[\frac{3}{4}]_3$ | $[0]_0$ | $[0]_3$ | $[0]_0$           | $[0]_0$           | $[0]_1$ | 12   | 48   | 12            | $\rightarrow$ <u>10</u> ✓ |
| 13:       | $[\frac{3}{4}]_3$ | $[\frac{3}{4}]_3$ | $[\frac{3}{4}]_3$ | $[0]_0$ | $[0]_0$ | $[-1]_2$          | $[\frac{3}{4}]_1$ | $[0]_0$ | 1    | 1    | <u>1</u>      |                           |

4.4.1. *Vector 1.*

```

1 := rec(),
2 := rec(fixed := -2, min := 38),          # min := 6
3 := rec(fixed := 2, min := 44, chain := 2), # min := 28

```

We use a non-standard, “non-cluster” approach, splitting  $\mathfrak{O}$  into seven pairwise disjoint triples of the form

$$(\mathfrak{o}_3^+, \mathfrak{o}_1, \mathfrak{o}_2), \quad \mathfrak{o}_i \in \bar{\mathfrak{o}}_i, \quad \text{supp } \mathfrak{o}_3 \cap \text{supp } \mathfrak{o}_2 = \text{supp } \mathfrak{o}_1 \cap \text{supp } \mathfrak{o}_2 = \text{supp } \bar{h}.$$

(Here,  $\mathfrak{o}_2$  and  $\mathfrak{o}_3^+$  determine each other uniquely, whereas for  $\mathfrak{o}_1$  choices can be made.) By the puzzle assembly §1.5 we show that, for each such triple,

$$\mathcal{B}'''_{104}(\mathfrak{o}_3^+, \mathfrak{o}_1, \mathfrak{o}_2) = \emptyset; \quad \text{hence, } \bar{b}(\mathfrak{O}) \leq 7 \cdot 102 = 714 :$$

```

ds := @data(3, @()[1]);          update(ds, 56);;
ss := @select(1, @(ds.dm), ds);; update(ss, 104);; # a pipe is used
                                @extend(ss);

```

There is a unique geometric set  $\mathfrak{L} \subset \mathfrak{O}$  of size  $|\mathfrak{L}| = 728$ . In the notation of \*\*§3.3, assuming that  $h|_1 = \mathbf{1}_\mathcal{I}$  and letting  $r := \{1, 2\}$ ,  $s := \{1, 3\}$ , the lattice  $\text{orth}_h \mathfrak{C}$  (see \*\*Convention 5.2) is generated by any three roots generating  $D_1$  and two extra vectors  $u, v$ :

$$u|_1 = v|_1 = v|_k = [r], \quad u|_k = [s] \quad \text{for } k = 2, \dots, 8.$$

4.4.2. *Vector 2.*

```

1 := rec(),
2 := rec(),
3 := rec(fixed := 1, min := 28),      # min := 18
4 := rec(fixed := 1, min := 24),      # min := 19
5 := rec(fixed := 4, min := 18),      # min := 14
6 := rec(),

```

By the puzzle assembly §1.5 we have

$$\mathcal{B}''_{70}(\bar{\mathfrak{o}}_3) = \mathcal{B}''_{36}(\bar{\mathfrak{o}}_1, \bar{\mathfrak{o}}_2, \bar{\mathfrak{o}}_6^+) = \emptyset :$$

```

ds := @data(3);          update(ds, 70);; # push := 4;
ch := @chain(1, 2, 6);;  update(ch, 36);;

```

There are 24 self-dual four-element sets  $\mathfrak{c}_i \subset \bar{\mathfrak{o}}_5$  such that  $\text{rk } \mathfrak{c}_i = 15$ . They constitute two  $O_{\bar{h}}(N)$ -orbits, both of length 12, and only one of them has disjoint pairs  $(\mathfrak{c}_i, \mathfrak{c}_j)$  such that  $\text{rk}(\mathfrak{c}_i \cup \mathfrak{c}_j) = 18$ . The elements  $\mathfrak{c}_i$  of this latter orbit are taken for clusters, and the 24 pairs  $\mathfrak{p}_k := \mathfrak{c}_i \cup \mathfrak{c}_j$  as above, for larger clusters, see §1.7. Setting  $\text{push} := 3$ , see §1.6, we use the puzzle assembly §1.5 to show that

$$\mathcal{B}''_{318}(\mathfrak{c}_i < \mathfrak{p}_k < \bar{\mathfrak{o}}_5) = \emptyset :$$

```

ds := @data(5, @ (5)[1]);          update(ds, 318);;
ss := @select(5, @(ds.dm), ds);;   update(ss, 318);; # a pipe is used

```

Likewise, there are twelve self-dual four-element sets  $\mathfrak{c}'_i \subset \bar{\mathfrak{o}}_4$  such that  $\text{rk } \mathfrak{c}'_i = 17$ , and they form six disjoint pairs  $\mathfrak{p}'_k := \mathfrak{c}'_i \cup \mathfrak{c}'_j$  such that  $\text{rk } \mathfrak{p}'_k = 20$ . By the puzzle assembly §1.5 with  $\text{push} := 4$  (see §1.6), we find

$$\mathcal{B}''_{152}(\mathfrak{c}'_i < \mathfrak{p}'_k) = \emptyset; \quad \text{hence, } \mathcal{B}''_{302}(\bar{\mathfrak{o}}_4) = \emptyset :$$

```

ds := @data(4, @ (4)[1]);          update(ds, 302);;
ss := @select(4, @(ds.dm), ds);;   update(ss, 302);;

```

Hence,

$$\bar{b}(\mathfrak{O}) \leq 34_{1,2,6} + 68_3 + 300_4 + 316_5 = 718.$$

**Remark 4.2.** Strictly speaking, the flags  $\mathfrak{c}_i \subset \mathfrak{p}_k$  are not homogeneous (see \*\*§4.1), but the group  $O_{\bar{h}}(N)$  acts transitively on the set of such flags; hence, we can still use the arguments of §1.7.

4.4.3. *Vector 3.*

```

1 := rec(),
2 := rec(fixed := 2, min := 14),    # min := 6
3 := rec(),
4 := rec(),
6 := rec(),

```

Consider the six pairwise disjoint clusters (see §1.7)

$$\mathbf{c}_o := \{\mathbf{o} \subset \bar{\mathbf{o}}_2 \mid \text{supp } \mathbf{o} \cap o = \emptyset\}, \quad o \subset \bar{\Omega}, \quad |o| = 2,$$

each consisting of eight combinatorial orbits. They split into three pairs  $(\mathbf{c}_o, \mathbf{c}_{\bar{o}})$ ,  $\bar{o} := \bar{\Omega} \setminus o$ . By the puzzle assembly §1.5 we find that

$$\mathcal{B}_{158}''(\mathbf{c}_o < \mathbf{c}_o \cup \mathbf{c}_{\bar{o}}) = \emptyset; \quad \text{hence,} \quad \mathcal{B}_{470}''(\bar{\mathbf{o}}_2) = \emptyset :$$

```
ds := @data(2, @(2)[1]);;      update(ds, 470);;    # a pipe is used

```

Next, by the puzzle assembly §1.5 we show that

$$\mathcal{B}_{126}''(\bar{\mathbf{o}}_1, \bar{\mathbf{o}}_6^+) = \emptyset :$$

```
ch := @chain(1, 6);;          update(ch, 126);;

```

This implies the bound

$$(4.3) \quad \bar{b}(\mathfrak{D}) \leq 124_{1,6} + 468_2 + 176_3 + 8_4 = 776.$$

To reduce this down to 718, we use the puzzle assembly §1.5 to show that

$$\mathcal{B}_{120,172}'''(\bar{\mathbf{o}}_3; \bar{\mathbf{o}}_1) = \emptyset :$$

```
ds := @data(3);;              update(ds, 120);;
ds := @data(1, ds);;          update(ds, 172);;    @extend(ds);

```

Hence, 176<sub>3</sub> in (4.3) can be reduced down to 118<sub>3</sub>, as  $|\mathfrak{L} \cap \bar{\mathbf{o}}_3| \geq 120$  would imply that

$$|\mathfrak{L}| \leq 170_{1,3} + 468_2 + 8_4 + 72_6 = 718.$$



4.4.4. *Vector 4.*

```

1 := rec(fixed := 1, min := 16),    # min := 10
2 := rec(),
3 := rec(),
5 := rec(),
7 := rec(fixed := 1, min := 19),    # min := 14
9 := rec(),
11 := rec(),
13 := rec(),

```

We apply the following uniform approach to the orbits  $\bar{o}_n$ ,  $n = 1, 9, 11$ . Subdivide  $\bar{o}_n$  into three pairwise disjoint clusters (see §1.7)

$$\mathbf{c}_p := \{\mathbf{o} \subset \bar{o}_n \mid \text{supp } \mathbf{o} \ni p \text{ (if } n = 1, 9) \text{ or } \text{supp } \mathbf{o} \not\ni p \text{ (if } n = 11)\}, \quad p \in \bar{\Omega} = \{4, 5, 8\}.$$

Then, for  $(i, j, k) = (4, 5, 8)$  or  $(4, 8, 5)$  and a certain even integer  $m$ , we iterate the puzzle assembly §1.5 to find that

$$\mathcal{B}'''_{3m+2}(\mathbf{c}_i^+ < \mathbf{c}_i^+ \cup \mathbf{c}_j^+ < \mathbf{c}_i^+ \cup \mathbf{c}_j^+ \cup \mathbf{c}_k^+) = \emptyset,$$

implying that  $\bar{b}(\bar{o}_n^+) \leq 3m$ . In this manner, we show that

$$(4.4) \quad (a) \bar{b}(\bar{o}_1) \leq 264, \quad (b) \bar{b}(\bar{o}_9^+) \leq 96, \quad (c) \bar{b}(\bar{o}_{11}^+) \leq 180 :$$

```

ds := @data(1, @(1)[1]);;      update(ds, 266);;
ss := @select(1, @(ds.dm), ds);; update(ss, 266);; # a pipe is used
ds := @data(9, @(9)[1]);;      update(ds, 98);;
ss := @select(9, @(ds.dm), ds);; update(ss, 98);; # a pipe is used
                                @extend(ss);;
ds := @data(11, @(11)[1]);;    update(ds, 182);;
ss := @select(11, @(ds.dm), ds);; update(ss, 182);; # a pipe is used

```

Next, by the puzzle assembly §1.5 we establish that

$$\mathcal{B}''_{90,186}(\bar{o}_2; \bar{o}_9^+) = \emptyset :$$

```

ds := @data(2);;              update(ds, 90);;
ds := @data(9, ds);;          update(ds, 186);;

```

Finally, iterating the puzzle assembly §1.5, we find that

$$\mathcal{B}''_{90,270}(\bar{o}_3^+, \bar{o}_5^+, \bar{o}_7^+, \bar{o}_{11}^+) = \emptyset :$$

```

ch := @chain(3, 5, 7);;       update(ch, 90);;
ds := @data(11, ch);;         update(ds, 270);;

```

Combining this with (4.4c), cf. (1.7), we arrive at

$$\bar{b}(\mathfrak{D}) \leq 264_1 + 184_{2,9} + 268_{3,5,7,11} + 2_{13} = 718.$$

5. THE LATTICE  $N(12\mathbf{A}_2)$ 

To simplify the tables, we change the notation as follows: we pick a standard Dynkin basis  $a_1, a_2$  for each  $\mathbf{A}_2$ -summand and use the following pictographs:

$$\begin{aligned} (\circ -) &\mapsto a_1, & (-\circ) &\mapsto a_2, & (\circ \circ) &\mapsto a_1 + a_2, \\ (\longrightarrow) &\mapsto \frac{1}{3}(2a_1 + a_2), & (\longleftarrow) &\mapsto \frac{1}{3}(a_1 + 2a_2), \end{aligned}$$

Certainly, in the  $l$ -rows these vectors are merely *representatives* of the combinatorial orbits.

There are 2 classes;  $b(\mathfrak{Q}) \leq 1260$ .

|           |               |               |               |               |               |               |   |               |               |               |   |               |   |   |      |      |               |                           |
|-----------|---------------|---------------|---------------|---------------|---------------|---------------|---|---------------|---------------|---------------|---|---------------|---|---|------|------|---------------|---------------------------|
| <b>1:</b> | $\circ -$     | $\circ -$     | .             | .             | .             | .             | . | .             | .             | .             | . | .             | . | . | 4984 | 1664 | $\rightarrow$ | <b>1184</b>               |
| 1:        | $\circ -$     | .             | $\circ$       | .             | .             | .             | . | .             | .             | .             | . | .             | . | . | 20*  | 6    |               | <u>2</u>                  |
| 2:        | $\circ$       | $\circ$       | .             | .             | .             | .             | . | .             | .             | .             | . | .             | . | . | 4*   | 1    |               | <u>1</u>                  |
| 3:        | $\rightarrow$ | $\rightarrow$ | $\rightarrow$ | $\rightarrow$ | .             | $\rightarrow$ | . | .             | $\rightarrow$ | .             | . | .             | . | . | 60*  | 81   | 27            | $\rightarrow$ <u>19</u> ✓ |
| <b>2:</b> | $\rightarrow$ | $\rightarrow$ | $\rightarrow$ | $\rightarrow$ | .             | $\rightarrow$ | . | .             | $\rightarrow$ | .             | . | .             | . | . | 4504 | 1532 | $\rightarrow$ | <b>1260</b>               |
| 1:        | $\rightarrow$ | $\rightarrow$ | $\rightarrow$ | .             | $\rightarrow$ | .             | . | $\rightarrow$ | .             | .             | . | $\rightarrow$ | . | . | 40*  | 27   | 9             | $\rightarrow$ <u>7</u> ✓  |
| 2:        | $\rightarrow$ | $\rightarrow$ | $\leftarrow$  | $\leftarrow$  | .             | .             | . | .             | .             | $\rightarrow$ | . | $\leftarrow$  | . | . | 90*  | 36   | 12            | $\rightarrow$ <u>10</u> ✓ |
| 3:        | $\leftarrow$  | $\leftarrow$  | $\leftarrow$  | $\leftarrow$  | .             | $\leftarrow$  | . | .             | $\leftarrow$  | .             | . | .             | . | . | 1**  | 64   | 32            | $\rightarrow$ <u>20</u> ✓ |
| 4:        | $\circ$       | $\circ$       | .             | .             | .             | .             | . | .             | .             | .             | . | .             | . | . | 15   | 4    |               | <u>2</u>                  |

## 5.1. Vector 1.

```

1 := rec(),
2 := rec(),
3 := rec(fixed := 3, min := 19),      # min := 10

```

By the puzzle assembly §1.5 we establish that

$$\mathcal{B}_{34}''(\bar{\mathfrak{o}}_1, \bar{\mathfrak{o}}_2) = \emptyset :$$

```

ch := @chain(1, 2);;      update(ch, 34);;

```

Next, we consider the 30 clusters (see §1.7)

$$\mathfrak{c}_{\mathfrak{s}} := \{\mathfrak{o} \in \bar{\mathfrak{o}}_3 \mid \text{supp } \mathfrak{o} \cap \text{supp } \mathfrak{s} = \text{supp } \mathfrak{h}\}, \quad \mathfrak{s} \in \bar{\mathfrak{o}}_3;$$

we have  $|\mathfrak{c}_{\mathfrak{s}}| = 6$  and each orbit  $\mathfrak{o} \subset \bar{\mathfrak{o}}_3$  is contained in three clusters. Hence, each cluster is contained in six *hooks*  $\mathfrak{h}$  and three *tridents*  $\mathfrak{t}_{\mathfrak{o}}$ :

$$\mathfrak{h} := \mathfrak{c}_{\mathfrak{s}'} \cup \mathfrak{c}_{\mathfrak{s}''}, \quad |\mathfrak{c}_{\mathfrak{s}'} \cap \mathfrak{c}_{\mathfrak{s}''}| = 2; \quad \mathfrak{t}_{\mathfrak{o}} := \bigcup_{\mathfrak{c}_{\mathfrak{s}} \ni \mathfrak{o}} \mathfrak{c}_{\mathfrak{s}}, \quad \mathfrak{o} \in \bar{\mathfrak{o}}_3;$$

we have  $|\mathfrak{h}| = 10$  and  $|\mathfrak{t}_{\mathfrak{o}}| = 14$ . Using the flags  $(\mathfrak{c}_{\mathfrak{s}} \setminus \mathfrak{o}^+) < (\mathfrak{h} \setminus \mathfrak{o}^+) < (\mathfrak{t}_{\mathfrak{o}} \setminus \mathfrak{o}^+)$  and puzzle assembly §1.5, we establish that

$$\mathcal{B}_{162}^{\text{iv}}(\mathfrak{t}_{\mathfrak{o}}) = \emptyset, \quad \text{hence} \quad \mathcal{B}_{686}^{\text{iv}}(\bar{\mathfrak{o}}_3) = \emptyset :$$

```

ds := @data(3, @ (3) [1]);;      update(ds, 162);;
ss := @select(3, @ (ds.dm), ds);; update(ss, 162);;  # a pipe is used
                                @extend(ss, 2);;

```

It follows that

$$\bar{b}(\mathfrak{Q}) \leq 32_{1,2} + 684_3 = 716.$$

To avoid the computation of the full set  $\mathcal{B}_0(\mathfrak{o})$ ,  $\mathfrak{o} \in \bar{\mathfrak{o}}_3$ , we set `push := 3` (or even `push := 4` at the very last step), see §1.6, and essentially reduce the algorithm to brute force §1.4.

We found but three large geometric sets  $\mathfrak{C}$ , of sizes 608, 608, 600, which are graph isomorphic to some of those listed in §6.1 below.

**Remark 5.1.** The chain  $\mathbf{c}_s \subset \mathbf{h} \subset \mathbf{t}_o$  is not homogeneous in the sense of [\\*\\*§4.1](#), and we need to modify the approach of [§1.7](#). We can assume that  $\mathbf{h}$  is the largest hook in  $\mathbf{t}_o$  and  $\mathbf{c}_s$  is the largest cluster in  $\mathbf{h}$  (hence, also in  $\mathbf{t}_o$ ). Then, for the “central” pair  $\mathbf{o}^+$  in  $\mathbf{h}$  and  $\mathbf{t}_o$ , we have

$$\begin{aligned} |\mathfrak{C} \cap \mathbf{h}| &\geq \frac{2}{3}|\mathfrak{C} \cap \mathbf{t}_o| + \frac{1}{3}|\mathfrak{C} \cap \mathbf{o}^+| \geq 108, \\ |\mathfrak{C} \cap \mathbf{c}_s| &\geq \frac{1}{3}|\mathfrak{C} \cap \mathbf{t}_o| + \frac{2}{3}|\mathfrak{C} \cap \mathbf{o}^+| \geq 54, \\ |\mathfrak{C} \cap \mathbf{c}_s| &\geq \frac{1}{2}|\mathfrak{C} \cap \mathbf{h}| + \frac{1}{2}|\mathfrak{C} \cap \mathbf{o}^+| \geq 54. \end{aligned}$$

Thus, we use the conservative estimates on the right aiming at  $\mathcal{B}_{54}(\mathbf{c}_s)$  and  $\mathcal{B}_{108}(\mathfrak{C}; \mathbf{h})$ , but we invoke the more refined estimates in the middle when setting the lower and upper bounds, as in [\(1.14\)](#), in the computation of  $\mathcal{B}_{108}(\mathfrak{C}; \mathbf{h})$  and  $\mathcal{B}_{162}(\mathfrak{C}; \mathbf{t}_o)$ . For example, a set  $\mathfrak{C} \subset \mathbf{c}_s$  would have to be rejected (for a particular hook  $\mathbf{h}$  or trident  $\mathbf{t}_o$ , which both determine the position of  $\mathbf{o}^+ \subset \mathbf{c}_s$ ) unless

$$3|\mathfrak{C}| - 2|\mathfrak{C} \cap \mathbf{o}^+| \geq 162.$$

## 5.2. Vector 2.

```
1 := rec(),
2 := rec(),
3 := rec(),
4 := rec(),
```

For each combinatorial orbit  $\mathbf{o} \in \bar{\mathbf{o}}_1$ , there is a unique *complimentary combinatorial orbit*  $\mathbf{o}' \in \bar{\mathbf{o}}_1$ , characterized by the property that  $\text{supp } \mathbf{o}' = \Omega \setminus \text{supp } \mathbf{o}$ , and we consider the 10 pairwise disjoint clusters (see [§1.7](#))

$$\mathbf{p}_i := \{\mathbf{o}, \mathbf{o}^*, \mathbf{o}', \mathbf{o}'^*\}, \quad i = 1, \dots, 10.$$

The unions  $\mathbf{p}_{ij} := \mathbf{p}_i \cup \mathbf{p}_j$ ,  $i \neq j$ , also constitute a single  $O_{\bar{\mathbf{h}}}(N)$ -orbit, and by the puzzle assembly [§1.5](#) we show that

$$\mathcal{B}_{172;210}^{\text{iv}}(\mathbf{p}_{ij} < \bar{\mathbf{o}}_1; \bar{\mathbf{o}}_4^+, \bar{\mathbf{o}}_3) = \mathcal{B}_{40;210}''(\bar{\mathbf{o}}_3, \bar{\mathbf{o}}_4^+; \mathbf{p}_i < \bar{\mathbf{o}}_1) = \emptyset, \quad \text{cf. (1.7):}$$

```
ds := @data(1, @@(2)[1]);      update(ds, 172);      # a pipe is used
ds := @data(4, ds);            update(ds, 190);
ds := @data(3, ds);            update(ds, 210);      @extend(ds, 2);

ch := @chain(3, 4);            update(ch, 40);
ss := @select(1, @@(1), ch);    update(ss, 210);      # a pipe is used
```

Next, we consider the 15 pairwise disjoint clusters (see [§1.7](#))

$$\mathbf{c}_o := \{\mathbf{o} \in \bar{\mathbf{o}}_2 \mid \text{supp } \mathbf{o} \subset \text{supp } \bar{\mathbf{h}} \cup \mathbf{o}\}, \quad o \subset \bar{\Omega}, \quad |o| = 2,$$

and the 20 triple unions

$$\mathbf{t}_s := \bigcup_{o \subset s} \mathbf{c}_o, \quad s = \text{supp } \mathbf{o} \setminus \text{supp } \bar{\mathbf{h}} \text{ for some } \mathbf{o} \in \bar{\mathbf{o}}_1.$$

By the puzzle assembly [§1.5](#), we have

$$\mathcal{B}_{512}''(\mathbf{c}_o < \mathbf{t}_s < \mathbf{t}_s \cup \mathbf{t}_{\bar{s}} < \bar{\mathbf{o}}_2) = \emptyset$$

for each pair  $o \subset s$  as above and  $\bar{s} := \bar{\Omega} \setminus s$ :

```
ds := @data(2, @(2)[1]);      update(ds, 512);
ss := @select(2, @(ds.dm), ds); update(ss, 512);      # a pipe is used
```

It follows that  $\bar{b}(\bar{\mathbf{o}}_2) \leq 510$  and

$$\bar{b}(\mathfrak{D}) \leq 208_{1,3,4} + 510_2 = 718.$$

We found but three large geometric sets  $\mathfrak{C}$ , of sizes 660, 640, 640, which are graph isomorphic to some of those listed in [§6.1](#) below.



|                         |  |                                              |
|-------------------------|--|----------------------------------------------|
| $ \mathfrak{C}  = 800:$ |  | $[4, 0, 40] (1, 0)$                          |
| $ \mathfrak{C}  = 736:$ |  | $[12, 0, 16] (1, 0)$                         |
| $ \mathfrak{C}  = 728:$ |  | $[14, 0, 14] (1, 0)$                         |
| $ \mathfrak{C}  = 704:$ |  | $[8, 4, 28] (0, 1)$                          |
| $ \mathfrak{C}  = 704:$ |  | $[8, 4, 28] (0, 1)$                          |
| $ \mathfrak{C}  = 680:$ |  | $[12, 4, 20] (0, 1)$                         |
| $ \mathfrak{C}  = 680:$ |  | $[12, 4, 20] (0, 1)$                         |
| $ \mathfrak{C}  = 680:$ |  | $[4, 2, 56] (1, 0)$<br>$[16, 6, 16] (1, 0)$  |
| $ \mathfrak{C}  = 664:$ |  | $[4, 0, 60] (1, 0)$                          |
| $ \mathfrak{C}  = 664:$ |  | $[4, 0, 60] (1, 0)$                          |
| $ \mathfrak{C}  = 660:$ |  | $[4, 0, 60] (1, 0)$                          |
| $ \mathfrak{C}  = 656:$ |  | $[2, 0, 122] (1, 0)$<br>$[10, 4, 26] (0, 1)$ |
| $ \mathfrak{C}  = 656:$ |  | $[2, 0, 122] (1, 0)$<br>$[10, 4, 26] (0, 1)$ |
| $ \mathfrak{C}  = 656:$ |  | $[2, 0, 122] (1, 0)$<br>$[10, 4, 26] (0, 1)$ |

|                         |  |                                             |
|-------------------------|--|---------------------------------------------|
| $ \mathfrak{C}  = 640:$ |  | $[4, 0, 72] (1, 0)$                         |
| $ \mathfrak{C}  = 640:$ |  | $[4, 0, 72] (1, 0)$                         |
| $ \mathfrak{C}  = 640:$ |  | $[4, 0, 72] (1, 0)$                         |
| $ \mathfrak{C}  = 640:$ |  | $[4, 0, 72] (1, 0)$                         |
| $ \mathfrak{C}  = 628:$ |  | $[4, 0, 66] (1, 0)$<br>$[12, 0, 22] (1, 0)$ |
| $ \mathfrak{C}  = 624:$ |  | $[12, 4, 24] (0, 2)$                        |
| $ \mathfrak{C}  = 624:$ |  | $[10, 2, 28] (0, 1)$                        |
| $ \mathfrak{C}  = 624:$ |  | $[10, 2, 28] (0, 1)$                        |
| $ \mathfrak{C}  = 622:$ |  | $[10, 2, 28] (0, 1)$                        |
| $ \mathfrak{C}  = 622:$ |  | $[10, 2, 28] (0, 1)$                        |
| $ \mathfrak{C}  = 622:$ |  | $[10, 2, 28] (0, 1)$                        |
| $ \mathfrak{C}  = 620:$ |  | $[14, 0, 20] (1, 0)$                        |
| $ \mathfrak{C}  = 620:$ |  | $[14, 0, 20] (1, 0)$                        |
| $ \mathfrak{C}  = 620:$ |  | $[12, 4, 24] (0, 2)$                        |

|                        |  |                                              |
|------------------------|--|----------------------------------------------|
| $ \mathcal{C}  = 616:$ |  | $[4, 0, 72] (2, 0)$                          |
| $ \mathcal{C}  = 616:$ |  | $[4, 0, 72] (2, 0)$                          |
| $ \mathcal{C}  = 616:$ |  | $[4, 0, 72] (2, 0)$                          |
| $ \mathcal{C}  = 616:$ |  | $[2, 0, 138] (1, 0)$<br>$[12, 6, 26] (1, 0)$ |
| $ \mathcal{C}  = 608:$ |  | $\text{rk} = 19 (1, 0)$                      |
| $ \mathcal{C}  = 608:$ |  | $[8, 0, 36] (1, 0)$                          |
| $ \mathcal{C}  = 608:$ |  | $[14, 4, 22] (0, 1)$                         |
| $ \mathcal{C}  = 608:$ |  | $[14, 4, 22] (0, 1)$                         |
| $ \mathcal{C}  = 608:$ |  | $[14, 4, 22] (0, 1)$                         |
| $ \mathcal{C}  = 608:$ |  | $[4, 0, 76] (1, 0)$<br>$[16, 4, 20] (0, 1)$  |
| $ \mathcal{C}  = 608:$ |  |                                              |

```
1  := rec(),
2  := rec(),
```

$$\mathbf{c}_o := \{\mathbf{o} \in \bar{\mathbf{o}}_1 \mid \text{supp } \mathbf{o} \subset o\}, \quad o \in \mathcal{C}_8 \text{ (an octad), } o \cap \text{supp } \mathbf{h} = \emptyset,$$
$$\mathcal{B}_{702}''(\mathbf{c}_o < \mathbf{c}_o \cup \mathbf{c}_{\bar{o}} < \bar{\mathbf{o}}_1) = \emptyset :$$

Likewise, we show that

$$\mathcal{B}''_{18:720}(\bar{\mathbf{o}}_2^+; \mathbf{c}_o < \mathbf{c}_o \cup \mathbf{c}_{\bar{o}} < \bar{\mathbf{o}}_1) = \emptyset :$$

```
ds := @data(2);           update(ds, 18);
ss := @select(1, @(1), ds); update(ss, 720); # a pipe is used
```

$$\bar{b}(\mathfrak{D}) \leq 700_1 + 16_2 = 716.$$

The complete list of the sets  $\mathfrak{C}$  of size  $|\mathfrak{C}| \geq 600$  that have been observed is as follows (in the same notation as in §6.1):

|                         |  |                                                          |
|-------------------------|--|----------------------------------------------------------|
| $ \mathfrak{C}  = 704:$ |  | $[8, 4, 28] \quad (0, 1)$                                |
| $ \mathfrak{C}  = 704:$ |  | $[8, 4, 28] \quad (0, 1)$                                |
| $ \mathfrak{C}  = 680:$ |  | $[12, 4, 20] \quad (0, 1)$                               |
| $ \mathfrak{C}  = 680:$ |  | $[12, 4, 20] \quad (0, 1)$                               |
| $ \mathfrak{C}  = 664:$ |  | $[4, 0, 60] \quad (1, 0)$                                |
| $ \mathfrak{C}  = 656:$ |  | $[2, 0, 122] \quad (1, 0)$<br>$[10, 4, 26] \quad (0, 1)$ |
| $ \mathfrak{C}  = 656:$ |  | $[2, 0, 122] \quad (1, 0)$<br>$[10, 4, 26] \quad (0, 1)$ |
| $ \mathfrak{C}  = 656:$ |  | $[2, 0, 122] \quad (1, 0)$<br>$[10, 4, 26] \quad (0, 1)$ |



|                         |  |                                              |
|-------------------------|--|----------------------------------------------|
| $ \mathfrak{C}  = 656:$ |  | $[2, 0, 122] (1, 0)$<br>$[10, 4, 26] (0, 1)$ |
| $ \mathfrak{C}  = 656:$ |  |                                              |
| $ \mathfrak{C}  = 624:$ |  | $[12, 4, 24] (0, 2)$                         |
| $ \mathfrak{C}  = 624:$ |  | $[12, 4, 24] (0, 2)$                         |
| $ \mathfrak{C}  = 624:$ |  | $[12, 4, 24] (0, 2)$                         |
| $ \mathfrak{C}  = 624:$ |  | $[10, 2, 28] (0, 1)$                         |
| $ \mathfrak{C}  = 624:$ |  |                                              |
| $ \mathfrak{C}  = 620:$ |  | $[12, 4, 24] (0, 2)$                         |
| $ \mathfrak{C}  = 620:$ |  | $[12, 4, 24] (0, 2)$                         |
| $ \mathfrak{C}  = 620:$ |  | $[12, 4, 24] (0, 2)$                         |
| $ \mathfrak{C}  = 620:$ |  | $[12, 4, 24] (0, 2)$                         |
| $ \mathfrak{C}  = 616:$ |  | $[4, 0, 72] (2, 0)$                          |
| $ \mathfrak{C}  = 616:$ |  | $[4, 0, 72] (2, 0)$                          |
| $ \mathfrak{C}  = 616:$ |  | $[2, 0, 138] (1, 0)$<br>$[12, 6, 26] (1, 0)$ |

|                         |  |                                                          |
|-------------------------|--|----------------------------------------------------------|
| $ \mathfrak{C}  = 616:$ |  | $[2, 0, 138] \quad (1, 0)$<br>$[12, 6, 26] \quad (1, 0)$ |
| $ \mathfrak{C}  = 616:$ |  | $[2, 0, 138] \quad (1, 0)$<br>$[12, 6, 26] \quad (1, 0)$ |
| $ \mathfrak{C}  = 616:$ |  | $[2, 0, 138] \quad (1, 0)$<br>$[12, 6, 26] \quad (1, 0)$ |
| $ \mathfrak{C}  = 608:$ |  | $[14, 4, 22] \quad (0, 1)$                               |
| $ \mathfrak{C}  = 608:$ |  | $[14, 4, 22] \quad (0, 1)$                               |
| $ \mathfrak{C}  = 608:$ |  | $[8, 0, 36] \quad (1, 0)$                                |
| $ \mathfrak{C}  = 608:$ |  | $[4, 0, 76] \quad (1, 0)$<br>$[16, 4, 20] \quad (0, 1)$  |
| $ \mathfrak{C}  = 608:$ |  | $[4, 0, 76] \quad (1, 0)$<br>$[16, 4, 20] \quad (0, 1)$  |
| $ \mathfrak{C}  = 600:$ |  | $[4, 0, 72] \quad (2, 0)$                                |
| $ \mathfrak{C}  = 600:$ |  | $[4, 0, 72] \quad (2, 0)$                                |
| $ \mathfrak{C}  = 600:$ |  | $[12, 0, 24] \quad (1, 0)$                               |
| $ \mathfrak{C}  = 600:$ |  | $[12, 0, 24] \quad (1, 0)$                               |
| $ \mathfrak{C}  = 600:$ |  | $[12, 0, 24] \quad (1, 0)$                               |

## 7. THE LEECH LATTICE

The Leech lattice  $\Lambda$  has a unique, up to  $O(\Lambda)$ , 4-polarization  $h \in \Lambda$ . The proof of [\\*\\*Theorem 6.1](#) is based on [\\*\\*Lemma 6.2](#). Namely, we start with  $\mathfrak{D}_h$  and build chains

$$\mathfrak{D}_h =: \mathfrak{C}_0 \supset \mathfrak{C}_1 \supset \dots$$

of self-dual (*a priori* not saturated) subsets recursively: once a set  $\mathfrak{C}_k$  has been constructed, we

- (1) consider the quotient projection (mod 2):  $\text{span}_{\mathbb{Z}} \mathfrak{C}_k \rightarrow V_k := (\text{span}_{\mathbb{Z}} \mathfrak{C}_k) \otimes \mathbb{F}_2$ ;
- (2) compute the  $(\text{stab } \mathfrak{C}_k)$ -orbits on the annihilator  $h^\perp \subset V_k^\vee$  (as all sets are self-dual);
- (3) for a representative  $v$  of each orbit, let  $\mathfrak{C}_{k+1} := \mathfrak{C}_k \cap (\text{mod } 2)^{-1}(v^\perp)$ ;
- (4) discard the subsets  $\mathfrak{C}_{k+1}$  of cardinality

$$|\mathfrak{C}_{k+1}| < 720 + \max\{0, 2(\text{rk } \mathfrak{C}_{k+1} - 20)\}$$

(as at least two conics are lost when the rank is reduced by one unit).

Several tricks described in [§7.1–§7.5](#) below are used to speed up the algorithm.

**Remark 7.1.** In fact, we work with the index 2 sublattice  $\Lambda' \subset \Lambda$  generated by  $\mathfrak{D}$ ; it has a larger orthogonal group:  $[O_h(\Lambda') : O_h(\Lambda)] = 2$ .

**7.1. Follow the proof of [\\*\\*Lemma 6.2](#) literally.** We do not accept a new set  $\mathfrak{C}_{k+1}$  unless

the group  $\text{span } \mathfrak{C}_{k+1} / \text{span}_{\mathbb{Z}} \mathfrak{C}_{k+1}$  is cyclic or free abelian.

More precisely, we keep track of the last

$$(7.2) \quad \text{saturated set } \mathfrak{S} := \mathfrak{C}_r, r \leq k, \quad \text{its lattice } \text{span}_{\mathbb{Z}} \mathfrak{S}, \quad \text{and group } H := \text{stab } \mathfrak{S},$$

and it is the quotient

$$(7.3) \quad Q_{k+1} := \text{span}_{\mathbb{Z}} \mathfrak{S} / \text{span}_{\mathbb{Z}} \mathfrak{C}_{k+1}$$

that we check. If  $Q_k \neq 0$  is a finite cyclic group, generated by (the image of) a vector  $\bar{\kappa} \in \text{span}_{\mathbb{Z}} \mathfrak{S}$ , we keep the vector  $\kappa := |Q_k| \bar{\kappa} \in \text{span}_{\mathbb{Z}} \mathfrak{C}_k$  and, at the next step, reduce  $V_k^\vee$  to the affine space

$$\bar{V}_k^\vee := \{v \in V_k^\vee \mid \langle v, \kappa \rangle \neq 0\}.$$

**7.2. Compute and sort rank by rank, set by set, index by index.** The saturated sets  $\mathfrak{S}$  as in (7.2) play a special rôle: each such set is considered separately and is exhausted index by index (referring to the size  $|Q_{k+1}|$  in (7.3)) until the rank drops. Thus, for each new set  $\mathfrak{C}_{k+1} \subset \mathfrak{S}$ ,

- if  $\text{rk } \mathfrak{C}_{k+1} < \text{rk } \mathfrak{S}$ , then  $\mathfrak{C}_{k+1}$  is carried over to the next rank, see below;
- otherwise,  $\mathfrak{C}_{k+1}$  is stored for a subsequent step within  $\mathfrak{S}$ .

In the latter case, we retain a single representative of each  $H$ -orbit. To compare two sets  $\mathfrak{C}'$ ,  $\mathfrak{C}''$ , we compare their

$$(7.4) \quad \text{ranks } \text{rk } \mathfrak{C}^*, \quad \text{sizes } |\mathfrak{C}^*|, \quad \text{indices } |Q^*|, \quad \text{graph isomorphism classes}$$

(for the latter, the sets are stored according to the canonical labelling given by the `digraph` package, so that it remains to compare their adjacency matrices); if everything coincides, we check if  $\mathfrak{C}'$ ,  $\mathfrak{C}''$  belong to the same orbit *via*

`RepresentativeAction(H, Set( $\mathfrak{C}'$ ), Set( $\mathfrak{C}''$ ), OnSets) <> fail;`

When storing a set  $\mathfrak{C}_{k+1}$  of lower rank  $\text{rk } \mathfrak{C}_{k+1} < \text{rk } \mathfrak{S}$ , we stop at (7.4): indeed, we are primarily interested in subsets  $\mathfrak{C} \subset \mathfrak{D}$  as abstract graphs rather than particular embeddings into  $\Lambda$ . However, if a new set  $\mathfrak{C}'$  has the stabilizer  $\text{stab } \mathfrak{C}'$  (to be used as  $H$  in a subsequent step) larger than that of a set  $\mathfrak{C}''$  already present on the list, then  $\mathfrak{C}'$  replaces  $\mathfrak{C}''$ .

**Remark 7.5.** *A posteriori*, we show (see [§7.6](#) below or [\\*\\*§6.2](#) for more details) that each of the large sets of rank at most 20 found admits a unique, up to  $O_h(\Lambda)$ , embedding to  $\mathfrak{D}$ .

**7.3. Choose a standard basis for  $V_k^\vee$ .** When computing the orbits (and even the spaces  $\bar{V}_k^\vee$ ), a great deal of time is spent to the mere listing of  $V_k^\vee$ , converting it from a vector space to a set on which the group  $G_k := \text{stab } \mathfrak{C}_k$  acts. On the other hand,  $V_k^\vee$  is an  $\mathbb{F}_2$ -vector space of dimension  $19 \leq \dim V_k^\vee \leq 23$ . Therefore, we conjugate the  $G_k$ -action to the standard basis and keep the five “standard” vector spaces pre-listed as sets.

**7.4. Compute representatives rather than orbits.** For small groups (we use  $|G| \leq 2^{13}$ : this may be arbitrary, but it works well), in item (2) above, instead of computing the whole orbits and selecting representatives *via*

```
V := List(OrbitsDomain(G, V), o -> o[1]);
```

we compute a list of representatives directly:

```
G := List(G);
V := Filtered(V, v -> ForAll(G, v <= v*g));
```

**7.5. Count both hits *and* misses.** In items (3), (4) above, for each orbit representative  $v \in V_k^\vee$ , a “natural” way to proceed would be to compute  $\mathfrak{C}_{k+1}$  first, item (3), and then discard it unless  $|\mathfrak{C}_{k+1}|$  is large, item (4):

```
new := Filtered(old, u -> u*o = Z(2)*0);
if Length(new) < min_size then return fail; fi;
return new;
```

where we let  $\text{old} := \mathfrak{C}_k$  and  $\text{new} := \mathfrak{C}_{k+1}$  or  $\text{fail}$ . However, the number of orbits is often huge (it is not uncommon that  $|G_k| = 4$  or even 2), and the following less straightforward code reduces the time dramatically:

```
new := [ ];
c := Length(old) - min_count;      # = 720
for u in old do
  if u*v = Z(2)*0 then
    Add(new, u);
  else
    c := c - 1;
    if c < 0 then return fail; fi;    # too many misses: abort!!
  fi;
od;
return new;
```

In other words, we count the misses as well, not only hits, and we abort prematurely as soon as too many misses have been encountered. This works well because the vast majority of sets  $\mathfrak{C}_k$  to be dealt with are relatively small,  $|\mathfrak{C}_k| < 800$  (the numbers growing quite fast as  $|\mathfrak{C}_k|$  approaches the goal 720), and we can abort after but a few misses. In particular, we avoid the creation of large lists never to be used, followed by garbage collection.

**7.6. The results.** The output of the algorithm is but nine sets  $\mathfrak{C}_k \subset \mathfrak{D}$  of rank  $\text{rk } \mathfrak{C} \leq 20$  and size  $|\mathfrak{C}| \geq 720$ . All sets are saturated and of rank 20, and their sizes are

$$|\mathfrak{C}| = 896, \underline{800}, \underline{768}, \underline{760}, \underline{740}, \underline{736}, \underline{736}, \underline{728}, \underline{720},$$

where underlined are the geometric ones. The sets are described below by means of the Gram matrix of the lattice  $\text{ort}_h \mathfrak{C}$  of **\*\*Convention 5.2**, where the first basis vector is always  $h$ . For the four geometric sets we show also the generators of  $\text{ort}_h \mathfrak{C}$  in the “standard” model  $\Lambda \subset \mathbf{H}_{24}(\frac{1}{8})$ , see **\*\*§6.2**, using the following notation for the coefficients:

$$(\bullet) \mapsto 4, \quad (\circ) \mapsto -4, \quad (+) \mapsto 2, \quad (-) \mapsto -2.$$

For transparency, we assume that  $\{1, \dots, 8\}$  and  $\{5, \dots, 12\}$  are octads of the Golay code, and we cut the display at position 14, extending each vector by zeroes. The four geometric sets  $\mathfrak{C}$  are

$$(7.6) \quad |\mathfrak{C}| = 800: \quad \begin{bmatrix} 4 & 0 & 0 & 0 & 2 \\ 0 & 4 & 0 & 1 & 2 \\ 0 & 0 & 4 & 1 & 2 \\ 0 & 1 & 1 & 4 & 0 \\ 2 & 2 & 2 & 0 & 4 \end{bmatrix} \quad \begin{matrix} \cdot & \cdot & \cdot & \bullet & \cdot & \cdot & \circ & \cdot & \cdot & \cdot & \cdot & \cdot & \cdot & \cdot \\ \cdot & \cdot & \cdot & \cdot & \cdot & \cdot & \bullet & \cdot & \cdot & \cdot & \cdot & \cdot & \cdot & \cdot \\ \cdot & \cdot & \cdot & + & + & - & + & - & + & - & + & + & + & \cdot \\ + & + & + & + & + & + & + & + & + & + & + & \cdot & \cdot & \cdot \\ \cdot & \cdot & \cdot & + & + & - & - & + & + & + & + & + & + & \cdot \end{matrix}$$

$$(7.7) \quad |\mathfrak{C}| = 736: \quad \begin{bmatrix} 4 & 2 & 0 & 0 & 0 \\ 2 & 4 & 0 & 0 & 2 \\ 0 & 0 & 4 & 1 & 2 \\ 0 & 0 & 1 & 4 & 2 \\ 0 & 2 & 2 & 2 & 4 \end{bmatrix} \quad \begin{matrix} \circ & \cdot & \cdot & \cdot & \bullet & \cdot & \cdot & \cdot & \cdot & \cdot & \cdot & \cdot & \cdot & \cdot \\ \cdot & \cdot & \cdot & \cdot & \bullet & \bullet & \cdot & \cdot & \cdot & \cdot & \cdot & \cdot & \cdot & \cdot \\ \cdot & \cdot & \cdot & \cdot & \cdot & \cdot & \cdot & \bullet & \cdot & \bullet & \cdot & \cdot & \cdot & \cdot \\ + & + & + & + & + & + & + & + & + & + & + & \cdot & \cdot & \cdot \\ \cdot & \cdot & \cdot & + & + & + & + & + & + & + & + & + & + & \cdot \end{matrix}$$

$$(7.8) \quad |\mathfrak{C}| = 728: \quad \begin{bmatrix} 4 & 2 & 2 & 2 & 2 \\ 2 & 4 & 0 & 1 & 0 \\ 2 & 0 & 4 & 0 & 1 \\ 2 & 1 & 0 & 4 & 2 \\ 2 & 0 & 1 & 2 & 4 \end{bmatrix} \quad \begin{matrix} \cdot & \cdot & \cdot & \cdot & \bullet & \bullet & \cdot & \cdot & \cdot & \cdot & \cdot & \cdot & \cdot & \cdot \\ + & + & + & + & + & + & + & + & + & + & + & \cdot & \cdot & \cdot \\ + & - & - & - & + & + & - & + & \cdot & \cdot & \cdot & \cdot & \cdot & \cdot \\ \cdot & \cdot & \cdot & + & + & + & - & - & + & + & + & \cdot & \cdot & \cdot \\ \cdot & \cdot & \cdot & + & + & - & - & + & + & + & + & + & + & \cdot \end{matrix}$$

$$(7.9) \quad |\mathfrak{C}| = 720: \quad \begin{bmatrix} 4 & 0 & 0 & 2 & 2 \\ 0 & 4 & 0 & 0 & 2 \\ 0 & 0 & 4 & 0 & 2 \\ 2 & 0 & 0 & 4 & 1 \\ 2 & 2 & 2 & 1 & 4 \end{bmatrix} \quad \begin{matrix} \bullet & \bullet & \cdot & \cdot & \cdot & \cdot & \cdot & \cdot & \cdot & \cdot & \cdot & \cdot & \cdot & \cdot \\ \cdot & \cdot & \bullet & \bullet & \cdot & \cdot & \cdot & \cdot & \cdot & \cdot & \cdot & \cdot & \cdot & \cdot \\ \cdot & \cdot & \cdot & \cdot & \bullet & \bullet & \cdot & \cdot & \cdot & \cdot & \cdot & \cdot & \cdot & \cdot \\ \bullet & \cdot & \cdot & \cdot & \cdot & \cdot & \cdot & \cdot & \bullet & \cdot & \cdot & \cdot & \cdot & \cdot \\ + & + & + & + & + & + & + & + & + & + & + & \cdot & \cdot & \cdot \end{matrix}$$

The other five sets  $\mathfrak{C}$  are as follows (listed in the decreasing order):

$$(7.10) \quad (a) \begin{bmatrix} 4 & 0 & 0 & 2 & 2 \\ 0 & 4 & 0 & 0 & 2 \\ 0 & 0 & 4 & 0 & 2 \\ 2 & 0 & 0 & 4 & 0 \\ 2 & 2 & 2 & 0 & 4 \end{bmatrix}, (b) \begin{bmatrix} 4 & 0 & 0 & 2 & 0 \\ 0 & 4 & 0 & 2 & 2 \\ 0 & 0 & 4 & 0 & 2 \\ 2 & 2 & 0 & 4 & 0 \\ 0 & 2 & 2 & 0 & 4 \end{bmatrix}, (c) \begin{bmatrix} 4 & 2 & 2 & 2 & 2 \\ 2 & 4 & 1 & 0 & 0 \\ 2 & 1 & 4 & 0 & 0 \\ 2 & 0 & 0 & 4 & 1 \\ 2 & 0 & 0 & 1 & 4 \end{bmatrix}, (d) \begin{bmatrix} 4 & 0 & 0 & 0 & 2 \\ 0 & 4 & 0 & 0 & 2 \\ 0 & 0 & 4 & 0 & 1 \\ 0 & 0 & 0 & 4 & 2 \\ 2 & 2 & 1 & 2 & 4 \end{bmatrix}.$$

The non-geometric sets of size 768 and 736 share the same lattice (7.10b), which has two distinct embeddings to  $\Lambda \ni h$ ; for the other seven sets in (7.6)–(7.10), an embedding  $(\text{ort}_h \mathfrak{C} \ni h) \hookrightarrow (\Lambda \ni h)$  is unique up to  $O_h(\Lambda)$ : since only square 4 vectors are involved, this fact can easily be established by brute force.
